# Supplementary material for: Optimal Diagonal Preconditioning
Source: arXiv:2209.00809 source file (2022-11-04)
Supplement: Supplementary file 1 [file appendix_concentration.tex]

\section{Results with Omitted Proofs for Condition Number Concentration}
\label{sec:appendix_concentration}

In this section we provide a sequence of results culminating in Theorem
\ref{thm:concentration_1} of the main paper, which states that the
diagonal preconditioning procedure given by 
\begin{align}
X_{0} & =XD^{-\frac{1}{2}}
\end{align}
where $D$ is the diagonal matrix with 
\begin{align*}
D_{jj} & =\frac{1}{n-1}\sum_{i=1}^{n}(X_{ij}-\mu_{j})^{2}\\
\mu_{j} & =\frac{1}{n}\sum_{i=1}^{n}X_{ij}
\end{align*}
results in a reduction of condition number on the order of $\frac{\kappa(\Sigma)}{\kappa(D^{-\frac{1}{2}}\Sigma D^{-\frac{1}{2}})}$
with high probability. 

Because the scaling matrix $D$ is a function of sample statistics,
namely the column-wise sample standard deviations or column norm,
the analysis with $D$ directly is cumbersome. Our strategy for showing
the main result is to start with the simplest possible case for $D$
and gradually increase the complexity of the scaling matrix. More
precisely, we show a sequence of concentration results, each one built
on top of the other, with the following scaling matrices:
\begin{itemize}
	\item $D$ is equal to the population covariance matrix $\Sigma$, with
	general non-diagonal $\Sigma$.
	\item $D$ is the sample column-wise standard deviation, under the assumption
	that $\Sigma$ is diagonal. 
	\item $D$ is the diagonal of the population covariance matrix, with general
	non-diagonal $\Sigma$.
	\item $D$ is the sample standard deviation, with general non-diagonal $\Sigma$. 
\end{itemize}
We start with the case $D=\Sigma$. Even though $\Sigma$ is not diagonal
in general, we will see that its concentration result on condition
numbers is the easiest to prove, and will also be useful for later
steps. Let
\begin{align*}
X_{0} & =X\Sigma^{-\frac{1}{2}}
\end{align*}

Observe that 
\begin{align*}
\|X^{T}X\|_{op} & \leq\|X_{0}^{T}X_{0}\|_{op}\cdot\|\Sigma\|_{op}\\
\|(X^{T}X)^{-1}\|_{op} & \leq\|(X_{0}^{T}X_{0})^{-1}\|_{op}\cdot\|(\Sigma)^{-1}\|_{op}
\end{align*}
so that
\begin{align*}
\kappa(X^{T}X) & \leq\kappa(X_{0}^{T}X_{0})\cdot\kappa(\Sigma)
\end{align*}
holds true for any positive definite $\Sigma$. We want to show that
when $X$ has independent sub-Gaussian rows with second moment $\Sigma$,
the gap in the inequality is small with high probability, i.e. 
\begin{align*}
\kappa(X^{T}X)\approx & \kappa(X_{0}^{T}X_{0})\cdot\kappa(\Sigma)
\end{align*}
with high probability. The intuition is that tall matrices $X$ are
approximate isometries, so that $X_{0}$ will be close to the identity
matrix with high probability.

Our first result is the closeness of the two quantities $\kappa(X_{0}^{T}X_{0})$
and $\frac{\kappa(X^{T}X)}{\kappa(\Sigma)}$. Intuitively, since $\mathbb{E}X_{0}^{T}X_{0}=\Sigma^{-\frac{1}{2}}\mathbb{E}(X^{T}X)\Sigma^{-\frac{1}{2}}=n\cdot I$,
we should expect the condition number $\kappa(X_{0}^{T}X_{0})$ to
concentrate around 1, and similarly for $\kappa(X^{T}X)$ to concentrate
around $\kappa(\Sigma)$, so this closeness result is essentially
a result of the concentration of condition numbers, but its particular
form is useful for later results.
\begin{thm}
	Let $X$ be an $n\times p$ random matrix with i.i.d. sub-Gaussian
	rows $X_{i}$ with sub-Gaussian norm $K=\|X_{i}\|_{\psi_{2}}$, $\mathbb{E}X_{i}=0$,
	and let $\Sigma=\mathbb{E}X_{i}^{T}X_{i}=\frac{1}{n}\mathbb{E}X^{T}X$
	be positive definite. Let $X_{0}=X\Sigma^{-\frac{1}{2}}$ be the matrix
	normalized by population covariance matrix. Then for universal constants
	$c,C$, with probability at least $1-2\exp(-\frac{ct^{2}}{K^{4}})-2\exp(-\frac{ct^{2}\sigma_{\min}^{2}(\Sigma)}{K^{4}})$,
	\begin{align*}
	|\kappa(X_{0}^{T}X_{0})-\frac{\kappa(X^{T}X)}{\kappa(\Sigma)}| & \leq\frac{2}{(1-(C\frac{K^{2}}{\sigma_{\min}(\Sigma)})\sqrt{\frac{p}{n}}-\frac{t}{\sqrt{n}})^{2}}\cdot(C\frac{K^{2}}{\sigma_{\min}(\Sigma)}\sqrt{\frac{p}{n}}+\frac{t}{\sqrt{n}})\\
	& +\frac{2}{(1-(CK^{2})\sqrt{\frac{p}{n}}-\frac{t}{\sqrt{n}})^{2}}\cdot(CK^{2}\sqrt{\frac{p}{n}}+\frac{t}{\sqrt{n}})
	\end{align*}
\end{thm}
\proof{Proof}
	Note that 
	\begin{align*}
	\frac{1}{n}\mathbb{E}X_{0}^{T}X_{0} & =\frac{1}{n}\Sigma^{-\frac{1}{2}}\mathbb{E}X^{T}X\Sigma^{-\frac{1}{2}}\\
	& =I
	\end{align*}
	and that $X_{0}$ has i.i.d sub-Gaussian rows with sub-Gaussian norm\textbf{
	}at most\textbf{ $\|\Sigma^{-\frac{1}{2}}\|K$}. This is because the
	$i$-th row of $X_{0}$, which is equal to $X_{i}\Sigma^{-\frac{1}{2}}$,
	satisfies 
	\begin{align*}
	\|X_{i}\Sigma^{-\frac{1}{2}}\|_{\psi_{2}} & =\|\Sigma^{-\frac{1}{2}}X_{i}^{T}\|_{\psi_{2}}\\
	& =\sup_{\|x\|_{2}\leq1}\|\langle\Sigma^{-\frac{1}{2}}X_{i}^{T},x\rangle\|_{\psi_{2}}\\
	& =\sup_{\|x\|_{2}\leq1}\|\langle X_{i}^{T},\Sigma^{-\frac{1}{2}}x\rangle\|_{\psi_{2}}\\
	& =\sup_{\|x\|_{2}\leq1}\|\langle X_{i}^{T},x\rangle\|_{\psi_{2}}\cdot\|\Sigma^{-\frac{1}{2}}\|_{op}\\
	& =\|X_{i}\|_{\psi_{2}}\cdot\|\Sigma^{-\frac{1}{2}}\|_{op}\leq\|\Sigma^{-\frac{1}{2}}\|K
	\end{align*}
	Applying the sub-Gaussian concentration result , we see that for $n$
	sufficiently large,
	\begin{align*}
	\|\frac{1}{n}X^{T}X-\Sigma\|_{op}\leq & CK^{2}\sqrt{\frac{p}{n}}+\frac{t}{\sqrt{n}}\\
	\|\frac{1}{n}X_{0}^{T}X_{0}-I\|_{op} & \leq C\frac{K^{2}}{\sigma_{\min}(\Sigma)}\sqrt{\frac{p}{n}}+\frac{t}{\sqrt{n}}
	\end{align*}
	jointly with probability at least $1-2\exp(-\frac{ct^{2}}{K^{4}})-2\exp(-\frac{ct^{2}\sigma_{\min}^{2}(\Sigma)}{K^{4}})$.
	The eigenvalue stability result then implies 
	\begin{align*}
	|\sigma_{\max}(\frac{1}{n}X^{T}X)-\sigma_{\max}(\Sigma)| & \leq CK^{2}\sqrt{\frac{p}{n}}+\frac{t}{\sqrt{n}}\\
	|\sigma_{\min}(\frac{1}{n}X^{T}X)-\sigma_{\min}(\Sigma)| & \leq CK^{2}\sqrt{\frac{p}{n}}+\frac{t}{\sqrt{n}}
	\end{align*}
	and 
	\begin{align*}
	|\sigma_{\max}(\frac{1}{n}X_{0}^{T}X_{0})-1| & \leq C\frac{K^{2}}{\sigma_{\min}(\Sigma)}\sqrt{\frac{p}{n}}+\frac{t}{\sqrt{n}}\\
	|\sigma_{\min}(\frac{1}{n}X_{0}^{T}X_{0})-1| & \leq C\frac{K^{2}}{\sigma_{\min}(\Sigma)}\sqrt{\frac{p}{n}}+\frac{t}{\sqrt{n}}
	\end{align*}

	It then follows that 
	\begin{align*}
	|\kappa(X^{T}X)-\kappa(\Sigma)| & =|\frac{\sigma_{\max}(\frac{1}{n}X^{T}X)}{\sigma_{\min}(\frac{1}{n}X^{T}X)}-\frac{\sigma_{\max}(\Sigma)}{\sigma_{\min}(\Sigma)}|\\
	& =|\frac{\sigma_{\max}(\frac{1}{n}X^{T}X)\cdot\sigma_{\min}(\Sigma)-\sigma_{\max}(\Sigma)\sigma_{\min}(\frac{1}{n}X^{T}X)}{\sigma_{\min}(\frac{1}{n}X^{T}X)\sigma_{\min}(\Sigma)}|\\
	& \leq|\frac{\sigma_{\max}(\frac{1}{n}X^{T}X)\cdot\sigma_{\min}(\Sigma)-\sigma_{\max}(\Sigma)\cdot\sigma_{\min}(\Sigma)}{\sigma_{\min}(\frac{1}{n}X^{T}X)\sigma_{\min}(\Sigma)}|+\\
	& |\frac{\sigma_{\max}(\Sigma)\cdot\sigma_{\min}(\Sigma)-\sigma_{\max}(\Sigma)\sigma_{\min}(\frac{1}{n}X^{T}X)}{\sigma_{\min}(\frac{1}{n}X^{T}X)\sigma_{\min}(\Sigma)}|\\
	& \leq|\frac{\sigma_{\max}(\frac{1}{n}X^{T}X)-\sigma_{\max}(\Sigma)}{\sigma_{\min}(\frac{1}{n}X^{T}X)}|+\kappa(\Sigma)|\frac{\sigma_{\min}(\Sigma)-\sigma_{\min}(\frac{1}{n}X^{T}X)}{\sigma_{\min}(\frac{1}{n}X^{T}X)}|\\
	& \leq\frac{n}{(\sqrt{n}-(CK^{2})\sqrt{p}-t)^{2}}\cdot\left[CK^{2}\sqrt{\frac{p}{n}}+\frac{t}{\sqrt{n}}\right](\kappa(\Sigma)+1)
	\end{align*}
	and similarly 
	\begin{align*}
	|\kappa(X_{0}^{T}X_{0})-1| & =|\frac{\sigma_{\max}(\frac{1}{n}X^{T}X)}{\sigma_{\min}(\frac{1}{n}X^{T}X)}-1|\\
	& =|\frac{\sigma_{\max}(\frac{1}{n}X^{T}X)-\sigma_{\min}(\frac{1}{n}X^{T}X)}{\sigma_{\min}(\frac{1}{n}X^{T}X)}|\\
	& \leq2\frac{C\frac{K^{2}}{\sigma_{\min}(\Sigma)}\sqrt{\frac{p}{n}}+\frac{t}{\sqrt{n}}}{\frac{(\sqrt{n}-(C\frac{K^{2}}{\sigma_{\min}(\Sigma)})\sqrt{p}-t)^{2}}{n}}=\frac{2n}{(\sqrt{n}-(C\frac{K^{2}}{\sigma_{\min}(\Sigma)})\sqrt{p}-t)^{2}}(C\frac{K^{2}}{\sigma_{\min}(\Sigma)}\sqrt{\frac{p}{n}}+\frac{t}{\sqrt{n}})
	\end{align*}
	Therefore 
	\begin{align*}
	|\kappa(X_{0}^{T}X_{0})-\frac{\kappa(X^{T}X)}{\kappa(\Sigma)}| & \leq\frac{2n}{(\sqrt{n}-(C\frac{K^{2}}{\sigma_{\min}(\Sigma)})\sqrt{p}-t)^{2}}\cdot(C\frac{K^{2}}{\sigma_{\min}(\Sigma)}\sqrt{\frac{p}{n}}+\frac{t}{\sqrt{n}})\\
	& +\frac{2n}{(\sqrt{n}-(CK^{2})\sqrt{p}-t)^{2}}\cdot(CK^{2}\sqrt{\frac{p}{n}}+\frac{t}{\sqrt{n}})\\
	& =\frac{2}{(1-(C\frac{K^{2}}{\sigma_{\min}(\Sigma)})\sqrt{\frac{p}{n}}-\frac{t}{\sqrt{n}})^{2}}\cdot(C\frac{K^{2}}{\sigma_{\min}(\Sigma)}\sqrt{\frac{p}{n}}+\frac{t}{\sqrt{n}})\\
	& +\frac{2}{(1-(CK^{2})\sqrt{\frac{p}{n}}-\frac{t}{\sqrt{n}})^{2}}\cdot(CK^{2}\sqrt{\frac{p}{n}}+\frac{t}{\sqrt{n}})
	\end{align*}
	and if $\sigma_{\min}(\Sigma)\geq1$, then the bound further simplifies
	to 
	\begin{align*}
	|\kappa(X_{0}^{T}X_{0})-\frac{\kappa(X^{T}X)}{\kappa(\Sigma)}| & \leq\frac{4}{(1-(CK^{2})\sqrt{\frac{p}{n}}-\frac{t}{\sqrt{n}})^{2}}\cdot(CK^{2}\sqrt{\frac{p}{n}}+\frac{t}{\sqrt{n}})
	\end{align*}
	\hfill \halmos
\endproof
\begin{cor}
	If in addition to the conditions in the theorem above, the population
	covariance matrix $\Sigma$ satisfies $\sigma_{\min}(\Sigma)\ge1$,
	the bound further simplifies to 
	\begin{align*}
	|\kappa(X_{0}^{T}X_{0})-\frac{\kappa(X^{T}X)}{\kappa(\Sigma)}| & \leq\frac{4}{(1-(CK^{2})\sqrt{\frac{p}{n}}-\frac{t}{\sqrt{n}})^{2}}\cdot(CK^{2}\sqrt{\frac{p}{n}}+\frac{t}{\sqrt{n}})
	\end{align*}
	with probability at least $1-4\exp(-\frac{ct^{2}}{K^{4}})$.
\end{cor}
The same result holds if the sub-Gaussian vector has non-zero mean
$\mu$.
\begin{cor}
	Same assumptions as in the previous theorem, but now with $\mathbb{E}X_{i}=\mu$,
	$\Sigma=\mathbb{E}X_{i}^{T}X_{i}$, and 
	\begin{align*}
	X_{0} & =(X-\mu)(\Sigma-\mu^{T}\mu)^{-\frac{1}{2}}
	\end{align*}
	Then with probability at least $1-2\exp(-\frac{ct^{2}}{K^{4}})-2\exp(-\frac{ct^{2}\sigma_{\min}^{2}(\Sigma)}{K^{4}})$,
	\begin{align*}
	|\kappa(X_{0}^{T}X_{0})-\frac{\kappa(X^{T}X)}{\kappa(\Sigma)}| & \leq\frac{2}{(1-(C\frac{K^{2}}{\sigma_{\min}(\Sigma)})\sqrt{\frac{p}{n}}-\frac{t}{\sqrt{n}})^{2}}\cdot(C\frac{K^{2}}{\sigma_{\min}(\Sigma)}\sqrt{\frac{p}{n}}+\frac{t}{\sqrt{n}})\\
	& +\frac{2}{(1-(CK^{2})\sqrt{\frac{p}{n}}-\frac{t}{\sqrt{n}})^{2}}\cdot(CK^{2}\sqrt{\frac{p}{n}}+\frac{t}{\sqrt{n}})
	\end{align*}
\end{cor}
So far we have shown that the condition number $\kappa(X^{T}X)$ is
close to $\kappa(\Sigma)\cdot\kappa(X_{0}^{T}X_{0})$ with high probability.
Our next step is to prove a similar result for normalization using
batch statistics, in the special case when $\Sigma$ is diagonal,
i.e. the columns of $X$ are also independent. 

When the columns of $X$ are also independent, a similar concentration
holds for sub-Gaussian random matrices, and as a consequence, the
condition number of a matrix normalized with sample statistics is
also smaller by $\kappa(\Sigma)$ with high probability. 
\begin{lem}
	(\cite{rudelson2010non}\label{lem:concentration_column})Let $X$
	be an $n\times p$ matrix with $n\geq p$ whose columns $X_{j}$ are
	i.i.d. sub-gaussian random vectors with $\|X_{j}\|_{2}=\sqrt{n}$
	almost surely, $K=\|X_{j}\|_{\psi_{2}}$, and $\frac{1}{n}\mathbb{E}X^{T}X=I$.
	Then for universal constants $c,C$ and every $t\geq0$, with probability
	at least $1-2\exp(-\frac{ct^{2}}{K^{4}})$, 
	\begin{align*}
	\|\frac{1}{n}X^{T}X-I\|_{op} & \le CK^{2}\sqrt{\frac{p}{n}}+\frac{t}{\sqrt{n}}
	\end{align*}
	and 
	\begin{align*}
	\sqrt{n}-(CK^{2})\sqrt{p}-t\leq\sigma_{\min}(X)\leq\sigma_{\max}(X) & \leq\sqrt{n}+(CK^{2})\sqrt{p}+t
	\end{align*}
\end{lem}
%
\begin{comment}
Consider a sub-Gaussian distribution in $\mathbb{R}^{p}$ with covariance
matrix $\Sigma$, and let $\varepsilon\in(0,1),t\geq1$. If $X$ is
an $n\times p$ random matrix with i.i.d rows drawn from this sub-Gaussian
distribution, with probability at least $1-2\exp(-t^{2}p)$, and $\Sigma_{n}=\frac{1}{n}X^{T}X$
\begin{align*}
\|\Sigma_{N}-\Sigma\| & \leq\varepsilon
\end{align*}
if $N\geq C(t/\varepsilon)^{2}n$, where $C$ is a constant that
depends only on the sub-Gaussian norm $K$ of the random vector. 
\end{comment}

\begin{thm}
	Let $X$ be an $n\times p$ random matrix with i.i.d. sub-Gaussian
	rows $X_{i}$, $\mathbb{E}X_{i}=0$, and let $\Sigma=\mathbb{E}X_{i}^{T}X_{i}=\frac{1}{n}\mathbb{E}X^{T}X$
	be \textbf{diagonal }and positive definite. Let $\hat{\Sigma}$ be
	the diagonal matrix with $\hat{\Sigma}_{jj}=\frac{1}{n}(X^{T}X)_{jj}$.
	Let $X_{0}:=X\hat{\Sigma}^{-\frac{1}{2}}$ be the normalized matrix.
	Then for universal constants $c,C$, and $K=\max_{j}\|X_{j}\|_{\psi_{2}}$
	where $X_{j}$ is the $j$-th column of $X$, with probability at
	least $1-4\exp(-\frac{ct^{2}}{K^{4}})-2\exp(-\frac{ct^{2}\sigma_{\min}^{2}(\Sigma)-(CK^{2}\sqrt{\frac{p}{n}}+\frac{t}{\sqrt{n}})}{K^{4}})$, 
	
	\begin{align*}
	|\kappa(X_{0}^{T}X_{0})-\frac{\kappa(X^{T}X)}{\kappa(\Sigma)}| & \leq\frac{2}{(1-(\frac{K^{2}}{\sigma_{\min}(\Sigma)-(CK^{2}\sqrt{\frac{p}{n}}+\frac{t}{\sqrt{n}})})\sqrt{\frac{p}{n}}-\frac{t}{\sqrt{n}})^{2}}\cdot(C\frac{K^{2}}{\sigma_{\min}(\Sigma)-(CK^{2}\sqrt{\frac{p}{n}}+\frac{t}{\sqrt{n}})}\sqrt{\frac{p}{n}}+\frac{t}{\sqrt{n}})\\
	& +\frac{2}{(1-(CK^{2})\sqrt{\frac{p}{n}}-\frac{t}{\sqrt{n}})^{2}}\cdot(CK^{2}\sqrt{\frac{p}{n}}+\frac{t}{\sqrt{n}})
	\end{align*}
\end{thm}
\proof{Proof}
	First note that since $\Sigma$ is diagonal, the entries of $X$ are
	independent. As a result, the sub-Gaussian norm of each row $X_{i}$
	of $X$ is bounded above by the sub-Gaussian norm of the maximum of
	the sub-Gaussian norm of its entries, which is in turn bounded above
	by $K$. 
	
	Matrix concentration \ref{lem:sub-Gaussian-concentration} then implies
	with probability at least $1-2\exp(-\frac{ct^{2}}{K^{4}}),$
	\begin{align*}
	\|\frac{1}{n}X^{T}X-\Sigma\|_{op} & \leq CK^{2}\sqrt{\frac{p}{n}}+\frac{t}{\sqrt{n}}
	\end{align*}
	On the other hand,
	\begin{align*}
	\mathbb{E}\frac{1}{n}X_{0}^{T}X_{0} & =I
	\end{align*}
	where now $X_{0}$ has independent columns but not independent rows.
	In addition, for each row $i$ of $X_{0}$, it holds true that 
	\begin{align*}
	\mathbb{E}(X_{0})_{i}^{T}(X_{0})_{i} & =I
	\end{align*}
	This is because of the identity 
	\begin{align*}
	\sum_{i}(X_{0})_{i}^{T}(X_{0})_{i} & =X_{0}^{T}X_{0}
	\end{align*}
	and by symmetry, 
	\begin{align*}
	\mathbb{E}(X_{0})_{i}^{T}(X_{0})_{i} & =\mathbb{E}(X_{0})_{j}^{T}(X_{0})_{j}
	\end{align*}
	for all $i,j$. 
	
	Note also that each column of $X_{0}$ satisfies $\|(X_{0}^{T})_{j}\|_{2}=\sqrt{n}$
	by construction, and the columns are independent. In order to apply
	the concentration result \ref{lem:concentration_column} on matrices
	with independent columns, we need a bound on the sub-Gaussian norm
	of the columns of $X_{0}$. 
	
	Since $X_{0}=X\hat{\Sigma}^{-\frac{1}{2}}$, the rows of $X_{0}$
	have sub-Gaussian norm of at most $\sqrt{\frac{K^{2}}{\sigma_{\min}(\hat{\Sigma})}}$.
	Moreover, since $\hat{\Sigma}$ is diagonal, the columns of $X_{0}$
	also have sub-Gaussian norm of at most $\sqrt{\frac{K^{2}}{\sigma_{\min}(\hat{\Sigma})}}$.
	The entries of each column of $X_{0}$ are no longer independent,
	due to normalization, but are still uncorrelated, as their products
	have symmetric distributions. Recall that $\hat{\Sigma}_{jj}=\frac{1}{n}(X^{T}X)_{jj}$.
	The relationship between infinity and operator norm implies 
	\begin{align*}
	\|\hat{\Sigma}-\Sigma\|_{op}=\|\hat{\Sigma}-\Sigma\|_{\infty}\leq\|\frac{1}{n}X^{T}X-\Sigma\|_{\infty}\leq\|\frac{1}{n}X^{T}X-\Sigma\|_{op} & \leq CK^{2}\sqrt{\frac{p}{n}}+\frac{t}{\sqrt{n}}
	\end{align*}
	
	We can conclude that the sub-Gaussian norm of columns of $X\hat{\Sigma}^{-\frac{1}{2}}$
	is bounded above by $\sqrt{\frac{K^{2}}{\sigma_{\min}(\Sigma)-(CK^{2}\sqrt{\frac{p}{n}}+\frac{t}{\sqrt{n}})}}$,
	with probability at least $1-2\exp(-\frac{ct^{2}}{K^{4}})$. Thus
	the concentration result on random matrices with independent columns
	apply, and with probability at least $1-2\exp(-\frac{ct^{2}}{K^{4}})-2\exp(-\frac{ct^{2}\sigma_{\min}^{2}(\Sigma)-(CK^{2}\sqrt{\frac{p}{n}}+\frac{t}{\sqrt{n}})}{K^{4}})$, 
	
	\begin{align*}
	\|\frac{1}{n}X_{0}^{T}X_{0}-I\|_{op} & \le C\frac{K^{2}}{\sigma_{\min}(\Sigma)-(CK^{2}\sqrt{\frac{p}{n}}+\frac{t}{\sqrt{n}})}\sqrt{\frac{p}{n}}+\frac{t}{\sqrt{n}}
	\end{align*}
	This combined with 
	\begin{align*}
	\|\frac{1}{n}X^{T}X-\Sigma\|_{op} & \leq CK^{2}\sqrt{\frac{p}{n}}+\frac{t}{\sqrt{n}}
	\end{align*}
	lets us conclude that with probability $1-4\exp(-\frac{ct^{2}}{K^{4}})-2\exp(-\frac{ct^{2}\sigma_{\min}^{2}(\Sigma)-(CK^{2}\sqrt{\frac{p}{n}}+\frac{t}{\sqrt{n}})}{K^{4}})$,
	\begin{align*}
	|\kappa(X_{0}^{T}X_{0})-\frac{\kappa(X^{T}X)}{\kappa(\Sigma)}| & \leq\frac{2}{(1-(\frac{K^{2}}{\sigma_{\min}(\Sigma)-(CK^{2}\sqrt{\frac{p}{n}}+\frac{t}{\sqrt{n}})})\sqrt{\frac{p}{n}}-\frac{t}{\sqrt{n}})^{2}}\cdot(C\frac{K^{2}}{\sigma_{\min}(\Sigma)-(CK^{2}\sqrt{\frac{p}{n}}+\frac{t}{\sqrt{n}})}\sqrt{\frac{p}{n}}+\frac{t}{\sqrt{n}})\\
	& +\frac{2}{(1-(CK^{2})\sqrt{\frac{p}{n}}-\frac{t}{\sqrt{n}})^{2}}\cdot(CK^{2}\sqrt{\frac{p}{n}}+\frac{t}{\sqrt{n}})
	\end{align*}
	and as before, with sufficiently large $n$ and $\sigma_{\min}(\Sigma)\geq1$,
	the bound simplifies to 
	\begin{align*}
	|\kappa(X_{0}^{T}X_{0})-\frac{\kappa(X^{T}X)}{\kappa(\Sigma)}| & \leq\frac{4}{(1-(CK^{2})\sqrt{\frac{p}{n}}-\frac{t}{\sqrt{n}})^{2}}\cdot(CK^{2}\sqrt{\frac{p}{n}}+\frac{t}{\sqrt{n}})
	\end{align*}
	\hfill \halmos
\endproof
\begin{cor}
	If in addition to the conditions in the theorem above, the population
	covariance matrix $\Sigma$ satisfies $\sigma_{\min}(\Sigma)\ge1$,
	the bound further simplifies to 
	\begin{align*}
	|\kappa(X_{0}^{T}X_{0})-\frac{\kappa(X^{T}X)}{\kappa(\Sigma)}| & \leq\frac{4}{(1-(CK^{2})\sqrt{\frac{p}{n}}-\frac{t}{\sqrt{n}})^{2}}\cdot(CK^{2}\sqrt{\frac{p}{n}}+\frac{t}{\sqrt{n}})
	\end{align*}
	with probability at least $1-4\exp(-\frac{ct^{2}}{K^{4}})-2\exp(-\frac{ct^{2}-(CK^{2}\sqrt{\frac{p}{n}}+\frac{t}{\sqrt{n}})}{K^{4}})$.
\end{cor}
\begin{cor}
	Same assumptions as in the previous theorem, but now with $\mathbb{E}X_{i}=\mu$,
	$\Sigma=\mathbb{E}X_{i}^{T}X_{i}$. Let $\hat{\mu}=\frac{1}{n}\sum_{i}X_{i}$
	be the sample mean of the columns, and $\hat{D}$ be the diagonal
	matrix with entries $\hat{D}_{ii}=\frac{1}{n}\sum_{j}(X_{ji}-\hat{\mu}_{i})^{2}$,
	or equivalently $\hat{D}$ is the diagonal of the empirical covariance
	matrix $\frac{1}{n}(X-\hat{\mu})^{T}(X-\hat{\mu})$. If we center
	and normalize $X$ with sample statistics:
	\begin{align*}
	X_{0} & =(X-\hat{\mu})\hat{D}^{-\frac{1}{2}}
	\end{align*}
	Then with probability at least $1-4\exp(-\frac{ct^{2}}{K^{4}})-2\exp(-\frac{ct^{2}\sigma_{\min}^{2}(\Sigma)-(CK^{2}\sqrt{\frac{p}{n}}+\frac{t}{\sqrt{n}})}{K^{4}})$,
	\begin{align*}
	|\kappa(X_{0}^{T}X_{0})-\frac{\kappa(X^{T}X)}{\kappa(\Sigma)}| & \leq\frac{2}{(1-(C\frac{K^{2}}{\sigma_{\min}(\Sigma)})\sqrt{\frac{p}{n}}-\frac{t}{\sqrt{n}})^{2}}\cdot(C\frac{K^{2}}{\sigma_{\min}(\Sigma)}\sqrt{\frac{p}{n}}+\frac{t}{\sqrt{n}})\\
	& +\frac{2}{(1-(CK^{2})\sqrt{\frac{p}{n}}-\frac{t}{\sqrt{n}})^{2}}\cdot(CK^{2}\sqrt{\frac{p}{n}}+\frac{t}{\sqrt{n}})
	\end{align*}
\end{cor}
So far our two results state that 
\begin{itemize}
	\item On one hand, for data matrix $X$ with general covariance matrix not
	necessarily diagonal, if we have access to the population covariace
	$\Sigma$ itself, then preconditioning $X$ by $\Sigma^{-\frac{1}{2}}$
	reduces the condition number by $\kappa(\Sigma)$ with high probability.
	\item On the other hand, if we don't have access to the population covariance
	$\Sigma$ but we know $\Sigma$ is diagonal, then preconditioning
	$X$ by $\hat{\Sigma}^{-\frac{1}{2}}$, where $\hat{\Sigma}$ is the
	diagonal matrix with entries equal to the norms squared of each column,
	also reduces the condition number by $\kappa(\Sigma)$ with high probability.
\end{itemize}
To work towards the ultimate goal of preconditioning with the column
sample standard deviations, we next consider the setting where the
covariance matrix $\Sigma$ is not necessarily diagonal, and show
that preconditioning by the diagonal matrices $D=\text{diag}(\Sigma)$
still results in the concentration of the condition number of the
preconditioned matrix $XD^{-\frac{1}{2}}$, this time towards that
of $\sqrt{\frac{\kappa(\Sigma)}{\kappa(D)}}$.%
\begin{comment}
\textbf{ Note that if we precondition by $(X^{T}X)^{-\frac{1}{2}}$,
then the resulting matrix will have condition number 1, which is the
best that can be achieved. The point is then that diagonal preconditioning
is simpler to implement, and does not involve inverting a matrix.
More precisely, computing the diagonal preconditioner $\hat{\Sigma}^{-\frac{1}{2}}$
requires $np+p$ calculations, while computing $(X^{T}X)^{-\frac{1}{2}}$
requires $np^{2}+p^{3}$ calculations. }
\end{comment}

\begin{comment}
Let $X$ be an $n\times p$ random matrix with i.i.d. sub-Gaussian
entries $X_{ij}$. Let $X_{i}$ be the i-th column of $X$ with $K=\|X_{i}\|_{\psi_{2}}$,
$\mathbb{E}X_{i}=0$, and let $\Sigma=\mathbb{E}X_{i}X_{i}^{T}=\frac{1}{n}\mathbb{E}X^{T}X$
be diagonal and positive definite. Let $\hat{\mu}_{i}$ be the sample
mean of column $i$, and $\hat{\Sigma}$ be the sample covariance
matrix, i.e. $\hat{\Sigma}_{jj}=\frac{1}{n}((X-\hat{\mu})^{T}(X-\hat{\mu}))_{jj}$.
Let $X_{0}:=(X-\hat{\mu})\hat{\Sigma}^{-\frac{1}{2}}$ be the matrix
normalized by sample estimator of covariance matrix. Then for universal
constants $c,C$, with probability at least $1-4\exp(-\frac{ct^{2}}{K^{4}})$, 

Matrix concentration and eigenvalue stability imply 
\begin{align*}
\|\frac{1}{n}X^{T}X-\Sigma\|_{op} & \leq CK^{2}\sqrt{\frac{p}{n}}+\frac{t}{\sqrt{n}}
\end{align*}
Moreover, 
\begin{align*}
\mathbb{E}\frac{1}{n}X_{0}^{T}X_{0} & =I
\end{align*}
where now $X_{0}$ has independent columns but not independent rows. 
\end{comment}

\begin{thm}
	Let $X$ be an $n\times p$ random matrix with i.i.d. sub-Gaussian
	rows $X_{i}$ with $K=\|X_{i}\|_{\psi_{2}}$, $\mathbb{E}X_{i}=0$,
	and let $\Sigma=\mathbb{E}X_{i}^{T}X_{i}=\frac{1}{n}\mathbb{E}X^{T}X$
	be the population covariance matrix. Let $D$ be the diagonal matirix
	with $D_{ii}=\Sigma_{ii}$, and let $X_{0}:=XD^{-\frac{1}{2}}$ the
	matrix normalized with diagonal entries of $\Sigma$. Then with probability
	at least $1-2\exp(-\frac{ct^{2}(\min_{i}(\Sigma)_{ii})^{2}}{K^{4}})-2\exp(-\frac{ct^{2}}{K^{4}})$,
	\begin{align*}
	|\frac{\kappa(X^{T}X)}{\kappa(\Sigma)}- & \frac{\kappa(X_{0}^{T}X_{0})}{\kappa(D^{-\frac{1}{2}}\Sigma D^{-\frac{1}{2}})}|\leq\frac{2}{(1-(CK^{2})\sqrt{\frac{p}{n}}-\frac{t}{\sqrt{n}})^{2}}\cdot\left[CK^{2}\sqrt{\frac{p}{n}}+\frac{t}{\sqrt{n}}\right]\\
	& +\frac{2}{(1-(C\frac{K^{2}}{\min_{i}(\Sigma)_{ii}})\sqrt{\frac{p}{n}}-\frac{t}{\sqrt{n}})^{2}}\cdot\left[C\frac{K^{2}}{\min_{i}(\Sigma)_{ii}}\sqrt{\frac{p}{n}}+\frac{t}{\sqrt{n}}\right]
	\end{align*}
\end{thm}
\proof{Proof}
	Note that $\mathbb{E}\frac{1}{n}X_{0}^{T}X_{0}=D^{-\frac{1}{2}}\Sigma D^{-\frac{1}{2}}$,
	i.e. the population correlation matrix. Moreover, the sub-Gaussian
	norm of $X_{0}=XD^{-\frac{1}{2}}$ is bounded above by $\|D^{-\frac{1}{2}}\|_{op}K$.
	By matrix concentration, with probability at least $1-2\exp(-\frac{ct^{2}(\min_{i}(\Sigma)_{ii})^{2}}{K^{4}})-2\exp(-\frac{ct^{2}}{K^{4}})$,
	the following two inequalities hold simultaneously
	\begin{align*}
	\|\frac{1}{n}X_{0}^{T}X_{0}-D^{-\frac{1}{2}}\Sigma D^{-\frac{1}{2}}\|_{op} & \leq C\frac{K^{2}}{\min_{i}(\Sigma)_{ii}}\sqrt{\frac{p}{n}}+\frac{t}{\sqrt{n}}\\
	\|\frac{1}{n}X^{T}X-\Sigma\|_{op} & \leq CK^{2}\sqrt{\frac{p}{n}}+\frac{t}{\sqrt{n}}
	\end{align*}
	and as a result 
	\begin{align*}
	|\kappa(X^{T}X)-\kappa(\Sigma)| & \leq\frac{1}{(1-(CK^{2})\sqrt{\frac{p}{n}}-\frac{t}{\sqrt{n}})^{2}}\cdot\left[CK^{2}\sqrt{\frac{p}{n}}+\frac{t}{\sqrt{n}}\right](\kappa(\Sigma)+1)
	\end{align*}
	and similarly 
	\begin{align*}
	|\kappa(X_{0}^{T}X_{0})-\kappa(D^{-\frac{1}{2}}\Sigma D^{-\frac{1}{2}})| & \leq\frac{1}{(1-(C\frac{K^{2}}{\min_{i}(\Sigma)_{ii}})\sqrt{\frac{p}{n}}-\frac{t}{\sqrt{n}})^{2}}\cdot\left[C\frac{K^{2}}{\min_{i}(\Sigma)_{ii}}\sqrt{\frac{p}{n}}+\frac{t}{\sqrt{n}}\right](\kappa(D^{-\frac{1}{2}}\Sigma D^{-\frac{1}{2}})+1)
	\end{align*}
	Therefore 
	\begin{align*}
	|\frac{\kappa(X^{T}X)}{\kappa(\Sigma)}- & \frac{\kappa(X_{0}^{T}X_{0})}{\kappa(D^{-\frac{1}{2}}\Sigma D^{-\frac{1}{2}})}|\leq\frac{2}{(1-(CK^{2})\sqrt{\frac{p}{n}}-\frac{t}{\sqrt{n}})^{2}}\cdot\left[CK^{2}\sqrt{\frac{p}{n}}+\frac{t}{\sqrt{n}}\right]\\
	& +\frac{2}{(1-(C\frac{K^{2}}{\min_{i}(\Sigma)_{ii}})\sqrt{\frac{p}{n}}-\frac{t}{\sqrt{n}})^{2}}\cdot\left[C\frac{K^{2}}{\min_{i}(\Sigma)_{ii}}\sqrt{\frac{p}{n}}+\frac{t}{\sqrt{n}}\right]
	\end{align*}
	which again simplifies to $\frac{2}{(1-(CK^{2})\sqrt{\frac{p}{n}}-\frac{t}{\sqrt{n}})^{2}}\cdot\left[CK^{2}\sqrt{\frac{p}{n}}+\frac{t}{\sqrt{n}}\right]$
	if the diagonal entries of $\Sigma$ are bounded below by 1. 
	\hfill \halmos
\endproof
\begin{cor}
	Same assumptions as in the previous theorem, but now with $\mathbb{E}X_{i}=\mu$,
	$\Sigma=\mathbb{E}X_{i}^{T}X_{i}$. Let $D$ be the diagonal matrix
	with $D_{ii}=(\Sigma-\mu^{T}\mu)_{ii}$. If we center and normalize
	$X$ with population statistics:
	\begin{align*}
	X_{0} & =(X-\mu)(D)^{-\frac{1}{2}}
	\end{align*}
	Then with probability at least $1-2\exp(-\frac{ct^{2}(\min_{i}D_{ii})^{2}}{K^{4}})-2\exp(-\frac{ct^{2}}{K^{4}})$,
	\begin{align*}
	|\frac{\kappa(X^{T}X)}{\kappa(\Sigma)}- & \frac{\kappa(X_{0}^{T}X_{0})}{\kappa(D^{-\frac{1}{2}}(\Sigma-\mu^{T}\mu)D^{-\frac{1}{2}})}|\leq\frac{2}{(1-(CK^{2})\sqrt{\frac{p}{n}}-\frac{t}{\sqrt{n}})^{2}}\cdot\left[CK^{2}\sqrt{\frac{p}{n}}+\frac{t}{\sqrt{n}}\right]\\
	& +\frac{2}{(1-(C\frac{K^{2}}{\min_{i}D_{ii}})\sqrt{\frac{p}{n}}-\frac{t}{\sqrt{n}})^{2}}\cdot\left[C\frac{K^{2}}{\min_{i}D_{ii}}\sqrt{\frac{p}{n}}+\frac{t}{\sqrt{n}}\right]
	\end{align*}
\end{cor}
The above result says that if we normalize by the diagonal of the
population covariance matrix, i.e. the population standard deviations,
then we would get a reduction in condition number of $XD^{-\frac{1}{2}}$
on the order close to $\sqrt{\frac{\kappa(\Sigma)}{\kappa(D^{-\frac{1}{2}}\Sigma D^{-\frac{1}{2}})}}$.
Thus if the population covariance $\Sigma$ has large condition number
while the population correlation matrix $D^{-\frac{1}{2}}\Sigma D^{-\frac{1}{2}}$
has small condition number, the reduction is large. However, the ratio
$\frac{\kappa(\Sigma)}{\kappa(D^{-\frac{1}{2}}\Sigma D^{-\frac{1}{2}})}$
is not always small, and in fact is not always bounded below by 1.
In the next section, we analyze situations when the ratio is small
for special classes of covariance matrices. 

Now what is left to be proved is the most general version of condition
number reduction with diagonal preconditioning, namely using sample
standard deviations instead of population standard deviations. 
\begin{thm}
	(Theorem \ref{thm:concentration_1} in paper) Let $X$ be an $n\times p$
	random matrix with i.i.d. sub-Gaussian rows $X_{i}$ with $K=\|X_{i}\|_{\psi_{2}}$
	the sub-Gaussian norm of its rows, $\mathbb{E}X_{i}=0$, and let $\Sigma=\mathbb{E}X_{i}^{T}X_{i}=\frac{1}{n}\mathbb{E}X^{T}X$
	be the population covariance matrix. Let $\hat{D}$ be the diagonal
	matrix with $\hat{D}_{ii}=(X^{T}X)_{ii}$, i.e. $\hat{D}_{ii}$ is
	the norm squared of the $i$-th column of $X$, and let $X_{0}=X\hat{D}^{-\frac{1}{2}}$
	be the matrix normalized with diagonal entries of $\hat{D}$. Let
	$D=\text{diag}(\Sigma)$. Then with probability at least $1-2\exp(-\frac{ct^{2}(\min_{i}(\Sigma)_{ii})^{2}}{K^{4}})-2\exp(-\frac{ct^{2}}{K^{4}})-2p\exp(-\frac{c}{K^{4}}\left[K^{2}+\frac{\min_{i}(\Sigma)_{ii}}{\sqrt{p}}\cdot t\right]^{2})$,
	\begin{align*}
	|\frac{\kappa(X^{T}X)}{\kappa(\Sigma)}- & \frac{\kappa(X_{0}^{T}X_{0})}{\kappa(D^{-\frac{1}{2}}\Sigma D^{-\frac{1}{2}})}|\leq\frac{2}{(1-(CK^{2})\sqrt{\frac{p}{n}}-\frac{t}{\sqrt{n}})^{2}}\cdot\left[CK^{2}\sqrt{\frac{p}{n}}+\frac{t}{\sqrt{n}}\right]\\
	& +\frac{2}{(1-(C\frac{K^{2}}{\min_{i}(\Sigma)_{ii}})\sqrt{\frac{p}{n}}-3\frac{t}{\sqrt{n}})^{2}}\cdot\left[C\frac{K^{2}}{\min_{i}(\Sigma)_{ii}}\sqrt{\frac{p}{n}}+3\frac{t}{\sqrt{n}}\right]
	\end{align*}
\end{thm}
\proof{Proof}
	Since the rows of $X$ are independent, its columns are sub-Gaussian
	vectors with independent entries with sub-Gaussian norm bounded above
	by $K$. Standard concentration result of the norm implies that with
	probability at least $1-2\exp(-\frac{cT^{2}}{K^{4}})$, 
	\begin{align*}
	|\hat{D}_{ii}^{\frac{1}{2}}-D_{ii}^{\frac{1}{2}}| & \leq T
	\end{align*}
	for all large $T$. Union bound then gives that with probability
	at least $1-2p\exp(-\frac{cT^{2}}{K^{4}})$, 
	\begin{align*}
	|\hat{D}_{ii}^{\frac{1}{2}}-D_{ii}^{\frac{1}{2}}| & \leq T,\forall i
	\end{align*}
	so that 
	\begin{align*}
	|\frac{\hat{D}_{ii}^{\frac{1}{2}}}{D_{ii}^{\frac{1}{2}}}-1| & \leq T\frac{1}{\sqrt{\min_{i}(\Sigma)_{ii}}}
	\end{align*}
	For any $i,j$, let $X_{i}$ denote the $i$th row of $X$, we have
	\begin{align*}
	|\hat{D}_{ii}^{-\frac{1}{2}}X_{i}^{T}X_{j}\hat{D}_{jj}^{-\frac{1}{2}}-D_{ii}^{-\frac{1}{2}}X_{i}^{T}X_{j}D_{jj}^{-\frac{1}{2}}| & \leq\|X_{i}^{T}\|_{2}\|X_{j}^{T}\|_{2}|\hat{D}_{ii}^{-\frac{1}{2}}\hat{D}_{jj}^{-\frac{1}{2}}-D_{ii}^{-\frac{1}{2}}D_{jj}^{-\frac{1}{2}}|\\
	& =|\hat{D}_{ii}^{\frac{1}{2}}\hat{D}_{jj}^{\frac{1}{2}}|\cdot|\hat{D}_{ii}^{-\frac{1}{2}}\hat{D}_{jj}^{-\frac{1}{2}}-D_{ii}^{-\frac{1}{2}}D_{jj}^{-\frac{1}{2}}|\\
	& =|1-\frac{\hat{D}_{ii}^{\frac{1}{2}}\hat{D}_{jj}^{\frac{1}{2}}}{D_{ii}^{\frac{1}{2}}D_{jj}^{\frac{1}{2}}}|=|1-\frac{\hat{D}_{ii}^{\frac{1}{2}}}{D_{ii}^{\frac{1}{2}}}+\frac{\hat{D}_{ii}^{\frac{1}{2}}}{D_{ii}^{\frac{1}{2}}}-\frac{\hat{D}_{ii}^{\frac{1}{2}}\hat{D}_{jj}^{\frac{1}{2}}}{D_{ii}^{\frac{1}{2}}D_{jj}^{\frac{1}{2}}}|\\
	& \leq|1-\frac{\hat{D}_{ii}^{\frac{1}{2}}}{D_{ii}^{\frac{1}{2}}}|+|\frac{\hat{D}_{ii}^{\frac{1}{2}}}{D_{ii}^{\frac{1}{2}}}-\frac{\hat{D}_{ii}^{\frac{1}{2}}\hat{D}_{jj}^{\frac{1}{2}}}{D_{ii}^{\frac{1}{2}}D_{jj}^{\frac{1}{2}}}|\\
	& \leq T\frac{1}{\sqrt{\min_{i}(\Sigma)_{ii}}}(1+\frac{\hat{D}_{ii}^{\frac{1}{2}}}{D_{ii}^{\frac{1}{2}}})\le2\frac{T^{2}}{\min_{i}(\Sigma)_{ii}}
	\end{align*}
	for all large $T$. %
	{} 
	
	The relation between operator norm and maximum entry of a matrix $A$,
	$\|A\|_{op}\leq\sqrt{np}\cdot\max_{i,j}|A_{ij}|$ then implies that 
	
	\begin{align*}
	\|\frac{1}{n}D^{-\frac{1}{2}}X^{T}XD^{-\frac{1}{2}}-\frac{1}{n}\hat{D}^{-\frac{1}{2}}X^{T}X\hat{D}^{-\frac{1}{2}}\|_{op} & \leq\sqrt{np}\cdot\frac{1}{n}\max_{i,j}|\hat{D}_{ii}^{-\frac{1}{2}}X_{i}^{T}X_{j}\hat{D}_{jj}^{-\frac{1}{2}}-D_{ii}^{-\frac{1}{2}}X_{i}^{T}X_{j}D_{jj}^{-\frac{1}{2}}|\\
	& \leq2\frac{T^{2}}{\min_{i}(\Sigma)_{ii}}\cdot\sqrt{\frac{p}{n}}
	\end{align*}
	
	Now recall the result from Theorem 5, that with probability at least
	$1-2\exp(-\frac{ct^{2}(\min_{i}(\Sigma)_{ii})^{2}}{K^{4}})-2\exp(-\frac{ct^{2}}{K^{4}})$,
	the following two inequalities hold simultaneously
	\begin{align*}
	\|\frac{1}{n}D^{-\frac{1}{2}}X^{T}XD^{-\frac{1}{2}}-D^{-\frac{1}{2}}\Sigma D^{-\frac{1}{2}}\|_{op} & \leq C\frac{K^{2}}{\min_{i}(\Sigma)_{ii}}\sqrt{\frac{p}{n}}+\frac{t}{\sqrt{n}}\\
	\|\frac{1}{n}X^{T}X-\Sigma\|_{op} & \leq CK^{2}\sqrt{\frac{p}{n}}+\frac{t}{\sqrt{n}}
	\end{align*}
	Now choose $T$ such that $T^{2}=K^{2}+\frac{\min_{i}(\Sigma)_{ii}}{\sqrt{p}}\cdot t$,
	we see that 
	\begin{align*}
	\|\frac{1}{n}D^{-\frac{1}{2}}X^{T}XD^{-\frac{1}{2}}-\frac{1}{n}\hat{D}^{-\frac{1}{2}}X^{T}X\hat{D}^{-\frac{1}{2}}\|_{op} & \leq2\frac{K^{2}}{\min_{i}(\Sigma)_{ii}}\cdot\sqrt{\frac{p}{n}}+2\frac{t}{\sqrt{n}}
	\end{align*}
	so that 
	\begin{align*}
	\|\frac{1}{n}\hat{D}^{-\frac{1}{2}}X^{T}X\hat{D}^{-\frac{1}{2}}-D^{-\frac{1}{2}}\Sigma D^{-\frac{1}{2}}\|_{op} & \leq C\frac{K^{2}}{\min_{i}(\Sigma)_{ii}}\sqrt{\frac{p}{n}}+3\frac{t}{\sqrt{n}}\\
	\|\frac{1}{n}X^{T}X-\Sigma\|_{op} & \leq CK^{2}\sqrt{\frac{p}{n}}+\frac{t}{\sqrt{n}}
	\end{align*}
	and eigenvalue stability result \ref{lem:weyl} allows us to conclude
	that 
	\begin{align*}
	|\frac{\kappa(X^{T}X)}{\kappa(\Sigma)}-\frac{\kappa(X_{0}^{T}X_{0})}{\kappa(D^{-\frac{1}{2}}\Sigma D^{-\frac{1}{2}})}| & \leq\frac{2}{(1-(CK^{2})\sqrt{\frac{p}{n}}-\frac{t}{\sqrt{n}})^{2}}\cdot\left[CK^{2}\sqrt{\frac{p}{n}}+\frac{t}{\sqrt{n}}\right]\\
	& +\frac{2}{(1-(C\frac{K^{2}}{\min_{i}(\Sigma)_{ii}})\sqrt{\frac{p}{n}}-3\frac{t}{\sqrt{n}})^{2}}\cdot\left[C\frac{K^{2}}{\min_{i}(\Sigma)_{ii}}\sqrt{\frac{p}{n}}+3\frac{t}{\sqrt{n}}\right]
	\end{align*}
	with probability at least 
	\begin{align*}
	1-2\exp(-\frac{ct^{2}(\min_{i}(\Sigma)_{ii})^{2}}{K^{4}})-2\exp(-\frac{ct^{2}}{K^{4}})-2p\exp(-\frac{c}{K^{4}}\left[K^{2}+\frac{\min_{i}(\Sigma)_{ii}}{\sqrt{p}}\cdot t\right]^{2})
	\end{align*}
	\hfill \halmos
\endproof
