# Supplementary material for: Optimal Diagonal Preconditioning
Source: arXiv:2209.00809 source file (2022-11-04)
Supplement: Supplementary file 2 [file appendix_right_precond_res.tex]

\section{Detailed Experiment Results for Right Preconditioning}
\label{app:right}
\begin{table}[H]
\centering
  \begin{tabular}{ccccccc}
    \hline
    Mat & Size & Cbef & Caft & Cdiag & Reduce & Time\\
    \hline
    abb313 & 176 & 3.719000e+07 & 3.146000e+07 & 6.779000e+07 & 0.154092 &
    0.374230\\
    ash219 & 85 & 9.150000e+00 & 4.194000e+00 & 4.690000e+00 & 0.541579 &
    0.171661\\
    ash292 & 292 & 4.188000e+07 & 6.040000e+06 & 2.645000e+07 & 0.855788 &
    1.126949\\
    ash331 & 104 & 9.588000e+00 & 3.668000e+00 & 4.084000e+00 & 0.617469 &
    0.226226\\
    ash608 & 188 & 1.138000e+01 & 3.861000e+00 & 4.317000e+00 & 0.660595 &
    0.435684\\
    ash85 & 85 & 2.151000e+05 & 1.283000e+05 & 1.839000e+05 & 0.403496 &
    0.204586\\
    ash958 & 292 & 1.025000e+01 & 4.757000e+00 & 4.317000e+00 & 0.535855 &
    0.623655\\
    bcspwr01 & 39 & 2.756000e+03 & 2.164000e+03 & 2.559000e+03 & 0.214776 &
    0.743860\\
    bcspwr02 & 49 & 1.856000e+07 & 6.563000e+06 & 1.200000e+07 & 0.646473 &
    0.134231\\
    bcspwr03 & 118 & 2.514000e+05 & 1.137000e+05 & 1.814000e+05 & 0.547642 &
    0.274450\\
    bcspwr04 & 274 & 2.558000e+07 & 6.589000e+06 & 2.436000e+07 & 0.742365 &
    1.315488\\
    bcspwr05 & 443 & 2.681000e+07 & 1.200000e+07 & 1.764000e+07 & 0.552557 &
    0.819582\\
    bcsstk02 & 66 & 1.871000e+07 & 2.973000e+06 & 4.023000e+06 & 0.841086 &
    0.162481\\
    bcsstk05 & 153 & 2.982000e+07 & 1.672000e+06 & 3.286000e+06 & 0.943950 &
    0.596362\\
    bcsstk06 & 420 & 2.109000e+07 & 1.593000e+04 & 3.030000e+04 & 0.999245 &
    3.996074\\
    bcsstk07 & 420 & 2.109000e+07 & 1.593000e+04 & 3.030000e+04 & 0.999245 &
    4.016814\\
    bcsstk22 & 138 & 6.194000e+07 & 5.012000e+05 & 7.312000e+05 & 0.991909 &
    0.381385\\
    bcsstm01 & 48 & 7.782000e+07 & 1.000000e+00 & 1.000000e+00 & 1.000000 &
    0.105460\\
    bcsstm02 & 66 & 7.660000e+01 & 1.000000e+00 & 1.000000e+00 & 0.986945 &
    0.106136\\
    bcsstm03 & 112 & 5.569000e+07 & 1.000000e+00 & 1.000000e+00 & 1.000000 &
    0.176999\\
    bcsstm04 & 132 & 2.987000e+04 & 1.000000e+00 & 1.000000e+00 & 0.999967 &
    0.134561\\
    bcsstm05 & 153 & 1.612000e+02 & 1.000000e+00 & 1.000000e+00 & 0.993798 &
    0.158579\\
    bcsstm06 & 420 & 5.512000e+07 & 1.000000e+00 & 1.000000e+00 & 1.000000 &
    0.721068\\
    bcsstm07 & 420 & 4.456000e+07 & 4.136000e+04 & 7.454000e+04 & 0.999072 &
    4.501864\\
    bcsstm22 & 138 & 8.860000e+05 & 1.000000e+00 & 1.000000e+00 & 0.999999 &
    0.148473\\
    can\_144 & 144 & 2.443000e+07 & 2.256000e+07 & 2.255000e+07 & 0.076367 &
    0.309114\\
    can\_161 & 161 & 4.940000e+04 & 3.960000e+04 & 4.615000e+04 & 0.198256 &
    0.440638\\
    can\_187 & 187 & 7.056000e+07 & 3.191000e+07 & 6.229000e+07 & 0.547706 &
    0.558273\\
    can\_229 & 229 & 1.891000e+07 & 1.604000e+07 & 1.929000e+07 & 0.151527 &
    0.606216\\
    can\_24 & 24 & 6.046000e+03 & 4.025000e+03 & 4.900000e+03 & 0.334338 &
    0.127885\\
    can\_256 & 256 & 7.565000e+06 & 3.686000e+06 & 6.533000e+06 & 0.512763 &
    4.624222\\
    can\_268 & 268 & 2.091000e+07 & 8.414000e+06 & 1.676000e+07 & 0.597536 &
    1.479174\\
    can\_292 & 292 & 3.699000e+07 & 2.342000e+07 & 1.324000e+08 & 0.366954 &
    1.222109\\
    can\_445 & 445 & 4.006000e+07 & 1.346000e+07 & 3.943000e+07 & 0.663895 &
    2.818335\\
    can\_61 & 61 & 2.996000e+07 & 1.355000e+07 & 2.925000e+07 & 0.547665 &
    0.163705\\
    can\_62 & 62 & 3.646000e+05 & 2.100000e+05 & 3.135000e+05 & 0.423995 &
    0.164177\\
    can\_73 & 73 & 1.270000e+03 & 1.053000e+03 & 1.228000e+03 & 0.170424 &
    0.191222\\
    can\_96 & 96 & 2.104000e+04 & 1.733000e+04 & 1.971000e+04 & 0.176483 &
    0.198430\\
    curtis54 & 54 & 4.522000e+07 & 1.366000e+07 & 3.878000e+07 & 0.697928 &
    0.146304\\
    dwt\_162 & 162 & 2.204000e+07 & 1.579000e+07 & 3.449000e+07 & 0.283632 &
    0.334807\\
    dwt\_193 & 193 & 1.310000e+07 & 1.037000e+07 & 1.513000e+07 & 0.208211 &
    0.597751\\
    dwt\_198 & 198 & 3.397000e+07 & 1.963000e+07 & 3.034000e+07 & 0.422230 &
    0.408961\\
    dwt\_209 & 209 & 5.449000e+07 & 9.330000e+06 & 3.408000e+07 & 0.828784 &
    0.795283\\
    \hline
  \end{tabular}
  \caption{\texttt{SuiteSparse} Dataset}
\end{table}

\begin{table}[H]
\centering
  \begin{tabular}{c|c|c|c|cc|c}
    \hline
    Mat & Size & Cbef & Caft & Cdiag & Reduce & Time\\
    \hline
    dwt\_221 & 221 & 3.381000e+07 & 1.101000e+07 & 5.672000e+07 & 0.674357 &
    0.675951\\
    dwt\_234 & 234 & 1.042000e+05 & 4.006000e+04 & 8.153000e+04 & 0.615561 &
    0.675201\\
    dwt\_245 & 245 & 3.634000e+07 & 1.218000e+07 & 3.336000e+07 & 0.664825 &
    0.766070\\
    dwt\_307 & 307 & 2.499000e+07 & 2.276000e+07 & 2.565000e+07 & 0.089230 &
    1.154597\\
    dwt\_310 & 310 & 1.069000e+07 & 5.251000e+06 & 9.304000e+06 & 0.508690 &
    1.361014\\
    dwt\_346 & 346 & 4.967000e+07 & 4.011000e+06 & 2.357000e+07 & 0.919252 &
    1.532717\\
    dwt\_361 & 361 & 3.879000e+07 & 2.166000e+07 & 3.706000e+07 & 0.441465 &
    1.496653\\
    dwt\_419 & 419 & 2.180000e+07 & 1.431000e+07 & 2.549000e+07 & 0.343696 &
    1.682823\\
    dwt\_492 & 492 & 3.047000e+07 & 1.301000e+07 & 2.418000e+07 & 0.572926 &
    2.487955\\
    dwt\_59 & 59 & 1.395000e+04 & 8.580000e+03 & 1.226000e+04 & 0.384885 &
    0.157282\\
    dwt\_66 & 66 & 2.234000e+04 & 1.530000e+04 & 2.160000e+04 & 0.314936 &
    0.146260\\
    dwt\_72 & 72 & 1.220000e+07 & 5.763000e+06 & 9.623000e+06 & 0.527499 &
    0.149897\\
    dwt\_87 & 87 & 1.024000e+04 & 5.077000e+03 & 8.223000e+03 & 0.504366 &
    0.218176\\
    gent113 & 113 & 3.203000e+07 & 8.757000e+06 & 1.758000e+07 & 0.726609 &
    0.259552\\
    gre\_115 & 115 & 2.467000e+03 & 1.835000e+03 & 2.332000e+03 & 0.256268 &
    0.278696\\
    gre\_185 & 185 & 1.230000e+06 & 9.805000e+05 & 1.313000e+06 & 0.202757 &
    0.684197\\
    gre\_216a & 216 & 1.061000e+04 & 9.002000e+03 & 1.145000e+04 & 0.151722 &
    0.655149\\
    gre\_343 & 343 & 1.254000e+04 & 9.442000e+03 & 1.288000e+04 & 0.246972 &
    1.478083\\
    hor\_131 & 434 & 4.365000e+05 & 8.362000e+04 & 3.197000e+05 & 0.808423 &
    3.846565\\
    ibm32 & 32 & 1.633000e+05 & 8.383000e+04 & 1.248000e+05 & 0.486670 &
    0.131650\\
    illc1033 & 320 & 4.540000e+06 & 2.175000e+06 & 4.540000e+06 & 0.520966 &
    1.358549\\
    impcol\_a & 207 & 2.233000e+07 & 1.613000e+07 & 1.202000e+07 & 0.277622 &
    0.395068\\
    impcol\_b & 59 & 3.727000e+07 & 1.754000e+06 & 4.031000e+06 & 0.952948 &
    0.167633\\
    impcol\_c & 137 & 4.736000e+07 & 3.128000e+04 & 6.180000e+04 & 0.999339 &
    0.326395\\
    impcol\_d & 425 & 4.250000e+06 & 4.157000e+05 & 8.524000e+05 & 0.902187 &
    2.347745\\
    impcol\_e & 225 & 2.384000e+07 & 2.028000e+01 & 2.922000e+01 & 0.999999 &
    0.997038\\
    jgl009 & 9 & 3.723000e+07 & 2.892000e+07 & 3.786000e+07 & 0.223225 &
    0.089136\\
    lshp\_265 & 265 & 1.927000e+06 & 1.145000e+06 & 1.804000e+06 & 0.405525 &
    1.256791\\
    lshp\_406 & 406 & 1.230000e+06 & 9.028000e+05 & 1.148000e+06 & 0.265790 &
    2.063599\\
    lund\_b & 147 & 4.977000e+07 & 9.277000e+04 & 1.431000e+05 & 0.998136 &
    0.775601\\
    mbeacxc & 496 & 2.857000e+06 & 2.172000e+06 & 1.894000e+07 & 0.239616 &
    5.161266\\
    mbeaflw & 496 & 5.820000e+06 & 1.068000e+05 & 3.381000e+06 & 0.981656 &
    8.130244\\
    mbeause & 496 & 7.052000e+06 & 1.249000e+05 & 4.015000e+06 & 0.982292 &
    8.919944\\
    nnc261 & 261 & 1.652000e+07 & 3.333000e+06 & 5.758000e+06 & 0.798272 &
    1.181010\\
    nos4 & 100 & 2.492000e+06 & 1.096000e+06 & 1.136000e+06 & 0.559997 &
    0.230104\\
    nos5 & 468 & 2.975000e+07 & 1.447000e+06 & 1.555000e+06 & 0.951367 &
    7.251103\\
    plat362 & 362 & 5.995000e+05 & 5.944000e+05 & 7.967000e+05 & 0.008550 &
    1.877958\\
    plskz362 & 362 & 7.743000e+05 & 6.933000e+05 & 8.058000e+05 & 0.104524 &
    1.290407\\
    pores\_1 & 30 & 2.774000e+07 & 4.481000e+06 & 7.514000e+06 & 0.838435 &
    0.128902\\
    str\_0 & 363 & 7.511000e+04 & 1.470000e+04 & 4.686000e+03 & 0.804285 &
    0.788147\\
    str\_200 & 363 & 1.371000e+07 & 4.065000e+05 & 7.715000e+05 & 0.970347 &
    2.368018\\
    str\_400 & 363 & 1.912000e+07 & 5.322000e+06 & 1.067000e+06 & 0.721693 &
    0.836974\\
    str\_600 & 363 & 1.184000e+07 & 4.537000e+05 & 1.212000e+06 & 0.961681 &
    2.305290\\
    west0067 & 67 & 1.696000e+04 & 5.903000e+03 & 7.326000e+03 & 0.651885 &
    0.160354\\
    west0132 & 132 & 4.772000e+07 & 4.199000e+02 & 7.208000e+02 & 0.999991 &
    0.278596\\
    west0167 & 167 & 4.772000e+07 & 8.476000e+02 & 1.147000e+03 & 0.999982 &
    0.396684\\
    west0381 & 381 & 2.245000e+07 & 2.068000e+02 & 4.687000e+02 & 0.999991 &
    3.711164\\
    west0479 & 479 & 4.737000e+07 & 1.252000e+03 & 2.064000e+03 & 0.999974 &
    2.245246\\
    west0497 & 497 & 5.540000e+07 & 2.286000e+03 & 4.163000e+03 & 0.999959 &
    2.031159\\
    will199 & 199 & 1.926000e+07 & 1.085000e+07 & 1.553000e+07 & 0.436279 &
    0.502647\\
    will57 & 57 & 3.781000e+07 & 2.533000e+07 & 6.034000e+07 & 0.330104 &
    0.141474\\
    wm1 & 277 & 2.135000e+07 & 7.922000e+03 & 6.662000e+04 & 0.999629 &
    2.268211\\
    wm2 & 260 & 1.244000e+07 & 8.332000e+05 & 5.324000e+06 & 0.933019 &
    1.470060\\
    wm3 & 260 & 9.514000e+06 & 9.065000e+05 & 1.103000e+07 & 0.904718 &
    1.571223\\
    \hline
  \end{tabular}
  \caption{\texttt{SuiteSparse} Dataset}
\end{table}

\begin{table}[H]
\centering
  \begin{tabular}{ccccccc}
    \hline
    Mat & Size & Cbef & Caft & Cdiag & Reduce & Time\\
    \hline
    bfwa398 & 398 & 8.959000e+06 & 1.682000e+06 & 1.791000e+06 & 0.812196 &
    3.615892\\
    bfwa62 & 62 & 3.059000e+05 & 5.152000e+04 & 5.508000e+04 & 0.831580 &
    0.174470\\
    bfwb398 & 398 & 4.465000e+02 & 1.565000e+02 & 2.912000e+01 & 0.649453 &
    3.353016\\
    bfwb62 & 62 & 2.958000e+02 & 2.676000e+01 & 2.729000e+01 & 0.909552 &
    0.246814\\
    bwm200 & 200 & 5.820000e+06 & 3.290000e+06 & 3.292000e+06 & 0.434761 &
    0.546737\\
    ck104 & 104 & 2.987000e+07 & 1.143000e+06 & 1.406000e+06 & 0.961728 &
    0.203493\\
    ck400 & 400 & 3.284000e+07 & 1.001000e+06 & 1.210000e+06 & 0.969527 &
    1.006684\\
    lop163 & 163 & 1.281000e+06 & 5.703000e+05 & 7.108000e+05 & 0.554680 &
    0.470454\\
    mhda416 & 416 & 2.466000e+07 & 3.819000e+05 & 1.990000e+06 & 0.984513 &
    3.291940\\
    olm100 & 100 & 4.480000e+07 & 3.092000e+07 & 5.322000e+07 & 0.309857 &
    0.243572\\
    olm500 & 500 & 3.185000e+07 & 3.146000e+07 & 6.098000e+07 & 0.012234 &
    2.274321\\
    pde225 & 225 & 1.526000e+03 & 9.913000e+02 & 1.009000e+03 & 0.350364 &
    1.132055\\
    rbsa480 & 480 & 5.333000e+06 & 7.129000e+05 & 1.213000e+06 & 0.866327 &
    9.633158\\
    rbsb480 & 480 & 1.038000e+07 & 2.140000e+06 & 3.135000e+06 & 0.793806 &
    9.278184\\
    rw136 & 136 & 1.302000e+06 & 5.420000e+05 & 8.482000e+05 & 0.583550 &
    0.342707\\
    rw496 & 496 & 1.315000e+06 & 8.306000e+05 & 1.325000e+06 & 0.368444 &
    3.604414\\
    tub100 & 100 & 4.427000e+07 & 4.254000e+07 & 4.311000e+07 & 0.039051 &
    0.226566\\
    cavity01 & 317 & 3.947000e+07 & 6.467000e+04 & 1.104000e+05 & 0.998361 &
    2.054133\\
    cavity02 & 317 & 1.823000e+07 & 3.743000e+04 & 6.269000e+04 & 0.997946 &
    1.405985\\
    mhdb416 & 416 & 4.824000e+06 & 5.071000e+01 & 6.303000e+01 & 0.999989 &
    1.188644\\
    odepa400 & 400 & 2.504000e+07 & 1.593000e+07 & 1.601000e+07 & 0.363637 &
    0.933260\\
    odepb400 & 400 & 1.000000e+00 & 1.000000e+00 & 1.000000e+00 & 0.000000 &
    0.330884\\
    cavity03 & 317 & 1.709000e+07 & 5.320000e+04 & 1.010000e+05 & 0.996887 &
    2.020333\\
    cavity04 & 317 & 1.966000e+07 & 9.305000e+04 & 1.743000e+05 & 0.995268 &
    1.563758\\
    ex1 & 216 & 1.695000e+04 & 7.532000e+01 & 8.818000e+01 & 0.995556 &
    0.926692\\
    ex5 & 27 & 3.457000e+07 & 3.443000e+07 & 7.392000e+07 & 0.004130 &
    0.102971\\
    b1\_ss & 7 & 3.896000e+04 & 7.115000e+01 & 7.581000e+01 & 0.998174 &
    0.107598\\
    d\_dyn & 87 & 4.941000e+07 & 2.718000e+07 & 5.370000e+07 & 0.449806 &
    0.154185\\
    d\_dyn1 & 87 & 3.799000e+07 & 2.324000e+07 & 4.598000e+07 & 0.388401 &
    0.212365\\
    d\_ss & 53 & 7.596000e+07 & 3.611000e+07 & 3.591000e+07 & 0.524657 &
    0.174045\\
    lp\_adlittle & 138 & 2.077000e+07 & 1.976000e+07 & 5.740000e+07 & 0.048207
    & 0.248500\\
    lp\_afiro & 51 & 2.299000e+07 & 1.711000e+07 & 2.240000e+07 & 0.255975 &
    0.129797\\
    lp\_bandm & 472 & 1.055000e+07 & 4.584000e+06 & 1.481000e+07 & 0.565650 &
    3.579121\\
    lp\_beaconfd & 295 & 8.045000e+06 & 5.414000e+06 & 3.167000e+07 & 0.327030
    & 2.481520\\
    lp\_blend & 114 & 1.085000e+07 & 2.700000e+06 & 4.689000e+06 & 0.751234 &
    0.229854\\
    lp\_bore3d & 334 & 5.691000e+06 & 1.693000e+06 & 1.527000e+07 & 0.702497 &
    1.908079\\
    lp\_brandy & 303 & 1.268000e+07 & 2.525000e+06 & 9.341000e+06 & 0.800858 &
    2.202008\\
    lp\_capri & 482 & 1.781000e+07 & 3.544000e+06 & 9.499000e+06 & 0.801002 &
    2.749435\\
    lp\_e226 & 472 & 7.518000e+06 & 2.876000e+06 & 7.345000e+07 & 0.617431 &
    5.803117\\
    lp\_israel & 316 & 2.213000e+07 & 1.540000e+07 & 8.211000e+07 & 0.303837 &
    1.090616\\
    lp\_kb2 & 68 & 2.378000e+07 & 1.584000e+07 & 3.134000e+07 & 0.333936 &
    0.396778\\
    lp\_lotfi & 366 & 3.101000e+06 & 1.475000e+06 & 2.984000e+07 & 0.524448 &
    3.473910\\
    lp\_recipe & 204 & 2.359000e+07 & 9.999000e+06 & 9.718000e+06 & 0.576179 &
    0.563452\\
    lp\_sc105 & 163 & 1.681000e+07 & 1.418000e+07 & 1.942000e+07 & 0.155977 &
    0.320327\\
    lp\_sc205 & 317 & 1.682000e+07 & 1.424000e+07 & 1.949000e+07 & 0.153231 &
    0.804767\\
    lp\_sc50a & 78 & 1.676000e+07 & 1.390000e+07 & 1.908000e+07 & 0.170654 &
    0.150149\\
    lp\_sc50b & 78 & 1.505000e+07 & 1.227000e+07 & 1.694000e+07 & 0.184765 &
    0.148078\\
    lp\_scagr7 & 185 & 1.053000e+07 & 1.761000e+06 & 2.693000e+06 & 0.832777 &
    0.393990\\
    lp\_scorpion & 466 & 7.188000e+06 & 5.136000e+06 & 8.973000e+06 & 0.285497
    & 1.739667\\
    lp\_share1b & 253 & 1.991000e+07 & 1.298000e+07 & 1.077000e+08 & 0.348287
    & 1.026345\\
    lp\_share2b & 162 & 2.101000e+07 & 1.321000e+07 & 2.775000e+07 & 0.371176
    & 0.472567\\
    lp\_stocfor1 & 165 & 1.460000e+07 & 9.642000e+06 & 2.154000e+07 & 0.339626
    & 0.431685\\
    lp\_vtp\_base & 346 & 2.890000e+07 & 6.588000e+04 & 5.285000e+05 &
    0.997720 & 2.345079\\
    lpi\_bgprtr & 40 & 2.497000e+07 & 6.505000e+05 & 1.091000e+06 & 0.973943 &
    0.147450\\
    \hline
  \end{tabular}
  \caption{\texttt{SuiteSparse} Dataset}
\end{table}

\begin{table}[H]
\centering
  \begin{tabular}{ccccccc}
    \hline
    Mat & Size & Cbef & Caft & Cdiag & Reduce & Time\\
    \hline
    lpi\_box1 & 261 & 3.616000e+07 & 2.108000e+07 & 4.128000e+07 & 0.416908 &
    0.692226\\
    lpi\_cplex2 & 378 & 1.344000e+07 & 8.448000e+06 & 1.189000e+07 & 0.371548
    & 1.543225\\
    lpi\_ex72a & 215 & 8.578000e+06 & 5.964000e+06 & 9.181000e+06 & 0.304744 &
    0.449019\\
    lpi\_ex73a & 211 & 8.578000e+06 & 5.968000e+06 & 8.855000e+06 & 0.304278 &
    0.398350\\
    lpi\_forest6 & 131 & 7.137000e+06 & 7.003000e+06 & 8.160000e+06 & 0.018793
    & 0.217445\\
    lpi\_galenet & 14 & 5.895000e+06 & 5.324000e+06 & 6.323000e+06 & 0.096880
    & 0.107415\\
    lpi\_itest2 & 13 & 1.786000e+07 & 5.946000e+06 & 6.415000e+06 & 0.667043 &
    0.109737\\
    lpi\_itest6 & 17 & 1.124000e+07 & 6.547000e+06 & 7.369000e+06 & 0.417575 &
    0.115537\\
    lpi\_klein1 & 108 & 1.431000e+07 & 2.869000e+06 & 5.145000e+06 & 0.799539
    & 0.444161\\
    lpi\_qual & 464 & 2.440000e+07 & 1.233000e+05 & 4.093000e+05 & 0.994946 &
    2.865512\\
    lpi\_refinery & 464 & 2.440000e+07 & 1.154000e+05 & 3.669000e+05 &
    0.995271 & 2.687036\\
    lpi\_vol1 & 464 & 2.440000e+07 & 1.233000e+05 & 4.093000e+05 & 0.994946 &
    2.806833\\
    lpi\_woodinfe & 89 & 8.685000e+06 & 8.619000e+06 & 1.008000e+07 & 0.007664
    & 0.156514\\
    lp\_nug05 & 225 & 9.453000e+06 & 9.445000e+06 & 1.167000e+07 & 0.000832 &
    0.484108\\
    lp\_nug06 & 486 & 5.863000e+06 & 5.862000e+06 & 8.000000e+06 & 0.000082 &
    2.855134\\
    utm300 & 300 & 5.520000e+06 & 2.591000e+06 & 5.520000e+06 & 0.530525 &
    1.371771\\
    pivtol & 102 & 1.201000e+04 & 6.731000e+02 & 6.756000e+02 & 0.943974 &
    0.181140\\
    mesh1e1 & 48 & 2.756000e+01 & 1.500000e+01 & 1.832000e+01 & 0.455693 &
    0.141812\\
    mesh1em1 & 48 & 3.609000e+02 & 1.553000e+02 & 1.634000e+02 & 0.569767 &
    0.187848\\
    mesh1em6 & 48 & 3.731000e+01 & 2.348000e+01 & 2.422000e+01 & 0.370796 &
    0.149999\\
    mesh2e1 & 306 & 8.431000e+04 & 1.934000e+04 & 2.331000e+04 & 0.770582 &
    1.767308\\
    mesh2em5 & 306 & 6.085000e+04 & 2.221000e+04 & 2.448000e+04 & 0.635019 &
    2.033301\\
    mesh3e1 & 289 & 7.970000e+01 & 7.367000e+01 & 7.371000e+01 & 0.075652 &
    0.948502\\
    mesh3em5 & 289 & 2.466000e+01 & 2.383000e+01 & 2.384000e+01 & 0.033547 &
    0.649657\\
    sphere2 & 66 & 4.729000e+07 & 2.100000e+07 & 4.810000e+07 & 0.555919 &
    0.143261\\
    sphere3 & 258 & 2.431000e+07 & 2.246000e+07 & 2.439000e+07 & 0.075870 &
    0.741558\\
    cage3 & 5 & 3.552000e+02 & 2.324000e+02 & 2.826000e+02 & 0.345737 &
    0.090801\\
    cage4 & 9 & 3.749000e+02 & 2.332000e+02 & 2.662000e+02 & 0.378129 &
    0.092323\\
    cage5 & 37 & 2.377000e+02 & 1.446000e+02 & 1.623000e+02 & 0.391509 &
    0.142229\\
    cage6 & 93 & 1.305000e+02 & 5.598000e+01 & 6.216000e+01 & 0.571133 &
    0.275322\\
    cage7 & 340 & 1.709000e+02 & 7.342000e+01 & 9.425000e+01 & 0.570302 &
    2.882972\\
    problem1 & 415 & 4.188000e+07 & 2.802000e+07 & 3.407000e+07 & 0.330968 &
    1.394374\\
    oscil\_trans\_01 & 430 & 5.827000e+07 & 5.562000e+07 & 7.219000e+07 &
    0.045355 & 0.800879\\
    Harvard500 & 500 & 1.830000e+07 & 1.673000e+07 & 9.449000e+07 & 0.085593 &
    3.517279\\
    lap\_25 & 25 & 2.786000e+07 & 2.436000e+07 & 2.985000e+07 & 0.125389 &
    0.108474\\
    rajat05 & 301 & 1.466000e+07 & 1.316000e+06 & 5.248000e+06 & 0.910252 &
    0.894197\\
    rajat11 & 135 & 7.500000e+07 & 9.077000e+05 & 3.267000e+06 & 0.987897 &
    0.284779\\
    rajat14 & 180 & 5.543000e+07 & 1.563000e+06 & 7.485000e+06 & 0.971808 &
    1.454099\\
    Hamrle1 & 32 & 4.796000e+07 & 3.333000e+05 & 5.875000e+05 & 0.993051 &
    0.134966\\
    robot & 120 & 4.407000e+07 & 1.020000e+04 & 1.204000e+04 & 0.999769 &
    0.335016\\
    rotor1 & 100 & 3.726000e+07 & 1.869000e+06 & 2.374000e+06 & 0.949828 &
    0.305103\\
    LF10 & 18 & 5.170000e+07 & 4.958000e+04 & 6.238000e+04 & 0.999041 &
    0.135056\\
    Cities & 46 & 4.291000e+04 & 1.275000e+04 & 1.996000e+04 & 0.702834 &
    0.121651\\
    divorce & 9 & 3.760000e+02 & 1.794000e+02 & 4.251000e+02 & 0.522869 &
    0.093020\\
    \hline
  \end{tabular}
  \caption{\texttt{SuiteSparse} Dataset}
\end{table}

\begin{table}[H]
\centering
  \begin{tabular}{ccccc}
    \hline
    Mat & Size & Cbef & Caft & Reduce\\
    \hline
    YearPredictionMSD & 90 & 5233000.00 & 470.20 & 0.999910\\
    YearPredictionMSD.t & 90 & 5521000.00 & 359900.00 & 0.934816\\
    abalone\_scale.txt & 8 & 2419.00 & 2038.00 & 0.157291\\
    bodyfat\_scale.txt & 14 & 1281.00 & 669.10 & 0.477475\\
    cadata.txt & 8 & 8982000.00 & 7632.00 & 0.999150\\
    cpusmall\_scale.txt & 12 & 20000.00 & 6325.00 & 0.683813\\
    eunite2001.t & 16 & 52450000.00 & 8530.00 & 0.999837\\
    eunite2001.txt & 16 & 67300000.00 & 3591.00 & 0.999947\\
    housing\_scale.txt & 13 & 153.90 & 83.22 & 0.459371\\
    mg\_scale.txt & 6 & 10.67 & 10.03 & 0.059988\\
    mpg\_scale.txt & 7 & 142.50 & 107.20 & 0.247842\\
    pyrim\_scale.txt & 27 & 49100000.00 & 3307.00 & 0.999933\\
    space\_ga\_scale.txt & 6 & 1061.00 & 729.60 & 0.312041\\
    triazines\_scale.txt & 60 & 24580000.00 & 15460000.00 & 0.371034\\
    \hline
  \end{tabular}
  \caption{\texttt{LIBSVM} Dataset (Time statistic is ignored, all less
  than 0.1 second)}
\end{table}
