# Supplementary material for: Optimal Diagonal Preconditioning
Source: arXiv:2209.00809 source file (2022-11-04)
Supplement: Supplementary file 3 [file appendix_left_precond_res.tex]

\section{Detailed Experiment Results for Left Preconditioning}
\label{app:left}
\begin{table}[H]
\centering
  \begin{tabular}{ccccc}
    \hline
    Mat & Cbef & Caft & Rdc & Time\\
    \hline
    ash219 & 9.150000e+00 & 4.580000e+00 & 0.499389 & 0.487467\\
    ash331 & 9.588000e+00 & 3.618000e+00 & 0.622636 & 0.730943\\
    ash608 & 1.138000e+01 & 3.789000e+00 & 0.666922 & 2.025805\\
    ash85 & 2.151000e+05 & 1.283000e+05 & 0.403496 & 0.204215\\
    ash958 & 1.025000e+01 & 3.702000e+00 & 0.638750 & 3.816961\\
    bcspwr01 & 2.756000e+03 & 1.676000e+03 & 0.391882 & 0.129029\\
    bcspwr03 & 2.514000e+05 & 1.137000e+05 & 0.547642 & 0.253503\\
    bcsstk02 & 1.871000e+07 & 2.973000e+06 & 0.841082 & 0.864357\\
    bcsstm02 & 7.660000e+01 & 1.000000e+00 & 0.986945 & 0.108913\\
    bcsstm05 & 1.612000e+02 & 1.000000e+00 & 0.993798 & 0.148165\\
    bcsstm07 & 5.799000e+07 & 4.737000e+04 & 0.999183 & 4.507644\\
    bcsstm22 & 8.860000e+05 & 8.336000e+02 & 0.999059 & 0.175163\\
    can\_161 & 4.940000e+04 & 3.960000e+04 & 0.198256 & 0.413971\\
    can\_24 & 6.046000e+03 & 4.025000e+03 & 0.334338 & 0.132879\\
    can\_62 & 3.646000e+05 & 2.100000e+05 & 0.423995 & 0.156431\\
    can\_73 & 1.270000e+03 & 1.053000e+03 & 0.170424 & 0.180774\\
    can\_96 & 2.104000e+04 & 1.733000e+04 & 0.176483 & 0.209492\\
    dwt\_234 & 1.042000e+05 & 4.006000e+04 & 0.615561 & 0.595150\\
    dwt\_310 & 1.069000e+07 & 5.251000e+06 & 0.508682 & 1.314032\\
    dwt\_59 & 1.395000e+04 & 8.580000e+03 & 0.384885 & 0.164891\\
    dwt\_66 & 2.234000e+04 & 1.530000e+04 & 0.314936 & 0.182006\\
    dwt\_87 & 1.024000e+04 & 5.077000e+03 & 0.504366 & 0.207312\\
    gre\_115 & 2.467000e+03 & 9.975000e+02 & 0.595714 & 0.236888\\
    gre\_216a & 1.061000e+04 & 7.721000e+03 & 0.272449 & 0.617148\\
    gre\_343 & 1.254000e+04 & 9.115000e+03 & 0.273061 & 1.331253\\
    ibm32 & 1.633000e+05 & 1.052000e+05 & 0.355548 & 0.131495\\
    impcol\_d & 4.250000e+06 & 2.025000e+05 & 0.952340 & 1.603679\\
    lshp\_265 & 1.927000e+06 & 1.145000e+06 & 0.405524 & 1.129425\\
    lshp\_406 & 1.230000e+06 & 9.028000e+05 & 0.265790 & 2.036749\\
    nos4 & 2.492000e+06 & 1.096000e+06 & 0.559996 & 0.285999\\
    str\_0 & 7.511000e+04 & 3.707000e+03 & 0.950651 & 2.102136\\
    str\_400 & 4.135000e+07 & 5.383000e+05 & 0.986983 & 2.211820\\
    west0067 & 1.696000e+04 & 3.618000e+03 & 0.786653 & 0.185835\\
    bfwa398 & 8.959000e+06 & 1.552000e+06 & 0.826792 & 1.788203\\
    bfwa62 & 3.059000e+05 & 4.735000e+04 & 0.845202 & 0.185078\\
    bfwb398 & 4.465000e+02 & 2.887000e+01 & 0.935330 & 1.681382\\
    bfwb62 & 2.958000e+02 & 2.676000e+01 & 0.909552 & 0.170433\\
    bwm200 & 5.820000e+06 & 4.045000e+06 & 0.304993 & 0.478939\\
    ck104 & 2.987000e+07 & 1.103000e+07 & 0.630594 & 0.285076\\
    pde225 & 1.526000e+03 & 1.056000e+03 & 0.308166 & 0.551753\\
    b1\_ss & 3.896000e+04 & 2.977000e+04 & 0.235744 & 0.117189\\
    pivtol & 1.201000e+04 & 1.045000e+01 & 0.999130 & 0.185078\\
    mesh1e1 & 2.756000e+01 & 1.500000e+01 & 0.455693 & 0.148006\\
    mesh1em1 & 3.609000e+02 & 1.553000e+02 & 0.569767 & 0.187894\\
    mesh1em6 & 3.731000e+01 & 2.348000e+01 & 0.370796 & 0.148615\\
    cage4 & 3.749000e+02 & 7.511000e+01 & 0.799676 & 0.095057\\
    cage5 & 2.377000e+02 & 3.664000e+01 & 0.845852 & 0.155320\\
    cage6 & 1.305000e+02 & 2.312000e+01 & 0.822845 & 0.292317\\
    cage7 & 1.709000e+02 & 2.372000e+01 & 0.861186 & 2.630823\\
    poisson2D & 1.762000e+04 & 1.298000e+04 & 0.263418 & 1.461464\\
    Cities & 4.291000e+04 & 2.032000e+04 & 0.526343 & 0.461808\\
    GD95\_c & 2.651000e+03 & 1.357000e+03 & 0.488034 & 0.157926\\
    \hline
  \end{tabular}
  \caption{\texttt{SuiteSparse} Datset}
\end{table}

\begin{table}[H]
\centering
  \begin{tabular}{ccccc}
    \hline
    Mat & Cbef & Caft & Rdc & Time\\
    \hline
    Journals & 9.629000e+07 & 2.666000e+02 & 0.999997 & 4.078209\\
    Stranke94 & 2.676000e+03 & 2.339000e+03 & 0.125982 & 0.098082\\
    Tina\_AskCog & 3.914000e+02 & 2.897000e+02 & 0.259784 & 0.100079\\
    rdb200 & 1.191000e+05 & 4.472000e+04 & 0.624532 & 0.642029\\
    rdb200l & 1.760000e+04 & 9.535000e+03 & 0.458098 & 0.650536\\
    rdb450 & 4.695000e+05 & 1.842000e+05 & 0.607593 & 2.102066\\
    rdb450l & 4.395000e+04 & 1.820000e+04 & 0.585936 & 2.126565\\
    CAG\_mat72 & 7.720000e+07 & 1.707000e+07 & 0.778920 & 0.316561\\
    08blocks & 2.749000e+07 & 7.380000e+02 & 0.999973 & 0.454232\\
    Trefethen\_20b & 9.212000e+02 & 8.697000e+00 & 0.990559 & 0.150969\\
    Trefethen\_20 & 3.980000e+03 & 2.859000e+01 & 0.992817 & 0.165166\\
    Trefethen\_150 & 5.928000e+05 & 3.893000e+01 & 0.999934 & 0.581308\\
    Trefethen\_200b & 2.723000e+05 & 1.102000e+01 & 0.999960 & 0.905146\\
    Trefethen\_200 & 1.190000e+06 & 3.893000e+01 & 0.999967 & 0.843932\\
    Trefethen\_300 & 3.142000e+06 & 4.213000e+01 & 0.999987 & 1.942225\\
    Trefethen\_500 & 1.015000e+07 & 4.213000e+01 & 0.999996 & 6.035735\\
    polbooks & 5.187000e+05 & 1.738000e+05 & 0.664881 & 0.329573\\
    jazz & 9.052000e+06 & 4.180000e+06 & 0.538207 & 3.676270\\
    cz148 & 6.113000e+06 & 6.738000e+05 & 0.889768 & 0.485724\\
    mycielskian2 & 1.000000e+00 & 1.000000e+00 & 0.000000 & 0.087618\\
    mycielskian4 & 9.391000e+01 & 8.476000e+01 & 0.097455 & 0.093933\\
    mycielskian5 & 7.641000e+02 & 6.110000e+02 & 0.200423 & 0.140891\\
    mycielskian6 & 5.863000e+03 & 4.139000e+03 & 0.293979 & 0.198246\\
    mycielskian7 & 4.337000e+04 & 2.700000e+04 & 0.377367 & 0.419387\\
    mycielskian8 & 3.132000e+05 & 1.717000e+05 & 0.451873 & 1.543068\\
    mycielskian9 & 2.227000e+06 & 1.072000e+06 & 0.518613 & 15.107065\\
    breasttissue & 4.147000e+05 & 4.605000e+04 & 0.888958 & 0.439709\\
    dermatology & 8.770000e+06 & 9.132000e+05 & 0.895866 & 1.544294\\
    Ecoli\_10NN & 9.637000e+07 & 9.046000e+06 & 0.906131 & 2.456245\\
    iris\_dataset & 4.617000e+05 & 2.363000e+05 & 0.488167 & 3.225024\\
    Olivetti\_norm & 3.756000e+06 & 3.668000e+05 & 0.902332 & 5.556022\\
    YaleA\_10NN & 7.517000e+07 & 4.723000e+06 & 0.937167 & 0.911497\\
    mesh2e1 & 8.431000e+04 & 1.934000e+04 & 0.770583 & 1.267981\\
    mesh2em5 & 6.085000e+04 & 2.221000e+04 & 0.635020 & 1.188451\\
    mesh3e1 & 7.970000e+01 & 7.367000e+01 & 0.075652 & 0.685717\\
    mesh3em5 & 2.466000e+01 & 2.383000e+01 & 0.033547 & 0.713168\\
    \hline
  \end{tabular}
  \caption{\texttt{SuiteSparse} Datset}
\end{table}
