# Supplementary material for: Optimal Diagonal Preconditioning
Source: arXiv:2209.00809 source file (2022-11-04)
Supplement: Supplementary file 4 [file appendix_two_sided_precond_res.tex]

\section{Detailed Experiment Results for Two-sided Preconditioning}
\label{app:two-sided}
\begin{table}[H]
\centering
  \begin{tabular}{cccccc}
  \hline
  Mat & cBef & cAft & cRuiz & Reduce & Best One-sided\\
  \hline
  ash85 & 2.151e+05 & 8.596e+04 & 2.151e+05 & 6.003e-01 & 1.283e+05\\
  
  bcspwr01 & 2.756e+03 & 1.268e+03 & 2.756e+03 & 5.399e-01 & 2.164e+03\\
  
  bcsstk02 & 1.871e+07 & 2.634e+06 & 3.284e+06 & 8.592e-01 & 2.973e+06\\
  
  bcsstm02 & 7.660e+01 & 1.000e+00 & 1.000e+00 & 9.869e-01 & 1.000e+00\\
  
  can\_24 & 6.046e+03 & 3.329e+03 & 6.046e+03 & 4.495e-01 & 4.025e+03\\
  
  can\_62 & 3.646e+05 & 1.371e+05 & 3.646e+05 & 6.241e-01 & 2.100e+05\\
  
  can\_73 & 1.270e+03 & 8.363e+02 & 1.270e+03 & 3.414e-01 & 1.053e+03\\
  
  can\_96 & 2.104e+04 & 1.602e+04 & 2.104e+04 & 2.386e-01 & 1.733e+04\\
  
  dwt\_59 & 1.395e+04 & 6.595e+03 & 1.395e+04 & 5.272e-01 & 8.580e+03\\
  
  dwt\_66 & 2.234e+04 & 1.171e+04 & 2.234e+04 & 4.759e-01 & 1.530e+04\\
  
  dwt\_87 & 1.024e+04 & 5.506e+03 & 1.024e+04 & 4.624e-01 & 5.077e+03\\
  
  ibm32 & 1.633e+05 & 4.762e+04 & 1.633e+05 & 7.084e-01 & 8.383e+04\\
  
  nos4 & 2.492e+06 & 9.715e+05 & 9.903e+05 & 6.101e-01 & 1.096e+06\\
  
  west0067 & 1.696e+04 & 2.716e+03 & 1.163e+04 & 8.398e-01 & 5.903e+03\\
  
  bfwa62 & 3.059e+05 & 3.868e+04 & 4.450e+04 & 8.735e-01 & 5.152e+04\\
  
  bfwb62 & 2.958e+02 & 2.307e+01 & 2.362e+01 & 9.220e-01 & 2.676e+01\\
  
  b1\_ss & 3.896e+04 & 9.353e+00 & 1.150e+02 & 9.998e-01 & 7.115e+01\\
  
  mesh1e1 & 2.756e+01 & 1.432e+01 & 1.727e+01 & 4.802e-01 & 1.500e+01\\
  
  mesh1em1 & 3.609e+02 & 1.300e+02 & 1.346e+02 & 6.399e-01 & 1.553e+02\\
  
  mesh1em6 & 3.731e+01 & 2.322e+01 & 2.394e+01 & 3.776e-01 & 2.348e+01\\
  
  cage3 & 3.552e+02 & 8.628e+01 & 1.503e+02 & 7.571e-01 & 2.324e+02\\
  
  cage4 & 3.749e+02 & 6.917e+01 & 9.644e+01 & 8.155e-01 & 2.332e+02\\
  
  cage5 & 2.377e+02 & 3.179e+01 & 6.664e+01 & 8.662e-01 & 1.446e+02\\
  
  cage6 & 1.305e+02 & 2.199e+01 & 3.265e+01 & 8.315e-01 & 5.598e+01\\
  
  Cities & 4.291e+04 & 5.647e+03 & 3.202e+04 & 8.684e-01 & 1.275e+04\\
  
  divorce & 3.760e+02 & 1.749e+00 & 3.760e+02 & 9.953e-01 & 1.794e+02\\
  
  GD95\_c & 2.651e+03 & 6.847e+02 & 2.651e+03 & 7.417e-01 & 1.357e+03\\
  
  Stranke94 & 2.676e+03 & 1.993e+03 & 2.499e+03 & 2.554e-01 & 2.339e+03\\
  
  Tina\_AskCog & 3.914e+02 & 1.655e+02 & 3.914e+02 & 5.771e-01 & 2.897e+02\\
  
  CAG\_mat72 & 7.720e+07 & 1.098e+06 & 9.330e+06 & 9.858e-01 & 1.707e+07\\
  
  Trefethen\_20b & 9.212e+02 & 6.245e+00 & 6.665e+00 & 9.932e-01 & 8.697e+00\\
  
  Trefethen\_20 & 3.980e+03 & 1.711e+01 & 1.904e+01 & 9.957e-01 & 2.859e+01\\
  
  mycielskian2 & 1.000e+00 & 1.000e+00 & 1.000e+00 & 1.000e+00 & 1.000e+00\\
  
  mycielskian4 & 9.391e+01 & 4.220e+01 & 9.391e+01 & 5.506e-01 & 8.476e+01\\
  
  mycielskian5 & 7.641e+02 & 1.618e+02 & 7.641e+02 & 7.882e-01 & 6.110e+02\\
  
  mycielskian6 & 5.863e+03 & 4.240e+02 & 5.863e+03 & 9.277e-01 & 4.139e+03\\
  
  mycielskian7 & 4.337e+04 & 4.753e+03 & 4.337e+04 & 8.904e-01 & 2.700e+04\\
  
  ash219 & 9.150e+00 & 3.124e+00 & 9.150e+00 & 6.585e-01 & 4.194e+00\\
  
  ash331 & 9.588e+00 & 2.954e+00 & 9.588e+00 & 6.919e-01 & 3.668e+00\\
  
  ash608 & 1.138e+01 & 3.012e+00 & 1.138e+01 & 7.353e-01 & 3.861e+00\\
  
  bcspwr03 & 2.514e+05 & 7.948e+04 & 2.514e+05 & 6.839e-01 & 1.137e+05\\
  
  bcsstm05 & 1.612e+02 & 1.000e+00 & 1.000e+00 & 9.938e-01 & 1.000e+00\\
  
  WorldCities & 4.356e+03 & 1.979e+03 & 3.283e+03 & 9.546e+00 & --\\
  
  arc130 & 3.665e+21 & 1.276e+00 & 1.490e+12 & 1.000e+00 & --\\
  \hline
\end{tabular}
  \caption{\texttt{SuiteSparse} Datset, "--": SDP fails}
  \label{tab:two-sided-comparison}
\end{table}
