# Supplementary material for: Optimal Diagonal Preconditioning
Source: arXiv:2209.00809 source file (2022-11-04)
Supplement: Supplementary file 11 [file appendix_optimal_old.tex]

\subsection{An Interior Point Algorithm for Optimal Diagonal Preconditioning}
\label{sec:potential-reduction}
Although the baseline algorithm introduced above is easy to implement, it suffers from sub-optimal complexity in theory and limited problem size in practice. In this section, we focus
on developing an interior point method that finds an $\epsilon$-optimal
solution in $O(\log\frac{1}{\epsilon})$ iterations, where each
iteration only consists of a Newton update step. This enjoys better
complexity than the baseline algorithm based on bisection, which requires solving an SDP feasibility problem at each iteration. Our algorithm draws inspirations from interior point
methods for linear programming and semidefinite programming 
\citep{mizuno1992new,ye1992potential,ye1995neumann,nesterov1997self},
particularly \cite{nesterov1997self}
on directions of Newton updates in interior point methods for SDPs and \cite{ye1995neumann}
on the ``Von Neumann economic growth problem'' \citep{von1937uber,neumann1945model}. 
%Add a remark on the connection to the Von Neumann problem of the right preconditioning problem.

Recall the reformulated two-sided optimal diagonal preconditioning problem in \eqref{eq:SDP-two-sided}. For ease of exposition, we present the algorithm and theory for the following right preconditioning problem by setting $D_1=I_m$ in \eqref{eq:SDP-two-sided}: %Extension to the two-sided problem can be found in the appendix.
\begin{align*}
\min_{\kappa\geq0}\kappa\\
A^{T}A\succeq D\\
\kappa D\succeq A^{T}A
\end{align*}
Let $\kappa^{\ast}\in[1,\infty)$ be optimal objective value of the above problem. Following \cite{ye1995neumann}, with $M=A^TA$, we define the \textbf{potential function} on $(\kappa^\ast,\infty)$
as
\begin{align*}
P(\kappa) & :=\sum_{i}\log\lambda_{i}(M-D^{\kappa})+\sum_{i}\log\lambda_{i}(\kappa D^{\kappa}-M)+\sum_{i}\log D_{ii}^{\kappa}
\end{align*}
where $D^{\kappa}$ is the \textbf{analytic center} of the feasible
region \textbf{
	\begin{align*}
	\Gamma(\kappa) & =\{D\succeq0:D\text{ diagonal};M\succeq D;\kappa D\succeq M\}
	\end{align*}
} which is simply the unique maximizer of the strictly concave problem
\begin{align*}
\max_{D\succeq0\text{ diagonal}} & \sum_{i}\log\lambda_{i}(M-D)+\sum_{i}\log\lambda_{i}(\kappa D-M)+\sum_{i}\log D_{ii}\\
& \Longleftrightarrow\\
\max_{D\succeq0\text{ diagonal}} & \log\det(M-D)+\log\det(\kappa D-M)+\log\det D
\end{align*}

See also \cite{mizuno1993adaptive,luo1998superlinear,sturm1999symmetric}
for the use of analytic centers in path-following and potential reduction
interior point algorithms for LP and SDP problems. 

The geometric interpretation of the problem makes it clear that if
the feasible region $\Gamma(\kappa^{0})$ has a non-empty interior
for some $\kappa^{0}<\infty$, then the feasible region $\Gamma(\kappa)$
has a non-empty interior for all $\kappa\geq\kappa^{0}$, so that
the analytic center is well defined. At the optimal objective value
$\kappa^{\ast}\geq1$, however, the solution set has no interior because
it must be the case that $\lambda_{n}(\kappa D-M)=0$ for any $D$
in the solution set, where $\lambda_{1}\geq\lambda_{2}\geq\cdots\geq\lambda_{n}$
are the eigenvalues of a matrix, and so perturbing $D$ in some direction
by any amount will violate the constraint $M\succeq D$. 
\begin{lemma}
	For $M\succ0,$ the feasible set of the feasibility problem 
	\begin{align*}
	\min_{D\succeq0}0\\
	M\succeq D\\
	\kappa D\succeq M
	\end{align*}
	has bounded non-empty interior for any $\kappa>\kappa^{\ast}$.
\end{lemma}
Next, we show that the potential function is monotonic in $\kappa$,
and that it is bounded away from $P(\kappa^{\ast})$, for any $\kappa$
large. This implies that $P(\kappa)$ is a reasonable measure of the progress of an algorithm:
to obtain an approximate optimal solution to the optimal preconditioning problem, it suffices to reduce the potential function by a constant
amount at every step and terminate when the potential function is
reduced below a certain threshold determined by accuracy $\epsilon$. This is summarized in the following two results. All proofs in this section can be found in the appendix.
\begin{proposition}\label{prop:monotonicity}
	If $\kappa_{0}>\kappa_{1}>\kappa^{\ast}$, then $P(\kappa_{0})>P(\kappa_{1})$. 
\end{proposition}
%
\begin{proposition}\label{prop:lower bound}
	Let $t$ satisfy $\kappa^{\ast}\leq2^{t}$, then for any $\overline{\kappa}>\kappa^{\ast}+2^{-t}$,
	we have
	\begin{align*}
	P(\overline{\kappa}) & >-Cnt
	\end{align*}
	for some universal constant that only depends on $M$. 
\end{proposition}
These two results imply that if $P(\kappa)<O(-nt)$, then we must
have $\kappa\leq\kappa^{\ast}+2^{-t}$. Therefore, if we can find a
$D$ whose associated potential is below the threshold of $O(n\log\epsilon)$,
we have found an approximate solution that yields a condition number
that is within $\epsilon$ of the optimal condition number. Our goal
is then to design an algorithm that achieves constant reduction of
the potential at every iteration, which would guarantee an iteration
complexity of $O(\log\frac{1}{\epsilon})$. 

In the next two subsections, we develop potential reduction algorithms based on this idea, using exact and approximate analytic centers, respetively. Before doing so, we show that the analytic center satisfies an equality condition that is useful in the analysis of the reduction of the potential function. It is essentially the first order condition of the convex optimziation problem. Since it also serves an important role in the Newton step, we state it in a particular form in the next lemma. 
\begin{lemma}
	The analytic center $D$ of the feasible region $\Gamma(\kappa)$
	satisfies 
	\begin{align*}
	Z+\kappa Y & =X
	\end{align*}
	where with $R:=M-D$, $S:=\kappa D-M$,  \begin{align*}
	X&=R^{-1},Y=S^{-1},Z=D^{-1}
	\end{align*}
\end{lemma}

\subsection{Analysis of Potential Reduction with Exact Analytic Centers}

Let $D^{0},D^{1}$ be the analytic centers of $\Gamma^{0}=\Gamma(\kappa^{0})$
and $\Gamma^{1}=\Gamma(\kappa^{1})$ for $\kappa^0,\kappa^1>\kappa^\ast$. With a suitable choice of $\Delta\kappa=\kappa^{0}-\kappa^{1}>0$,
we show that the analytic centers $D^{0}$ and $D^{1}$ are close,
and that 
\begin{align*}
P(\kappa^{1}) & \leq P(\kappa^{0})-\Omega(1)
\end{align*}
so that we can achieve constant reductions of the potential function
by updating from $D^{0}$ to $D^{1}$. To obtain $D^{1}$ from $D^{0}$,
we can use Newton iterations with a quadratic
convergence rate. The exact form of the Newton iteration is deferred
to the next subsection, where we propose a practical potential algorithm
using approximate analytic centers and only one Newton step.
%
\begin{theorem}
	\label{thm:exact center}Let $\overline{\kappa}$ be an upper bound of $\kappa^{\ast}$. Let $D^{0}$ and $D^{1}$ be the analytic centers of $\Gamma^{0}=\Gamma(\kappa^{0})$
	and $\Gamma^{1}=\Gamma(\kappa^{1})$ for $\kappa^{0},\kappa^{1}\in(\kappa^{\ast},\overline{\kappa})$.
	If $\Delta\kappa=\kappa^{0}-\kappa^{1}>0$ satisfies
	\begin{align*}
	\Delta\kappa & =\frac{\beta}{Tr(D^{0}\cdot(\kappa^{0}D^{0}-M)^{-1})}\\
	& =\frac{\beta}{e^{T}D^{0}\text{diag}((\kappa^{0}D^{0}-M)^{-1})e}
	\end{align*}
	for some sufficiently small $\beta\in(0,1)$ that only depends on
	$\overline{\kappa},M$, then 
	\begin{align*}
	\sqrt{Tr((D^{1})^{1/2}(D^{0})^{-1}(D^{1})^{1/2}-I)^{2}} & \leq c\cdot\beta\\
	\sqrt{Tr((D^{0})^{1/2}(D^{1})^{-1}(D^{0})^{1/2}-I)^{2}} & \leq c\cdot\beta
	\end{align*}
	for some constant $c$,
	and	$P(\kappa^{1}) \leq P(\kappa^{0})-\beta$.
	
\end{theorem}

%We have thus obtained a conceptual algorithm, which uses the exact
%analytic center, summarized in Algorithm \ref{alg:exact}.
\begin{algorithm}[Potential Reduction with Exact Analytic Center]
	\label{alg:exact}
\begin{enumerate}
	\normalfont 
	    \item Let $D^{0}$ be analytic center of $\Gamma(\kappa^{0})$ with some
	$\kappa^{0}>\kappa^{\ast}$. Set $k=0$. 
	
	\item  With a small fixed constant $0<\beta<1$, set 
	\begin{align*}
	\Delta\kappa^{k} & =\frac{\beta}{Tr(D^{0}\cdot(\kappa^{0}D^{0}-M)^{-1})},
	\end{align*}
and let $\kappa^{k+1}=\kappa^{k}-\Delta\kappa^{k}$.
	Then use Newton's method with updates of the form in Proposition \ref{prop:Newton step} to generate
	the exact analytic center $D^{k+1}$ of $\Gamma(\kappa^{k+1})$. 
	
	\item If $P(\kappa^{k+1})>O(-nt)$, set $k\leftarrow k+1$ and return
	to Step 1.
	\end{enumerate}
\end{algorithm}

\subsection{Algorithm with Approximate Analytic Center}

Given step size $\Delta\kappa$, in order to apply the potential reduction
algorithm, we still need to find the new analytic center $D^{1}$
corresponding to $\kappa^{0}-\Delta\kappa$. This can be achieved
using Newton iterations. However, it is not necessary to use exact
analytic centers. Instead, we can use an approximate analytic center
obtained from only one Newton update step, and show that the potential function
still reduces by a constant amount. Moreover, if we start from an approximate
analytic center, one Newton step with an appropriate step size $\Delta\kappa$
yields an approximate center that still achieves this constant reduction
in potential. We develop these results in this subsection. 

By an approximate analytic center, we mean a set of variables $(R,S,D,X,Y,Z)$
that satisfy the optimality conditions 
\begin{align*}
R & =M-D\succeq0\\
S & =\kappa D-M\succeq0\\
D & \succeq0\\
Z+\kappa Y & =X,
\end{align*}
but instead of requiring $RX=SY=DZ=I$ as is true for the exact analytic
center, we allow the products to be close to the identity $I$, where we use the following measure of proximity:
\begin{align*}
\delta(A,B) & :=\sqrt{Tr(B^{1/2}AB^{1/2}-I)^{2}}\\
& =\|B^{1/2}AB^{1/2}-I\|_{F}=\|A^{1/2}BA^{1/2}-I\|_{F}
\end{align*}
The second equality above follows from the fact that the Frobenius norm
is a spectral property for symmetric matrices. We may also check that
\begin{align*}
\delta(A,B) & =\sqrt{Tr((AB-I)^{2})}=\sqrt{Tr((BA-I)^{2})}
\end{align*}
As we will see in the following results, this is the appropriate measure
of proximity. The first result we show is that starting from an exact analytic
center for $\Gamma(\kappa^{0})$, we can obtain a feasible point in
$\Gamma(\kappa^{1})$ that is an $O(\beta)$ approximate analytic center.
\begin{proposition}
	\label{prop:initial}
	Let $D^{0}$ be the exact analytic center of $\kappa^{0}$. Define
	$R_{0}=M-D_{0}$, $S_{0}=\kappa_{0}D_{0}-M$ and $X_{0}=R_{0}^{-1},Y_{0}=S_{0}^{-1},Z_{0}=D_{0}^{-1}$.	Further, let $\Delta\kappa=\kappa^{0}-\kappa^{1}$ with $\Delta\kappa=\frac{\beta}{Tr(D^{0}\cdot(\kappa^{0}D^{0}-M)^{-1})}$
	where $\beta\in(0,1)$ is a sufficiently small constant, and 
	\begin{align*}
	\overline{R}^{0} & =R^{0},\overline{S}^{0}=-\Delta\kappa D^{0}+S^{0},\overline{D}^{0}=D^{0}\\
	\overline{X}^{0} & =X^{0},\overline{Y}^{0}=Y^{0},\overline{Z}^{0}=\Delta\kappa Y^{0}+Z^{0}
	\end{align*}
	Then, the new variables satisfy 
	\begin{align*}
	\overline{R}^{0} & =M-\overline{D}^{0}\succeq0\\
	\overline{S}^{0} & =\kappa^{1}\overline{D}^{0}-M\succeq0\\
	\overline{D}^{0} & \succeq0
	\end{align*}
	and $\overline{Z}^{0}+\kappa^{1}\overline{Y}^{0}=\overline{X}^{0}$.
	Moreover, $\delta(\overline{S}^{0},\overline{Y}^{0})\leq\beta,\delta(\overline{D}^{0},\overline{Z}^{0})\leq\beta,\delta(\overline{R}^{0},\overline{X}^{0})=0$.
\end{proposition}
Next we show that this set of variables $(\overline{R}^{0},\overline{S}^{0},\overline{D}^{0},\overline{X}^{0},\overline{Y}^{0},\overline{Z}^{0})$
can be used as an initial set to generate a new $ O(\beta^{2}) $ approximate center
for $\kappa^{1}$, using a Newton step. This also implies that starting from an approximate analytic center we can obtain an exact analytic center by applying the Newton iterations with quadratic convergence. Here to ensure the symmetry
of updates in the Newton step, we use the Nesterov-Todd direction
\citep{todd1998nesterov,nesterov1997self}. 

\begin{proposition}
   \label{prop:Newton step}
   Let $(\overline{R}^{0},\overline{S}^{0},\overline{D}^{0},\overline{X}^{0},\overline{Y}^{0},\overline{Z}^{0})$
	be any set that satisfy 
	\begin{align*}
	\overline{R}^{0} & =M-\overline{D}^{0}\succeq0\\
	\overline{S}^{0} & =\kappa^{1}\overline{D}^{0}-M\succeq0\\
	\overline{D}^{0} & \succeq0
	\end{align*}
	and $\overline{Z}^{0}+\kappa^{1}\overline{Y}^{0}=\overline{X}^{0}$,
	with 
	\begin{align*}
	\delta(\overline{R}^{0},\overline{X}^{0})=\|(\overline{R}^{0})^{\frac{1}{2}}\overline{X}^{0}(\overline{R}^{0})^{\frac{1}{2}}-I\|_{F} & \leq\beta\\
	\delta(\overline{D}^{0},\overline{Z}^{0})=\|(\overline{D}^{0})^{\frac{1}{2}}\overline{Z}^{0}(\overline{D}^{0})^{\frac{1}{2}}-I\|_{F} & \leq\beta\\
	\delta(\overline{S}^{0},\overline{Y}^{0})=\|(\overline{S}^{0})^{\frac{1}{2}}\overline{Y}^{0}(\overline{S}^{0})^{\frac{1}{2}}-I\|_{F} & \leq\beta
	\end{align*}
	for some $\beta\in(0,1)$.	Let $X^{1},Y^{1},Z^{1},R^{1},S^{1},D^{1}$ be defined by 
	\begin{align*}
	X^{1} & =\overline{X}^{0}+\Delta X,Y^{1}=\overline{Y}^{0}+\Delta Y,Z^{1}=\overline{Z}^{0}+\Delta Z\\
	R^{1} & =\overline{R}^{0}+\Delta R,S^{1}=\overline{S}^{0}+\Delta S,D^{1}=\overline{D}^{0}+\Delta D
	\end{align*}
	where the increments $\Delta$s are given by the Newton step %
	\begin{comment}
	The Newton step is to ensure 
	\begin{align*}
	\overline{R}^{0} & =M-\overline{D}^{0}\succeq0\\
	\overline{S}^{0} & =\kappa^{1}\overline{D}^{0}-M\succeq0\\
	\overline{D}^{0} & \succeq0
	\end{align*}
	and 
	\begin{align*}
	\overline{Z}^{0}+\kappa^{1}\overline{Y}^{0} & =\overline{X}^{0}
	\end{align*}
	still holds. 
	
	Regular Newton step is
	
	\begin{align*}
	\overline{D}^{0}\cdot\Delta Z+\overline{Z}^{0}\cdot\Delta D & =I-\overline{D}^{0}\cdot\overline{Z}^{0}\\
	\overline{R}^{0}\cdot\Delta X+\overline{X}^{0}\cdot\Delta R & =I-\overline{R}^{0}\cdot\overline{X}^{0}\\
	\overline{S}^{0}\cdot\Delta Y+\overline{Y}^{0}\cdot\Delta S & =I-\overline{S}^{0}\cdot\overline{Y}^{0}
	\end{align*}
	but here we need to use the Nesterov-Todd direction to ensure symmetry
	of updates. 
	\end{comment}
	\begin{align*}
	\Delta Z+W^{-1}\Delta DW^{-1} & =(\overline{D}^{0})^{-1}-\overline{Z}^{0}\\
	\Delta X+U^{-1}\Delta RU^{-1} & =(\overline{R}^{0})^{-1}-\overline{X}^{0}\\
	\Delta Y+V^{-1}\Delta S & V^{-1}=(\overline{S}^{0})^{-1}-\overline{Y}^{0}
	\end{align*}
	{} and 
	$\Delta R  =-\Delta D,\Delta S=\kappa^{1}\Delta D,\Delta X=\Delta Z+\kappa^{1}\Delta Y$,
	where $U,V,W$ are the geometric means 
	\begin{align*}
	U & =(\overline{R}^{0})^{1/2}((\overline{R}^{0})^{1/2}\overline{X}^{0}(\overline{R}^{0})^{1/2})^{-1/2}(\overline{R}^{0})^{1/2}\\
	V & =(\overline{S}^{0})^{1/2}((\overline{S}^{0})^{1/2}\overline{Y}^{0}(\overline{S}^{0})^{1/2})^{-1/2}(\overline{S}^{0})^{1/2}\\
	W & =(\overline{D}^{0})^{1/2}((\overline{D}^{0})^{1/2}\overline{Z}^{0}(\overline{D}^{0})^{1/2})^{-1/2}(\overline{D}^{0})^{1/2}
	\end{align*}
	to ensure that updates are symmetric. Then we have 
	\begin{align*}
	\delta(R^{1},X^{1})=\|(R^{1})^{\frac{1}{2}}X^{1}(R^{1})^{\frac{1}{2}}-I\|_{F} & \leq\frac{1}{2}\frac{\beta^{2}}{1-\beta}\\
	\delta(S^{1},Y^{1})=\|(S^{1})^{\frac{1}{2}}Y^{1}(S^{1})^{\frac{1}{2}}-I\|_{F} & \leq\frac{1}{2}\frac{\beta^{2}}{1-\beta}\\
	\delta(D^{1},Z^{1})=\|(D^{1})^{\frac{1}{2}}Z^{1}(D^{1})^{\frac{1}{2}}-I\|_{F} & \leq\frac{1}{2}\frac{\beta^{2}}{1-\beta}
	\end{align*}
	and 
	\begin{align*}
	\|(\overline{D}^{0})^{-\frac{1}{2}}D^{1}(\overline{D}^{0})^{-\frac{1}{2}}-I\|_{F} & \le\frac{\beta}{1-\beta}.
	\end{align*}
\end{proposition}
%
Our next result shows that starting from an $O(\delta)$ approximate
center $(R^{0},S^{0},D^{0},X^{0},Y^{0},Z^{0})$ instead of an exact
center for $\kappa^{0}$, by following the procedures described in
Proposition \ref{prop:initial} to form the initial set $(\overline{R}^{0},\overline{S}^{0},\overline{D}^{0},\overline{X}^{0},\overline{Y}^{0},\overline{Z}^{0})$
for $\kappa^{1}$, this intial set also satisfies the closeness conditions
\begin{align*}
\delta(\overline{R}^{0},\overline{X}^{0}) & \leq\delta',\delta(\overline{D}^{0},\overline{Z}^{0})\leq\delta',\delta(\overline{S}^{0},\overline{Y}^{0})\leq\delta'
\end{align*}
for $\delta'=\beta+\delta$, i.e. it is an $O(\beta+\delta)$ approximate
analytic center for $\kappa^{1}$, for $\delta$ sufficiently small.
This $O(\beta+\delta)$ approximate center can then be used in the
Newton step in Proposition \ref{prop:Newton step} to obtain
an $O((\beta+\delta)^{2})=O(\delta)$ approximate center for $\kappa^{1}$,
thus ensuring that we can go from an $O(\delta)$ approximate center
for $\kappa^{0}$ to an $O(\delta)$ approximate center for $\kappa^{1}$
with a single Newton step. 
\begin{proposition}\label{prop:approximate}
	Suppose that $(R^{0},S^{0},D^{0},X^{0},Y^{0},Z^{0})$ satisfy 
	\begin{align*}
	R^{0} & =M-D^{0}\succeq0\\
	S^{0} & =\kappa^{0}S^{0}-M\succeq0\\
	D^{0} & \succeq0\\
	Z^{0}+\kappa^{0}Y^{0} & =X^{0}
	\end{align*}
	with $\delta(R^{0},X^{0})\leq\delta,\delta(D^{0},Z^{0})\leq\delta,\delta(S^{0},Y^{0})\leq\delta$
	for some $\delta\in(0,1)$. Further, let $\Delta\kappa=\kappa^{0}-\kappa^{1}$
	with 
	\begin{align*}
	\Delta\kappa & =\frac{\beta}{Tr(D^{0}\cdot(\kappa^{0}D^{0}-M)^{-1})}
	\end{align*}
	where $\beta\in(0,1)$ is a sufficiently small constant, then with
	\begin{align*}
	\overline{R}^{0} & =R^{0},\overline{S}^{0}=-\Delta\kappa D^{0}+S^{0},\overline{D}^{0}=D^{0}\\
	\overline{X}^{0} & =X^{0},\overline{Y}^{0}=Y^{0},\overline{Z}^{0}=\Delta\kappa Y^{0}+Z^{0}
	\end{align*}
	we have 
	$\overline{R}^{0} =M-\overline{D}^{0}\succeq0$, $\overline{S}^{0} =\kappa^{1}\overline{D}^{0}-M\succeq 0$, $\overline{D}^{0} \succeq0$, $\overline{Z}^{0}+\kappa^{1}\overline{Y}^{0} =\overline{X}^{0}$,
	and $\delta(\overline{R}^{0},\overline{X}^{0})  \leq\beta$, $\delta(\overline{S}^{0},\overline{Y}^{0})\leq\delta+\beta$, $\delta(\overline{D}^{0},\overline{Z}^{0})\leq\delta+\beta$.

\end{proposition}
%
The above three results guarantee that if we start from an $O(\delta)$
approximate center for $\kappa^{0}$, by taking a small but constant
step $\Delta\kappa$, a Newton update step yields an $O(\delta)$
approximate center for $\kappa^{1}=\kappa^{0}-\Delta\kappa$, and
we may iteratively generate approximate centers in this fashion. In
the next result, we show that approximate centers, as the name suggests,
yields a potential that is close to that of the exact center, and
we have thus obtained an algorithm with approximate centers, such that the reduction
in potential at every step is constant, and the termination criterion
is the same as before, when the potential drops below
some threshold. 
\begin{theorem}
	\label{thm:approximate center}Let $\overline{D}^{0}$ and $\overline{D}^{1}$
	be approximate centers for $\kappa^{0}$ and $\kappa^{1}=\kappa^{0}-\frac{\beta}{Tr(\overline{D}^{0}\cdot(\kappa^{0}\overline{D}^{0}-M)^{-1})}$
	respectively, obtained using the procedures in Proposition \ref{prop:initial}
	to generate a feasible point and the Newton update with Nesterov-Todd
	directions for $\beta$ sufficiently small. If 
	\begin{align*}
	\delta(\overline{R}^{0},\overline{X}^{0}) & \leq\delta,\delta(\overline{D}^{0},\overline{Z}^{0})\leq\delta,\delta(\overline{S}^{0},\overline{Y}^{0})\leq\delta
	\end{align*}
	for $\delta$ a small universal constant, then 
	\begin{align*}
	\delta(\overline{R}^{1},\overline{X}^{1}) & \leq\delta,\delta(\overline{D}^{1},\overline{Z}^{1})\leq\delta,\delta(\overline{S}^{1},\overline{Y}^{1})\leq\delta
	\end{align*}
	and $P(\overline{D}^{1},\kappa^{1})\leq P(\overline{D}^{0},\kappa^{0})-c\beta$
	for $c\in(0,1)$ a universal constant. 
\end{theorem}
%The above result thus guarantees that if we start from an approximate center that is accurate enough, we can always ensure that the updated approximate center obtained from a Newton step with Nesterov-Todd direction remain as accurate, given small but constant step size.
\begin{algorithm}[Potential Reduction with Approximate Analytic Center]
	\label{alg:approximate}
	\begin{enumerate}
	\normalfont
	    \item  Let $\overline{D}^{0}$ be an $O(\beta)$ approximate analytic
	center of $\Gamma(\kappa^{0})$ with $\kappa^{0}>\kappa^{\ast}$.
	Set $k=0$. 
	
	\item Let $\Delta\kappa^{k}=\frac{\beta}{Tr(\overline{D}^{0}\cdot(\kappa^{0}\overline{D}^{0}-M)^{-1})}$
	for fixed constant $0<\beta<1$ and let $\kappa^{k+1}=\kappa^{k}-\Delta\kappa^{k}$.
	Update 
	\begin{align*}
	\overline{S}^{0}\leftarrow & -\Delta\kappa\overline{D}^{0}+\overline{S}^{0}\\
	\overline{Z}^{0}\leftarrow & \Delta\kappa Y^{0}+\overline{Z}^{0}
	\end{align*}
	to obtain feasible point for $\kappa^{k+1}$. 
	
	\item Use Newton's update to generate approximate analytic center
	$\overline{D}^{k+1}$ of $\Gamma(\kappa^{k+1})$. 
	
	\item If $P(\kappa^{k+1})>O(-nt)$, set $k\leftarrow k+1$ and return
	to Step 1. 
	\end{enumerate}
\end{algorithm}
%
Our results in this section provided us with algorithms that generate two-sided
optimal diagonal preconditioners  given any fixed matrix $A$. In practice, we observe that running
the bisection algorithm for a few itereations already
generates a pair of preconditioners $(D_1,D_2)$ with high quality. In numerical experiments in Section \ref{sec:experiments}, we will implement the bisection algorithm to solve \eqref{eq:two-sided-problem} when
comparing with other preconditioning techniques, including the one-sided optimal diagonal preconditioners via SDPs introduced next in Section \ref{sec:DSDP}.


\section{Details on the Interior Point Algorithm in Section \ref{sec:potential-reduction}}
\label{sec:appendix_optimal}

\begin{prop}
 If $\kappa_{0}>\kappa_{1}>\kappa^{\ast}$,
	then $P(\kappa_{0})>P(\kappa_{1})$. 
\end{prop}
\proof{Proof}
Let $D^{0}$ and $D^{1}$ denote the analytic centers of $\Gamma(\kappa^{0})$
and $\Gamma(\kappa^{1})$, respectively. We know that $D^{1}$ is
contained in the feasible region $\Gamma(\kappa^{0})$, so that
\begin{align*}
P(\kappa_{0})\geq\sum_{i}\log\lambda_{i}(M-D^{1})+\sum_{i}\log\lambda_{i}(\kappa_{0}D^{1}-M)+\sum_{i}\log D^{1}\\
>\sum_{i}\log\lambda_{i}(M-D^{1})+\sum_{i}\log\lambda_{i}(\kappa_{1}D^{1}-M)+\sum_{i}\log D^{1} & =P(\kappa_{1})
\end{align*}
where the second inequality follows from the following minimax principle:
for any real symmetric matrix with $\lambda_{1}\geq\lambda_{2}\dots$, 

\begin{align*}
\lambda_{k} & =\min_{C}\max_{\|C\|=1,Cx=0}\langle Ax,x\rangle
\end{align*}
where $C$ is any $(k-1)\times n$ matrix. This implies that if $A\succeq B$,
$\lambda_{k}(A)\geq\lambda_{k}(B)$, since for 
\begin{align*}
C & =\arg\min_{C}\max_{\|C\|=1,Cx=0}\langle Ax,x\rangle
\end{align*}
we have 
\begin{align*}
\lambda_{k}(B)\leq\max_{\|C\|=1,Cx=0}\langle Bx,x\rangle & \leq\max_{\|C\|=1,Cx=0}\langle Ax,x\rangle=\lambda_{k}(A)
\end{align*}
and if $A\neq B$, then at least one inequality is strict. 
\hfill \halmos
\endproof
%
\begin{prop}
Let $t$ satisfy
	$\kappa^{\ast}\leq2^{t}$, then for any $\overline{\kappa}>\kappa^{\ast}+2^{-t}$,
	we have
	\begin{align*}
	P(\overline{\kappa}) & >-Cpt
	\end{align*}
	for some universal constant that only depends on $M$. 
\end{prop}

\proof{Proof}
	Recall that 
	\begin{align*}
	P(\kappa) & =\max_{D\succeq0}\log\det(M-D)+\log\det(\kappa D-M)+\log\det D
	\end{align*}
	
	Since $\overline{\kappa}>\kappa^{\ast}$, $\Gamma(\overline{\kappa})$
	has a bounded and nonempty interior. We claim that there exists an
	interior point $\overline{D}\in\Gamma(\overline{\kappa})$ such that
	\begin{align*}
	\overline{D} & \succeq2^{-Ct}I\\
	M-\overline{D} & \succeq2^{-Ct}I\\
	\overline{\kappa}\overline{D}-M & \succeq2^{-Ct}I
	\end{align*}
	for some $C$ that only depends on $M$. We may obtian this $\overline{D}$
	by shrinking any $D^{\ast}$ that satisfies 
	\begin{align*}
	M-D^{\ast} & \succeq0\\
	\kappa^{\ast}D^{\ast}-M & \succeq0\\
	D^{\ast} & \succeq0
	\end{align*}
	as follows. Given $D^{\ast}$ satisfying the above conditions, we
	can first find some $C$ such that $D^{\ast}\succeq2^{-Ct}I$. Then
	for $\delta>0$ sufficiently close to 0, 
	\begin{align*}
	M-2^{-\delta t}\cdot D^{\ast} & \succeq M-D^{\ast}+(D^{\ast}-2^{-\delta t}\cdot D^{\ast})\\
	& \succeq(1-2^{-\delta t})2^{-Ct}I\succeq2^{-C't}I
	\end{align*}
	Finally, since $\overline{\kappa}>\kappa^{\ast}+2^{-t}$, we have
	\begin{align*}
	\overline{\kappa}2^{-\delta t}D^{\ast}-M & \succeq(\kappa^{\ast}+2^{-t})2^{-\delta t}D^{\ast}-M\\
	& \succeq2^{-(1+\delta)t}D^{\ast}\succeq2^{-C't}I
	\end{align*}
	so that $\overline{D}=2^{-\delta t}D^{\ast}$ satisfies the required
	conditions. This implies that $P(\overline{\kappa})\geq P(\overline{D},\overline{\kappa})>-Cpt$. 
	\hfill \halmos
\endproof
\begin{lem}
	The analytic center $D$ of the feasible region $\Gamma(\kappa)$
	satisfies 
	\begin{align*}
	Z+\kappa Y & =X
	\end{align*}
	where \begin{align*}
	X&=R^{-1},Y=S^{-1},Z=D^{-1},R=M-D,S=\kappa D-M
	\end{align*}
\end{lem}
\proof{Proof}
	Since $D$ solves the convex problem
	\begin{align*}
	& \max_{D}\log\det(M-D)+\log\det(\kappa D-M)+\log\det D
	\end{align*}
	The first order condition implies 
	\begin{align*}
	-(M-D)^{-1}+\kappa(\kappa D-M)^{-1}+D^{-1} & =0
	\end{align*}
	so if we define $R=M-D$ and $S=\kappa D-M$, and 
	\begin{align*}
	X	=R^{-1},Y=S^{-1},Z=D^{-1}
	\end{align*}
	then we have $	Z+\kappa Y  =X$ and moreover $R+S=(\kappa-1)D$. 
	\hfill \halmos
\endproof
 Recall the following property which is useful in our proof. 
\begin{lem}
	Let $X$ be a symmetric matrix, $\|X\|$ be the Frobenius norm, and
	$\|X\|_{\infty}=\max_{j}|\lambda_{j}(X)|$. Then if $\|X\|_{\infty}<1$,
	\begin{align*}
	Tr(X) & \geq\log\det(I+X)\geq Tr(X)-\frac{\|X\|^{2}}{2(1-\|X\|_{\infty})}
	\end{align*}
\end{lem}
\begin{thm}
	(Theorem \ref{thm:exact center} in the paper) Let $\kappa^{\ast}\in[1,\infty)$
	be the solution of 
	\begin{align*}
	\min_{D\succeq0}\kappa\\
	s.t.M\succeq D\\
	\kappa D\succeq M
	\end{align*}
	and let $\overline{\kappa}$ be a known upper bound of $\kappa^{\ast}$,
	i.e. 
	\begin{align*}
	\min_{D\succeq0}0\\
	s.t.M\succeq D\\
	\overline{\kappa}D\succeq M
	\end{align*}
	is feasible. 
	
	Let $D^{0}$ and $D^{1}$ be the analytic centers of $\Gamma^{0}=\Gamma(\kappa^{0})$
	and $\Gamma^{1}=\Gamma(\kappa^{1})$ for $\kappa^{0},\kappa^{1}\in(\kappa^{\ast},\overline{\kappa})$.
	If $\Delta\kappa=\kappa^{0}-\kappa^{1}>0$ satisfies
	\begin{align*}
	\Delta\kappa & =\frac{\beta}{Tr(D^{0}\cdot(\kappa^{0}D^{0}-M)^{-1})}\\
	& =\frac{\beta}{e^{T}D^{0}\text{diag}((\kappa^{0}D^{0}-M)^{-1})e}
	\end{align*}
	for some sufficiently small $\beta\in(0,1)$ that only depends on
	$\overline{\kappa},M$, then 
	\begin{align*}
	Tr(D^{1}(D^{0})^{-1}) & \leq O(1)\\
	Tr(D^{0}(D^{1})^{-1}) & \leq O(1)
	\end{align*}
	and\textbf{
		\begin{align*}
		P(\kappa^{1}) & \leq P(\kappa^{0})-\beta
		\end{align*}
	}
\end{thm}
\proof{Proof}
	First note that the function
	\begin{align*}
	P(D,\kappa) & =\log\det(M-D)+\log\det(\kappa D-M)+\log\det D
	\end{align*}
	is jointly concave in $(\kappa,D)$ on any convex set $(\underline{\kappa},\infty)\times\mathcal{D}(\underline{\kappa})$
	for any $\underline{\kappa}>\kappa^{\ast}$, and $\mathcal{D}(\kappa)$
	is the set of all positive matrices such that $\kappa D-M\succ0$.
	This implies that 
	\begin{align*}
	\underline{P}(\kappa) & =\max_{D\in\mathcal{D}(\underline{\kappa})}\log\det(M-D)+\log\det(\kappa D-M)+\log\det D
	\end{align*}
	is a concave function on $(\underline{\kappa},\infty)$. Note, however,
	that $\underline{P}(\kappa)$ is not necessarily equal to $P(\kappa)$,
	because for $\kappa^{0}>\underline{\kappa}$, the solution $D^{0}$
	of 
	\begin{align*}
	\max_{D\in\mathcal{D}(\kappa^{0})}\log\det(M-D)+\log\det(\kappa^{0}D-M)+\log\det D
	\end{align*}
	does not necessarily satisfy $D^{0}\in\mathcal{D}(\underline{\kappa})$.
	Fortunately, since the optimizer $D(\kappa)$ corresponding to each
	$\kappa$ is always in the interior of $\mathcal{D}(\kappa)$, if
	$\beta$ is small enough, we can guarantee that $D^{0}\in\mathcal{D}(\kappa^{1})$
	with $\kappa^{1}=\kappa^{0}-\Delta\kappa$ and $\Delta\kappa=\frac{\beta}{Tr(D^{0}\cdot(\kappa^{0}D^{0}-M)^{-1})}$.
	More precisely, with $D^{0}$ being the solution of 
	\begin{align*}
	\max_{D\in\mathcal{D}(\kappa^{0})}\log\det(M-D)+\log\det(\kappa^{0}D-M)+\log\det D
	\end{align*}
	and $\kappa^{1}=\kappa^{0}-\Delta\kappa$, we have 
	
	\begin{align*}
	|\lambda_{n}(\kappa^{1}D^{0}-M)-\lambda_{n}(\kappa^{0}D^{0}-M)| & \leq\Delta\kappa\cdot\max_{i}D_{ii}^{0}\\
	& =\frac{\beta}{Tr(D^{0}\cdot(\kappa^{0}D^{0}-M)^{-1})}\cdot\max_{i}D_{ii}^{0}\\
	& \leq\frac{\beta}{(\min_{i}D_{ii}^{0})\cdot\lambda_{1}((\kappa^{0}D^{0}-M)^{-1})}\cdot\max_{i}D_{ii}^{0}\\
	& =\beta\cdot\kappa(D^{0})\cdot\lambda_{n}(\kappa^{0}D^{0}-M)
	\end{align*}
	where we have used Weyl's inequality and 
	\begin{align*}
	Tr(D^{0}\cdot(\kappa^{0}D^{0}-M)^{-1}) & \geq Tr(\min{}_{i}D_{ii}^{0}\cdot I\cdot(\kappa^{0}D^{0}-M)^{-1})\\
	& \geq\min{}_{i}D_{ii}^{0}\cdot\lambda_{1}((\kappa^{0}D^{0}-M)^{-1})
	\end{align*}
	
	Since $\kappa(D^{0})$ is bounded above by some universal constant
	that only depends on $M,\overline{\kappa}$, with $\beta$ small enough,
	we have 
	\begin{align*}
	\lambda_{n}(\kappa^{1}D^{0}-M) & \geq\lambda_{n}(\kappa^{0}D^{0}-M)-\beta\cdot\kappa(D^{0})\cdot\lambda_{n}(\kappa^{0}D^{0}-M)\\
	& >0
	\end{align*}
	so that $D^{0}$ is in the interior of $\mathcal{D}(\kappa^{1})$. 
	
	Thus on any interval $[\kappa^{1},\kappa^{0}]\subset(\kappa^{\ast},\overline{\kappa})$
	with length bounded by $\frac{\beta}{Tr(D^{0}\cdot(\kappa^{0}D^{0}-M)^{-1})}$,\textbf{
	}the function 
	\begin{align*}
	P(\kappa) & =\max_{D\in\mathcal{D}(\kappa)}\log\det(M-D)+\log\det(\kappa D-M)+\log\det D
	\end{align*}
	is concave in $\kappa$. 
	
	Now 
	\begin{align*}
	P(\kappa) & =P(D(\kappa),\kappa)
	\end{align*}
	where $D(\kappa)$ is the unique maximizer corresponding to $\kappa$,
	so that 
	\begin{align*}
	\frac{d}{d\kappa}P(\kappa) & =Tr(\nabla_{D}P(D(\kappa),\kappa)\cdot\partial_{\kappa}D(\kappa))+\partial_{\kappa}P(D(\kappa),\kappa)\\
	& =\partial_{\kappa}P(D(\kappa),\kappa)\\
	& =Tr(D\cdot(\kappa D-M)^{-1})
	\end{align*}
	using the envelope theorem, or equivalently the first order condition
	of the maximization problem. By concavity of $P(\kappa)$, we have
	\begin{align*}
	P(\kappa^{1})-P(\kappa^{0}) & \leq\frac{d}{d\kappa}P(\kappa)\mid_{\kappa^{0}}\cdot(\kappa^{1}-\kappa^{0})\\
	& =-\Delta\kappa\cdot Tr(D^{0}\cdot(\kappa^{0}D^{0}-M)^{-1})\\
	& =-\beta
	\end{align*}
	and since $P(\kappa)$ is increasing and concave on $[\kappa^{1},\kappa^{0}]$
	\begin{align*}
	|P(\kappa^{1})-P(\kappa^{0})| & \leq\max_{\kappa\in[\kappa^{1},\kappa^{0}]}|\frac{d}{d\kappa}P(\kappa)\mid_{\kappa}|\cdot\Delta\kappa\\
	& =\Delta\kappa\cdot Tr(D^{0}\cdot(\kappa^{1}D^{0}-M)^{-1})\\
	& =\beta\cdot\frac{Tr(D^{0}\cdot(\kappa^{1}D^{0}-M)^{-1})}{Tr(D^{0}\cdot(\kappa^{0}D^{0}-M)^{-1})}\\
	& \leq\beta\cdot\kappa(D^{0})\cdot\frac{Tr((\kappa^{1}D^{0}-M)^{-1})}{Tr((\kappa^{0}D^{0}-M)^{-1})}\\
	& =\beta\cdot\kappa(D^{0})\cdot\frac{\sum_{i}\frac{1}{\lambda_{i}(\kappa^{1}D^{0}-M)}}{\sum_{i}\frac{1}{\lambda_{i}(\kappa^{0}D^{0}-M)}}\\
	& =\beta\cdot\kappa(D^{0})\cdot\frac{\sum_{i}\frac{\lambda_{1}(\kappa^{0}D^{0}-M)}{\lambda_{i}(\kappa^{1}D^{0}-M)}}{\sum_{i}\frac{\lambda_{1}(\kappa^{0}D^{0}-M)}{\lambda_{i}(\kappa^{0}D^{0}-M)}}\\
	& \leq\beta\cdot\kappa(D^{0})\cdot\frac{\sum_{i}\frac{\lambda_{1}(\kappa^{0}D^{0}-M)}{\lambda_{i}(\kappa^{1}D^{0}-M)}}{n}\\
	& =\beta\cdot\kappa(D^{0})\cdot\frac{\sum_{i}\frac{\lambda_{n}(\kappa^{1}D^{0}-M)}{\lambda_{i}(\kappa^{1}D^{0}-M)}}{n}\cdot\frac{\lambda_{1}(\kappa^{0}D^{0}-M)}{\lambda_{n}(\kappa^{1}D^{0}-M)}\\
	& \leq\beta\cdot\kappa(D^{0})\cdot\frac{\lambda_{1}(\kappa^{0}D^{0}-M)}{\lambda_{1}(\kappa^{1}D^{0}-M)}\cdot\frac{\lambda_{1}(\kappa^{1}D^{0}-M)}{\lambda_{n}(\kappa^{1}D^{0}-M)}
	\end{align*}
	and 
	\begin{align*}
	\frac{\lambda_{1}(\kappa^{0}D^{0}-M)}{\lambda_{1}(\kappa^{1}D^{0}-M)} & \leq C(\beta,\kappa^{\ast},\overline{\kappa})\\
	\frac{\lambda_{1}(\kappa^{1}D^{0}-M)}{\lambda_{n}(\kappa^{1}D^{0}-M)} & \leq C(\beta,\kappa^{\ast},\overline{\kappa})
	\end{align*}
	by a similar argument as before. So there exists $\xi>0$ depending
	only on $\beta,\kappa^{\ast},\overline{\kappa}$, so that
	\begin{align*}
	-\xi-\beta\leq P(\kappa^{1})-P(\kappa^{0}) & \leq-\beta
	\end{align*}
	
	\textbf{}%
	\begin{comment}
	\begin{proof}
	\textbf{Now 
	\begin{align*}
	P(\kappa^{1})-P(\kappa^{0}) & =\log\det(M-D^{1})+\log\det(\kappa^{1}D^{1}-M)+\log\det D^{1}\\
	& -\log\det(M-D^{0})-\log\det(\kappa^{0}D^{0}-M)-\log\det D^{0}
	\end{align*}
	and }
	\begin{align*}
	-Tr((D^{1}-D^{0})+Tr(\nabla_{D}P(\kappa^{0},D^{0})\cdot(D^{1}-D^{0})) & \geq P(\kappa^{0},D^{1})-P(\kappa^{0},D^{0})\\
	\end{align*}
	\begin{align*}
	D\\
	\end{align*}
	
	\begin{align*}
	\log\det(\kappa^{1}D^{0}-M)-\log\det(\kappa^{0}D^{0}-M) & =(\kappa^{1}-\kappa^{0})\cdot Tr(D^{0}\cdot(\kappa^{0}D^{0}-M)^{-1})\\
	& \leq-\beta\\
	\end{align*}
	
	\begin{align*}
	Tr((D^{0})^{-1}D^{1}-I)\\
	\end{align*}
	\begin{align*}
	\log\det D^{1}-\log\det D^{0} & \leq Tr((D^{0})^{-1}(D^{1}-D^{0}))\\
	\end{align*}
	\end{proof}
	\end{comment}
	
	Now we show that $D^{0}$ and $D^{1}$ are close. Recall the inequality
	
	\begin{align*}
	Tr(X) & \geq\log\det(I+X)\geq Tr(X)-\frac{\|X\|^{2}}{2(1-\|X\|_{\infty})}
	\end{align*}
	
	\begin{align*}
	\log\det((D^{0})^{-1}D^{1}) & \leq Tr((D^{0})^{-1}(D^{1}-D^{0}))\\
	& \leq\log\det((D^{0})^{-1}D^{1})+\frac{\|(D^{0})^{-1}(D^{1}-D^{0})\|}{2(1-\lambda_{1}((D^{0})^{-1}(D^{1}-D^{0}))}\\
	\log\det(M-D^{0})^{-1}(M-D^{1}) & \leq Tr((M-D^{0})^{-1}(D^{0}-D^{1})))\\
	& \leq\log\det(M-D^{0})^{-1}(M-D^{1})+\frac{\|(M-D^{0})^{-1}(D^{0}-D^{1})\|}{2(1-\lambda_{1}((M-D^{0})^{-1}(D^{0}-D^{1}))}\\
	\log\det(\kappa^{0}D^{0}-M)^{-1}(\kappa^{1}D^{1}-M) & \leq Tr((\kappa^{0}D^{0}-M)^{-1}(\kappa^{1}D^{1}-\kappa^{0}D^{0}))\\
	& \leq\log\det(\kappa^{0}D^{0}-M)^{-1}(\kappa^{1}D^{1}-M)+\frac{\|(\kappa^{0}D^{0}-M)^{-1}(\kappa^{1}D^{1}-\kappa^{0}D^{0})\|}{2(1-\lambda_{1}((\kappa^{0}D^{0}-M)^{-1}(\kappa^{1}D^{1}-\kappa^{0}D^{0}))}
	\end{align*}
	summing the inequalities, and using 
	\begin{align*}
	-(M-D^{0})^{-1}+\kappa^{0}(\kappa^{0}D^{0}-M)^{-1}+(D^{0})^{-1} & =0
	\end{align*}
	we have
	\begin{align*}
	-\Delta\kappa\cdot Tr((\kappa^{0}D^{0}-M)^{-1}D^{1}) & \geq P(\kappa^{1})-P(\kappa^{0})\\
	& \geq-\beta-\xi
	\end{align*}
	
	\textbf{}%
	\begin{comment}
	\textbf{
	\begin{align*}
	-\Delta\kappa\cdot Tr((\kappa^{0}D^{0}-M)^{-1}D^{1}) & \geq P(\kappa^{1})-P(\kappa^{0})\\
	& \geq-\Delta\kappa\cdot Tr((\kappa^{1}D^{1}-M)^{-1}D^{0})
	\end{align*}
	so that 
	\begin{align*}
	\frac{Tr((\kappa^{0}D^{0}-M)^{-1}D^{1})}{Tr((\kappa^{1}D^{1}-M)^{-1}D^{0})} & \leq1\\
	\end{align*}
	}
	\end{comment}
	Recall that 
	\begin{align*}
	\Delta\kappa & =\frac{\beta}{Tr(D^{0}\cdot(\kappa^{0}D^{0}-M)^{-1})}
	\end{align*}
	so that 
	\begin{align*}
	\frac{Tr((\kappa^{0}D^{0}-M)^{-1}D^{1})}{Tr(D^{0}\cdot(\kappa^{0}D^{0}-M)^{-1})} & \leq1+\frac{\xi}{\beta}
	\end{align*}
	and the left hand side is bounded below by 
	\begin{align*}
	\frac{Tr((\kappa^{0}D^{0}-M)^{-1}D^{1})}{Tr(D^{0}\cdot(\kappa^{0}D^{0}-M)^{-1})} & =\frac{Tr((\kappa^{0}D^{0}-M)^{-1}D^{0}\cdot(D^{0})^{-1}D^{1})}{Tr(D^{0}\cdot(\kappa^{0}D^{0}-M)^{-1})}\\
	& \geq\frac{\sum_{i}\lambda_{i}((\kappa^{0}D^{0}-M)^{-1}D^{0})\cdot\lambda_{n-i+1}((D^{0})^{-1}D^{1})}{Tr(D^{0}\cdot(\kappa^{0}D^{0}-M)^{-1})}\\
	& \geq\frac{(\sum_{i}\lambda_{i}^{2}((\kappa^{0}D^{0}-M)^{-1}D^{0}))^{\frac{1}{2}}\cdot(\sum_{i}\lambda_{n-i+1}^{2}((D^{0})^{-1}D^{1}))^{\frac{1}{2}}}{Tr(D^{0}\cdot(\kappa^{0}D^{0}-M)^{-1})}\cdot\eta\\
	& =\frac{\frac{1}{n}(\sum_{i}\lambda_{i}((\kappa^{0}D^{0}-M)^{-1}D^{0}))\cdot(\sum_{i}\lambda_{n-i+1}((D^{0})^{-1}D^{1}))}{Tr(D^{0}\cdot(\kappa^{0}D^{0}-M)^{-1})}\cdot\eta\\
	& =Tr((D^{0})^{-1}D^{1})\cdot\frac{1}{n}\cdot\eta
	\end{align*}
	where $\eta$ is upper bounded by a universal constant, so that 
	
	\begin{align*}
	Tr(D^{1}(D^{0})^{-1}) & \leq O(1)
	\end{align*}
	\begin{comment}
	\begin{proof}
	From the concavity of $\log\det X$, we have 
	\begin{align*}
	\log\det X-\log\det Y & \leq Tr((X-Y)Y^{-1})\\
	& =Tr(Y^{-\frac{1}{2}}(X-Y)Y^{-\frac{1}{2}})
	\end{align*}
	
	We have
	\begin{align*}
	\log\det(D^{1})-\log\det(D^{0}) & =\log\det((D^{0})^{-\frac{1}{2}}(D^{1}-D^{0})(D^{0})^{-\frac{1}{2}})+I)\\
	& \leq Tr((D^{0})^{-\frac{1}{2}}(D^{1}-D^{0})(D^{0})^{-\frac{1}{2}}))
	\end{align*}
	Similarly, 
	\begin{align*}
	\log\det(M-D^{1})-\log\det(M-D^{0}) & =\log\det((M-D^{0})^{-\frac{1}{2}}((M-D^{1})-(M-D^{0}))(M-D^{0})^{-\frac{1}{2}}+I)\\
	& \leq Tr((M-D^{0})^{-\frac{1}{2}}(D^{0}-D^{1})(M-D^{0})^{-\frac{1}{2}}))
	\end{align*}
	and 
	\begin{align*}
	\log\det(\kappa^{1}D^{1}-M)-\log\det(\kappa^{0}D^{0}-M) & =\log\det((\kappa^{0}D^{0}-M)^{-\frac{1}{2}}((\kappa^{1}D^{1}-M)-(\kappa^{0}D^{0}-M))(\kappa^{0}D^{0}-M)^{-\frac{1}{2}}+I)\\
	& \leq Tr((\kappa^{0}D^{0}-M)^{-\frac{1}{2}}(\kappa^{1}D^{1}-\kappa^{0}D^{0})(\kappa^{0}D^{0}-M)^{-\frac{1}{2}})
	\end{align*}
	Summing up the three inequalities, and using the KKT condition of
	the max-potential at $\kappa_{0}$, i.e. 
	\begin{align*}
	-(M-D^{0})^{-1}+\kappa^{0}(\kappa^{0}D^{0}-M)^{-1}+(D^{0})^{-1} & =0
	\end{align*}
	we have 
	\begin{align*}
	P(\kappa^{1})-P(\kappa^{0}) & \leq Tr((\kappa^{0}D^{0}-M)^{-\frac{1}{2}}(\kappa^{1}D^{1}-\kappa^{0}D^{1})(\kappa^{0}D^{0}-M)^{-\frac{1}{2}})\\
	& =-\Delta\kappa\cdot Tr((\kappa^{0}D^{0}-M)^{-\frac{1}{2}}D^{1}(\kappa^{0}D^{0}-M)^{-\frac{1}{2}})
	\end{align*}
	It remains to bound the quantity 
	\begin{align*}
	\Delta\kappa\cdot Tr((\kappa^{0}D^{0}-M)^{-\frac{1}{2}}D^{1}(\kappa^{0}D^{0}-M)^{-\frac{1}{2}})
	\end{align*}
	from below. First notice that 
	\begin{align*}
	\Delta\kappa\cdot Tr((\kappa^{0}D^{0}-M)^{-\frac{1}{2}}D^{1}(\kappa^{0}D^{0}-M)^{-\frac{1}{2}}) & =\Delta\kappa\cdot Tr((\kappa^{0}D^{0}-M)^{-1}D^{1})\\
	& =\Delta\kappa\cdot e^{T}D^{1}\text{diag}((\kappa^{0}D^{0}-M)^{-1})e
	\end{align*}
	Moreover, since by assumption $\Delta\kappa=\frac{\beta}{e^{T}D^{0}\text{diag}((\kappa^{0}D^{0}-M)^{-1})e}$,
	we have 
	\begin{align*}
	\Delta\kappa\cdot Tr((\kappa^{0}D^{0}-M)^{-\frac{1}{2}}D^{1}(\kappa^{0}D^{0}-M)^{-\frac{1}{2}}) & \geq\beta\cdot\frac{e^{T}D^{1}\text{diag}((\kappa^{0}D^{0}-M)^{-1})e}{e^{T}D^{0}\text{diag}((\kappa^{0}D^{0}-M)^{-1})e}\\
	& \geq\Omega(n)
	\end{align*}
	where the last inequality follows from 
	\begin{align*}
	e^{T}D^{1}\text{diag}((\kappa^{0}D^{0}-M)^{-1})e & =\sum_{i}D_{ii}^{1}\text{diag}((\kappa^{0}D^{0}-M)^{-1})_{ii}\\
	& \geq\Omega(n)\sum_{i}D_{ii}^{0}\text{diag}((\kappa^{0}D^{0}-M)^{-1})_{ii}\\
	& =\Omega(n)e^{T}D^{0}\text{diag}((\kappa^{0}D^{0}-M)^{-1})e
	\end{align*}
	and the inequality
	\begin{align*}
	Tr(D^{1}(D^{0})^{-1}) & \leq O(n)\\
	Tr(D^{0}(D^{1})^{-1}) & \leq O(n)
	\end{align*}
	which we now prove.
	
	Note that 
	\begin{align*}
	\|D^{\ast}D^{-1}-e\|\\
	\end{align*}
	
	\begin{align*}
	\overline{Z}^{l+1}\overline{y}^{l} & =\overline{Z}^{l}\overline{y}^{l}+\Delta Z\overline{y}^{l}\\
	& =e-\overline{Z}^{l}\Delta y
	\end{align*}
	so that 
	\begin{align*}
	\|(\overline{Y}^{l})^{-1}(\overline{y}^{l+1}-\overline{y}^{l})\| & =\|(\overline{Y}^{l})^{-1}(\overline{Z}^{l})^{-1}-\overline{Z}^{l+1}(\overline{Z}^{l})^{-1}\|\\
	& =\|(\overline{Y}^{l})^{-1}(\overline{Z}^{l})^{-1}+e-\Delta z(\overline{Z}^{l})^{-1}\|
	\end{align*}
	\end{proof}
	\end{comment}
	
	\begin{comment}
	\begin{proof}
	We have 
	\begin{align*}
	\frac{\exp(P(\kappa^{1}))}{\exp(P(\kappa^{0}))} & =\prod_{i}\frac{\lambda_{i}(M-D^{1})}{\lambda_{i}(M-D^{0})}\cdot\prod_{i}\frac{\lambda_{i}(\kappa^{1}D^{1}-M)}{\lambda_{i}(\kappa^{0}D^{0}-M)}\cdot\prod_{i}\frac{\lambda_{i}(D^{1})}{\lambda_{i}(D^{0})}\\
	& =\prod_{i}\lambda_{i}(M-D^{1})\cdot\lambda_{n-i}(X^{0})\cdot\prod_{i}\lambda_{i}(\kappa^{1}D^{1}-M)\cdot\lambda_{n-i}(Y^{0})\cdot\prod_{i}\lambda_{i}(D^{1})\cdot\lambda_{n-i}(Z^{0})\\
	& \leq\left(\frac{\sum_{i}\lambda_{i}(M-D^{1})\cdot\lambda_{n-i}(X^{0})+\sum_{i}\lambda_{i}(\kappa^{1}D^{1}-M)\cdot\lambda_{n-i}(Y^{0})+\sum_{i}\lambda_{i}(D^{1})\cdot\lambda_{n-i}(Z^{0})}{3n}\right)^{3n}
	\end{align*}
	
	We claim that the numerator is bounded above by $3n-\Delta\kappa\sum_{i}\lambda_{i}(D^{1})\cdot\lambda_{n-i}(Y^{0})$,
	so that we have 
	\begin{align*}
	\frac{\exp(P(\kappa^{1}))}{\exp(P(\kappa^{0}))} & \leq\left(\frac{3n-\Delta\kappa\sum_{i}\lambda_{i}(D^{1})\cdot\lambda_{n-i}(Y^{0})}{3n}\right)^{3n}\\
	& =\left(1-\frac{\Delta\kappa\sum_{i}\lambda_{i}(D^{1})\cdot\lambda_{n-i}(Y^{0})}{3n}\right)^{3n}\\
	& \leq\exp(-\Delta\kappa\sum_{i}\lambda_{i}(D^{1})\cdot\lambda_{n-i}(Y^{0}))
	\end{align*}
	since 
	\begin{align*}
	\Delta\kappa\sum_{i}\lambda_{i}(D^{1})\cdot\lambda_{n-i}(Y^{0}) & =\beta\frac{1}{\sum_{i}\lambda_{i}(D^{0})\cdot\lambda_{n-i}(Y^{0})}\cdot\sum_{i}\lambda_{i}(D^{1})\cdot\lambda_{n-i}(Y^{0})\\
	& \geq\beta
	\end{align*}
	this implies 
	\begin{align*}
	P(\kappa^{1}) & \leq P(\kappa^{0})-\Omega(1)
	\end{align*}
	
	Use 
	
	To prove the claimed bound, we use Weyl's inequality, which states
	that 
	\begin{align*}
	\lambda_{i}(A+B) & \leq\lambda_{i}(A)+\lambda_{1}(B)
	\end{align*}
	Applying this bound, and using the first order condition 
	\begin{align*}
	Z^{0}e+\kappa Y^{0}e & =X^{0}e
	\end{align*}
	we have
	
	\begin{align*}
	\sum_{i}\lambda_{i}(M-D^{1})\cdot\lambda_{n-i+1}(X^{0})+\sum_{i}\lambda_{i}(\kappa^{1}D^{1}-M)\cdot\lambda_{n-i+1}(Y^{0})+\sum_{i}\lambda_{i}(D^{1})\cdot\lambda_{n-i+1}(Z^{0}) & \leq\\
	\sum_{i}(\lambda_{i}(M-D^{0})+\lambda_{1}(D^{0}-D^{1}))\cdot\lambda_{n-i+1}(X^{0})+\sum_{i}(\lambda_{i}(\kappa^{0}D^{0}-M)+\lambda_{1}(\kappa^{1}D^{1}-\kappa^{0}D^{0}))\cdot\lambda_{n-i+1}(Y^{0})+\\
	\sum_{i}(\lambda_{i}(D^{0})+\lambda_{1}(D^{1}-D^{0}))\cdot\lambda_{n-i+1}(Z^{0}) & =\\
	3n+\sum_{i}\lambda_{1}(D^{0}-D^{1})\cdot\lambda_{n-i+1}(X^{0})+\sum_{i}\lambda_{1}(\kappa^{1}D^{1}-\kappa^{0}D^{0})\cdot\lambda_{n-i+1}(Y^{0})+\sum_{i}\lambda_{1}(D^{1}-D^{0})\cdot\lambda_{n-i+1}(Z^{0}) & =\\
	3n+\sum_{i}\lambda_{1}(D^{0}-D^{1})\cdot\lambda_{n-i+1}(X^{0})+\sum_{i}\lambda_{1}(\kappa^{1}D^{1}-\kappa^{0}D^{1}+\kappa^{0}D^{1}-\kappa^{0}D^{0})\cdot\lambda_{n-i+1}(Y^{0})+\sum_{i}\lambda_{1}(D^{1}-D^{0})\cdot\lambda_{n-i+1}(Z^{0}) & \leq\\
	3n+\sum_{i}\lambda_{1}(D^{0}-D^{1})\cdot\lambda_{n-i+1}(X^{0})+\sum_{i}\lambda_{1}(\kappa^{1}D^{1}-\kappa^{0}D^{1})\cdot\lambda_{n-i+1}(Y^{0})+\sum_{i}\lambda_{1}(\kappa^{0}D^{1}-\kappa^{0}D^{0})\cdot\lambda_{n-i+1}(Y^{0})+\sum_{i}\lambda_{1}(D^{1}-D^{0})\cdot\lambda_{n-i+1}(Z^{0}) & =\\
	3n+\sum_{i}\lambda_{1}(D^{0}-D^{1})\cdot\lambda_{n-i+1}(X^{0})+\sum_{i}\lambda_{1}(-\Delta\kappa\cdot D^{1})\cdot\lambda_{n-i+1}(Y^{0})+\sum_{i}\lambda_{1}(D^{1}-D^{0})\cdot\lambda_{n-i+1}(\kappa^{0}Y^{0})+\sum_{i}\lambda_{1}(D^{1}-D^{0})\cdot\lambda_{n-i+1}(Z^{0}) & =\\
	3n+\sum_{i}\lambda_{1}(D^{0}-D^{1})\cdot\lambda_{n-i+1}(X^{0})+\sum_{i}\lambda_{1}(-\Delta\kappa\cdot D^{1})\cdot\lambda_{n-i+1}(Y^{0})+\sum_{i}\lambda_{1}(D^{1}-D^{0})\cdot\lambda_{n-i+1}(X^{0}) & \leq\\
	3n-\Delta\kappa\cdot\sum_{i}\lambda_{n}(D^{1})\cdot\lambda_{n-i+1}(Y^{0})+(\lambda_{1}(D^{1}-D^{0})-\lambda_{n}(D^{1}-D^{0}))\cdot Tr((M-D^{0})^{-1})
	\end{align*}
	\end{proof}
	\end{comment}
	\hfill \halmos
\endproof
%
\begin{proposition}

	Let $D^{0}$ be the exact analytic center of $\kappa^{0}$. Define
	$R_{0}=M-D_{0}$, $S_{0}=\kappa_{0}D_{0}-M$ and $X_{0}=R_{0}^{-1},Y_{0}=S_{0}^{-1},Z_{0}=D_{0}^{-1}$.	Further, let $\Delta\kappa=\kappa^{0}-\kappa^{1}$ with $\Delta\kappa=\frac{\beta}{Tr(D^{0}\cdot(\kappa^{0}D^{0}-M)^{-1})}$
	where $\beta\in(0,1)$ is a sufficiently small constant, and 
	\begin{align*}
	\overline{R}^{0} & =R^{0},\overline{S}^{0}=-\Delta\kappa D^{0}+S^{0},\overline{D}^{0}=D^{0}\\
	\overline{X}^{0} & =X^{0},\overline{Y}^{0}=Y^{0},\overline{Z}^{0}=\Delta\kappa Y^{0}+Z^{0}
	\end{align*}
	Then, the new variables satisfy 
	\begin{align*}
	\overline{R}^{0} & =M-\overline{D}^{0}\succeq0\\
	\overline{S}^{0} & =\kappa^{1}\overline{D}^{0}-M\succeq0\\
	\overline{D}^{0} & \succeq0
	\end{align*}
	and $\overline{Z}^{0}+\kappa^{1}\overline{Y}^{0}=\overline{X}^{0}$.
	Moreover, $\delta(\overline{S}^{0},\overline{Y}^{0})\leq\beta,\delta(\overline{D}^{0},\overline{Z}^{0})\leq\beta,\delta(\overline{R}^{0},\overline{X}^{0})=0$.
\end{proposition}
\proof{Proof}
	We can readily verify that the new variables satisfy the desired equalities.
	When $\Delta\kappa$ is appropriately chosen as in the previous theorem,
	we can guarantee that $\overline{S}^{0}\succeq0$. Now 
	\begin{align*}
	\delta(\overline{S}^{0},\overline{Y}^{0})^{2}=Tr((\overline{S}^{0}\overline{Y}^{0}-I)^{2}) & =Tr((-\Delta\kappa D^{0}+S^{0})Y^{0}-I)^{2}\\
	& =Tr(-\Delta\kappa D^{0}Y^{0})^{2}\\
	& =Tr(-\Delta\kappa D^{0}(\kappa_{0}D_{0}-M)^{-1})^{2}\\
	& \leq(Tr(-\Delta\kappa D^{0}(\kappa_{0}D_{0}-M)^{-1}))^{2}=\beta^{2}
	\end{align*}
	where we have used $Tr(A^{2})=(TrA)^{2}-2\sigma_{2}(A)$ where $\sigma_{2}(A)=\sum_{i<j}\lambda_{i}\lambda_{j}$
	and $\lambda_{i}$ are the eigenvalues of $A$. Therefore, $\delta(\overline{S}^{0},\overline{Y}^{0})\leq\beta$.
	Similarly, $\delta(\overline{D}^{0},\overline{Z}^{0})\leq\beta$ and
	since $\overline{R}^{0}=R^{0},\overline{X}^{0}=X^{0}$, we have $\delta(\overline{D}^{0},\overline{Z}^{0})=0$
	\hfill \halmos
\endproof
%
\begin{proposition}
Let $(\overline{R}^{0},\overline{S}^{0},\overline{D}^{0},\overline{X}^{0},\overline{Y}^{0},\overline{Z}^{0})$
	be any set that satisfy 
	\begin{align*}
	\overline{R}^{0} & =M-\overline{D}^{0}\succeq0\\
	\overline{S}^{0} & =\kappa^{1}\overline{D}^{0}-M\succeq0\\
	\overline{D}^{0} & \succeq0
	\end{align*}
	and 
	\begin{align*}
	\overline{Z}^{0}+\kappa^{1}\overline{Y}^{0} & =\overline{X}^{0}
	\end{align*}
	with 
	\begin{align*}
	\delta(\overline{R}^{0},\overline{X}^{0})=\|(\overline{R}^{0})^{\frac{1}{2}}\overline{X}^{0}(\overline{R}^{0})^{\frac{1}{2}}-I\|_{F} & \leq\beta\\
	\delta(\overline{D}^{0},\overline{Z}^{0})=\|(\overline{D}^{0})^{\frac{1}{2}}\overline{Z}^{0}(\overline{D}^{0})^{\frac{1}{2}}-I\|_{F} & \leq\beta\\
	\delta(\overline{S}^{0},\overline{Y}^{0})=\|(\overline{S}^{0})^{\frac{1}{2}}\overline{Y}^{0}(\overline{S}^{0})^{\frac{1}{2}}-I\|_{F} & \leq\beta
	\end{align*}
	for any $\beta\in(0,1)$. 
	
	Let $X^{1},Y^{1},Z^{1},R^{1},S^{1},D^{1}$ be defined by 
	\begin{align*}
	X^{1} & =\overline{X}^{0}+\Delta X\\
	Y^{1} & =\overline{Y}^{0}+\Delta Y\\
	Z^{1} & =\overline{Z}^{0}+\Delta Z\\
	R^{1} & =\overline{R}^{0}+\Delta R\\
	S^{1} & =\overline{S}^{0}+\Delta S\\
	D^{1} & =\overline{D}^{0}+\Delta D
	\end{align*}
	where the increments $\Delta$s are given by the Newton step %
	\begin{comment}
	The Newton step is to ensure 
	\begin{align*}
	\overline{R}^{0} & =M-\overline{D}^{0}\succeq0\\
	\overline{S}^{0} & =\kappa^{1}\overline{D}^{0}-M\succeq0\\
	\overline{D}^{0} & \succeq0
	\end{align*}
	and 
	\begin{align*}
	\overline{Z}^{0}+\kappa^{1}\overline{Y}^{0} & =\overline{X}^{0}
	\end{align*}
	still holds. 
	
	Regular Newton step is
	
	\begin{align*}
	\overline{D}^{0}\cdot\Delta Z+\overline{Z}^{0}\cdot\Delta D & =I-\overline{D}^{0}\cdot\overline{Z}^{0}\\
	\overline{R}^{0}\cdot\Delta X+\overline{X}^{0}\cdot\Delta R & =I-\overline{R}^{0}\cdot\overline{X}^{0}\\
	\overline{S}^{0}\cdot\Delta Y+\overline{Y}^{0}\cdot\Delta S & =I-\overline{S}^{0}\cdot\overline{Y}^{0}
	\end{align*}
	but here we need to use the Nesterov-Todd direction to ensure symmetry
	of updates. 
	\end{comment}
	\begin{align*}
	\Delta Z+W^{-1}\Delta DW^{-1} & =(\overline{D}^{0})^{-1}-\overline{Z}^{0}\\
	\Delta X+U^{-1}\Delta RU^{-1} & =(\overline{R}^{0})^{-1}-\overline{X}^{0}\\
	\Delta Y+V^{-1}\Delta S & V^{-1}=(\overline{S}^{0})^{-1}-\overline{Y}^{0}
	\end{align*}
	{} and 
	\begin{align*}
	\Delta R & =-\Delta D\\
	\Delta S & =\kappa^{1}\Delta D\\
	\Delta Z+\kappa^{1}\Delta Y & =\Delta X
	\end{align*}
	where $U,V,W$ are the geometric means 
	\begin{align*}
	U & =(\overline{R}^{0})^{1/2}((\overline{R}^{0})^{1/2}\overline{X}^{0}(\overline{R}^{0})^{1/2})^{-1/2}(\overline{R}^{0})^{1/2}\\
	V & =(\overline{S}^{0})^{1/2}((\overline{S}^{0})^{1/2}\overline{Y}^{0}(\overline{S}^{0})^{1/2})^{-1/2}(\overline{S}^{0})^{1/2}\\
	W & =(\overline{D}^{0})^{1/2}((\overline{D}^{0})^{1/2}\overline{Z}^{0}(\overline{D}^{0})^{1/2})^{-1/2}(\overline{D}^{0})^{1/2}
	\end{align*}
	to ensure that updates $\Delta$s are symmetric.
	
	Then we have 
	\begin{align*}
	\delta(R^{1},X^{1})=\|(R^{1})^{\frac{1}{2}}X^{1}(R^{1})^{\frac{1}{2}}-I\|_{F} & \leq\frac{1}{2}\frac{\beta^{2}}{1-\beta}\\
	\delta(S^{1},Y^{1})=\|(S^{1})^{\frac{1}{2}}Y^{1}(S^{1})^{\frac{1}{2}}-I\|_{F} & \leq\frac{1}{2}\frac{\beta^{2}}{1-\beta}\\
	\delta(D^{1},Z^{1})=\|(D^{1})^{\frac{1}{2}}Z^{1}(D^{1})^{\frac{1}{2}}-I\|_{F} & \leq\frac{1}{2}\frac{\beta^{2}}{1-\beta}
	\end{align*}
	and 
	\begin{align*}
	\|(\overline{D}^{0})^{-\frac{1}{2}}D^{1}(\overline{D}^{0})^{-\frac{1}{2}}-I\|_{F} & \le\frac{\beta}{1-\beta}
	\end{align*}
\end{proposition}
\proof{Proof}
	First observe that the Newton system has a unique solution. To see
	this, note that we can eliminate $\Delta X,\Delta Y,\Delta Z$ using
	$\Delta Z+\kappa^{1}\Delta Y=\Delta X$. Then using
	\begin{align*}
	\Delta R & =-\Delta D\\
	\Delta S & =\kappa^{1}\Delta D
	\end{align*}
	we can uniquely solve for $\Delta D$, from which all other increments
	can be uniquely determined. 
	
	We have 
	\begin{align*}
	\delta(D^{1},Z^{1})^{2}=\|(Z^{1})^{\frac{1}{2}}D^{1}(Z^{1})^{\frac{1}{2}}-I\|_{F}^{2} & =Tr(((Z^{1})^{\frac{1}{2}}D^{1}(Z^{1})^{\frac{1}{2}}-I)^{2})\\
	& =Tr((Z^{1})D^{1}(Z^{1})D^{1})-2Tr(Z^{1}D^{1})+Tr(I)\\
	& =Tr((D^{1}Z^{1}-I)^{2})\\
	& \leq\left(Tr(D^{1}Z^{1}-I)\right)^{2}
	\end{align*}
	where we have used $Tr(A^{2})=(TrA)^{2}-2\sigma_{2}(A)$ where 
	\begin{align*}
	\sigma_{2}(A) & =\sum_{i<j}\lambda_{i}\lambda_{j}
	\end{align*}
	and $\lambda_{i}$ are the eigenvalues of $A$. 
	
	The Newton update formula 
	\begin{align*}
	\Delta Z+W^{-1}\Delta DW^{-1} & =(\overline{D}^{0})^{-1}-\overline{Z}^{0}\\
	Z^{1} & =Z^{0}+\Delta Z\\
	D^{1} & =D^{0}+\Delta D
	\end{align*}
	and 
	\begin{align*}
	W & =(\overline{D}^{0})^{1/2}((\overline{D}^{0})^{1/2}\overline{Z}^{0}(\overline{D}^{0})^{1/2})^{-1/2}(\overline{D}^{0})^{1/2}
	\end{align*}
	imply
	
	\begin{align*}
	Tr(D^{1}Z^{1}-I) & =Tr((\overline{D}^{0}+\Delta D)(\overline{Z}^{0}+\Delta Z)-I)\\
	& =Tr(\overline{D}^{0}\overline{Z}^{0}+\Delta D\overline{Z}^{0}+\overline{D}^{0}\Delta Z+\Delta D\Delta Z-I)\\
	& =Tr(-\overline{D}^{0}W^{-1}\Delta DW^{-1}+\Delta D\overline{Z}^{0}+\Delta D\Delta Z)\\
	& =Tr(-(\overline{D}^{0})^{1/2}\overline{Z}^{0}(\overline{D}^{0})^{1/2}(\overline{D}^{0})^{-1/2}\Delta D(\overline{D}^{0})^{-1/2}+\Delta D\overline{Z}^{0}+\Delta D\Delta Z)\\
	& =Tr(-\Delta D\overline{Z}^{0}+\Delta D\overline{Z}^{0}+\Delta D\Delta Z)\\
	& =Tr(\Delta D\Delta Z)
	\end{align*}
	So that 
	\begin{align*}
	\delta(D^{1},Z^{1}) & \leq Tr(\Delta D\Delta Z)
	\end{align*}
	and similarly 
	\begin{align*}
	\delta(R^{1},X^{1}) & \leq Tr(\Delta R\Delta X)\\
	\delta(S^{1},Y^{1}) & \leq Tr(\Delta S\Delta Y)
	\end{align*}
	
	Multiplying both sides of
	\begin{align*}
	\Delta Z+W^{-1}\Delta DW^{-1} & =(\overline{D}^{0})^{-1}-\overline{Z}^{0}
	\end{align*}
	by $W^{\frac{1}{2}}$ on the left and on the right we have
	\begin{align*}
	W^{\frac{1}{2}}\Delta ZW^{\frac{1}{2}}+W^{-\frac{1}{2}}\Delta DW^{-\frac{1}{2}} & =W^{\frac{1}{2}}(\overline{D}^{0})^{-1}W^{\frac{1}{2}}-W^{\frac{1}{2}}\overline{Z}^{0}W^{\frac{1}{2}}
	\end{align*}
	Then squaring and taking the trace, 
	\begin{align*}
	Tr(W^{\frac{1}{2}}\Delta ZW^{\frac{1}{2}}+W^{-\frac{1}{2}}\Delta DW^{-\frac{1}{2}})^{2} & =Tr(W^{\frac{1}{2}}(\overline{D}^{0})^{-1}W^{\frac{1}{2}}-W^{\frac{1}{2}}\overline{Z}^{0}W^{\frac{1}{2}})^{2}
	\end{align*}
	and the left hand side is equal to 
	\begin{align*}
	Tr(W^{\frac{1}{2}}\Delta ZW^{\frac{1}{2}}+W^{-\frac{1}{2}}\Delta DW^{-\frac{1}{2}})^{2} & =Tr(W^{\frac{1}{2}}\Delta ZW^{\frac{1}{2}})^{2}+Tr(W^{-\frac{1}{2}}\Delta DW^{-\frac{1}{2}})^{2}\\
	& +Tr(\Delta Z\Delta D)+Tr(\Delta D\Delta Z)
	\end{align*}
	So we have 
	\begin{align*}
	2Tr(\Delta Z\Delta D) & \leq Tr(W^{\frac{1}{2}}(\overline{D}^{0})^{-1}W^{\frac{1}{2}}-W^{\frac{1}{2}}\overline{Z}^{0}W^{\frac{1}{2}})^{2}
	\end{align*}
	Now we calculate the right hand side. Using
	\begin{align*}
	W & =(\overline{D}^{0})^{1/2}((\overline{D}^{0})^{1/2}\overline{Z}^{0}(\overline{D}^{0})^{1/2})^{-1/2}(\overline{D}^{0})^{1/2}\\
	& =(\overline{Z}^{0})^{-1/2}((\overline{Z}^{0})^{1/2}\overline{D}^{0}(\overline{Z}^{0})^{1/2})^{1/2}(\overline{Z}^{0})^{-1/2}
	\end{align*}
	we get 
	\begin{align*}
	Tr(W^{\frac{1}{2}}(\overline{D}^{0})^{-1}W^{\frac{1}{2}})^{2} & =Tr(\overline{D}^{0})^{1/2}((\overline{D}^{0})^{1/2}\overline{Z}^{0}(\overline{D}^{0})^{1/2})^{-1}(\overline{D}^{0})^{1/2}(\overline{D}^{0})^{-1}\\
	& =Tr(\overline{Z}^{0})^{-1}(\overline{D}^{0})^{-1}\\
	Tr(W^{\frac{1}{2}}\overline{Z}^{0}W^{\frac{1}{2}})^{2} & =Tr(\overline{Z}^{0})^{-1/2}((\overline{Z}^{0})^{1/2}\overline{D}^{0}(\overline{Z}^{0})^{1/2})^{1}(\overline{Z}^{0})^{-1/2}\overline{Z}^{0}\\
	& =Tr\overline{D}^{0}\overline{Z}^{0}\\
	Tr(W^{\frac{1}{2}}(\overline{D}^{0})^{-1}W^{\frac{1}{2}})(W^{\frac{1}{2}}\overline{Z}^{0}W^{\frac{1}{2}}) & =Tr(I)\\
	Tr(W^{\frac{1}{2}}\overline{Z}^{0}W^{\frac{1}{2}})(W^{\frac{1}{2}}(\overline{D}^{0})^{-1}W^{\frac{1}{2}}) & =Tr(I)
	\end{align*}
	so that %
	\begin{comment}
	\begin{align*}
	Tr(W^{\frac{1}{2}}(\overline{D}^{0})^{-1}W^{\frac{1}{2}}-W^{\frac{1}{2}}\overline{Z}^{0}W^{\frac{1}{2}})^{2} & =Tr(\overline{Z}^{0})^{-1}(\overline{D}^{0})^{-1}+Tr\overline{D}^{0}\overline{Z}^{0}+2Tr(I)\\
	& =\frac{1}{2}Tr((\overline{Z}^{0})^{-1}(\overline{D}^{0})^{-1}(I-2\overline{D}^{0}\overline{Z}^{0}+\overline{D}^{0}\overline{Z}^{0}\overline{Z}^{0}\overline{D}^{0}))\\
	& +\frac{1}{2}Tr((\overline{D}^{0})^{-1}(\overline{Z}^{0})^{-1}(I-2\overline{Z}^{0}\overline{D}^{0}+\overline{Z}^{0}\overline{D}^{0}\overline{D}^{0}\overline{Z}^{0}))\\
	& =Tr((I-\overline{Z}^{0}\overline{D}^{0})(\overline{D}^{0}\overline{Z}^{0})^{-1}(I-\overline{D}^{0}\overline{Z}^{0}))\\
	& =\\
	& =Tr((\overline{D}^{0}\overline{Z}^{0})^{-\frac{1}{2}}(I-\overline{D}^{0}\cdot\overline{Z}^{0}))^{T}((\overline{D}^{0}\overline{Z}^{0})^{-\frac{1}{2}}(I-\overline{D}^{0}\cdot\overline{Z}^{0}))
	\end{align*}
	\end{comment}
	
	\begin{align*}
	Tr(W^{\frac{1}{2}}(\overline{D}^{0})^{-1}W^{\frac{1}{2}}-W^{\frac{1}{2}}\overline{Z}^{0}W^{\frac{1}{2}})^{2} & =Tr(\overline{Z}^{0})^{-1}(\overline{D}^{0})^{-1}+Tr\overline{D}^{0}\overline{Z}^{0}+2Tr(I)\\
	& =Tr((\overline{D}^{0})^{-1/2}(\overline{Z}^{0})^{-1}(\overline{D}^{0})^{-1/2}(I-2(\overline{D}^{0})^{1/2}\overline{Z}^{0}(\overline{D}^{0})^{1/2}+((\overline{D}^{0})^{1/2}\overline{Z}^{0}(\overline{D}^{0})^{1/2})^{2}))\\
	& =Tr((\overline{D}^{0})^{-1/2}(\overline{Z}^{0})^{-1}(\overline{D}^{0})^{-1/2}(I-(\overline{D}^{0})^{1/2}\overline{Z}^{0}(\overline{D}^{0})^{1/2})^{2})
	\end{align*}
	
	Now recall that 
	\begin{align*}
	\delta(\overline{D}^{0},\overline{Z}^{0})=\|(\overline{D}^{0})^{\frac{1}{2}}\overline{Z}^{0}(\overline{D}^{0})^{\frac{1}{2}}-I\|_{F} & \leq\beta
	\end{align*}
	and so 
	\begin{align*}
	Tr((I-(\overline{D}^{0})^{1/2}\overline{Z}^{0}(\overline{D}^{0})^{1/2})^{2}) & =\|(\overline{D}^{0})^{1/2}\overline{Z}^{0}(\overline{D}^{0})^{1/2}-I\|_{F}^{2}\\
	& =\delta(\overline{D}^{0},\overline{Z}^{0})^{2}\leq\beta^{2}
	\end{align*}
	and Holder's inequality yields 
	\begin{align*}
	Tr((\overline{D}^{0})^{-1/2}(\overline{Z}^{0})^{-1}(\overline{D}^{0})^{-1/2}(I-(\overline{D}^{0})^{1/2}\overline{Z}^{0}(\overline{D}^{0})^{1/2})^{2}) & \leq\lambda_{1}((\overline{D}^{0})^{-1/2}(\overline{Z}^{0})^{-1}(\overline{D}^{0})^{-1/2})\cdot Tr(I-(\overline{D}^{0})^{1/2}\overline{Z}^{0}(\overline{D}^{0})^{1/2})^{2})\\
	& \leq\lambda_{1}((\overline{Z}^{0})^{-1}(\overline{D}^{0})^{-1})\beta^{2}
	\end{align*}
	Recall the eigenvalue stability result 
	\begin{align*}
	|\lambda_{i}(X)-\lambda_{i}(Y)| & \leq\|X-Y\|_{op}
	\end{align*}
	for symmetric positive definite matrices $X,Y$ and again using 
	\begin{align*}
	\|(\overline{D}^{0})^{1/2}\overline{Z}^{0}(\overline{D}^{0})^{1/2}-I\|_{F} & =\|\overline{D}^{0}\overline{Z}^{0}-I\|_{F}\\
	& =\sqrt{Tr(\overline{D}^{0}\overline{Z}^{0}-I)^{T}(\overline{D}^{0}\overline{Z}^{0}-I)}\leq\beta
	\end{align*}
	and the inequality 
	\begin{align*}
	\|X\|_{op} & \leq\|X\|_{F}
	\end{align*}
	between operator norm and Frobenius norm, we have 
	\begin{align*}
	|\lambda_{n}((\overline{D}^{0})^{1/2}\overline{Z}^{0}(\overline{D}^{0})^{1/2})-1| & =|\lambda_{n}((\overline{D}^{0})^{1/2}\overline{Z}^{0}(\overline{D}^{0})^{1/2})-\lambda_{n}(I)|\\
	& \leq\|(\overline{D}^{0})^{1/2}\overline{Z}^{0}(\overline{D}^{0})^{1/2}-I\|_{op}\leq\|(\overline{D}^{0})^{1/2}\overline{Z}^{0}(\overline{D}^{0})^{1/2}-I\|_{F}\leq\beta
	\end{align*}
	so that 
	\begin{align*}
	\lambda_{n}((\overline{D}^{0})^{1/2}\overline{Z}^{0}(\overline{D}^{0})^{1/2}) & \geq1-\beta
	\end{align*}
	and 
	\begin{align*}
	\lambda_{1}((\overline{D}^{0})^{-1/2}(\overline{Z}^{0})^{-1}(\overline{D}^{0})^{-1/2}) & =\frac{1}{\lambda_{n}((\overline{D}^{0})^{1/2}\overline{Z}^{0}(\overline{D}^{0})^{1/2})}\leq\frac{1}{1-\beta}
	\end{align*}
	This allows us to finally conclude that 
	\begin{align*}
	Tr(\Delta Z\Delta D) & \leq\frac{1}{2}\frac{\beta^{2}}{1-\beta}
	\end{align*}
	and so 
	\begin{align*}
	\delta(D^{1},Z^{1}) & \leq Tr(\Delta Z\Delta D)\\
	& \leq\frac{1}{2}\frac{\beta^{2}}{1-\beta}
	\end{align*}
	The same argument applied to $(R^{1},X^{1})$, $(S^{1},Y^{1})$ gives
	\begin{align*}
	\delta(R^{1},X^{1}) & \leq\frac{1}{2}\frac{\beta^{2}}{1-\beta}\\
	\delta(S^{1},Y^{1}) & \leq\frac{1}{2}\frac{\beta^{2}}{1-\beta}
	\end{align*}
	
	Now we show that 
	\begin{align*}
	\|(\overline{D}^{0})^{-\frac{1}{2}}D^{1}(\overline{D}^{0})^{-\frac{1}{2}}-I\|_{F} & \le\frac{\beta}{1-\beta}
	\end{align*}
	Note 
	\begin{align*}
	\|(\overline{D}^{0})^{-\frac{1}{2}}D^{1}(\overline{D}^{0})^{-\frac{1}{2}}-I\|_{F}^{2} & =Tr(((\overline{D}^{0})^{-\frac{1}{2}}D^{1}(\overline{D}^{0})^{-\frac{1}{2}}-I)^{2})\\
	& =Tr(((\overline{D}^{0})^{-1}(D^{1}-\overline{D}^{0})(\overline{D}^{0})^{-1}(D^{1}-\overline{D}^{0})\\
	& =Tr((\overline{D}^{0})^{-1}\Delta D(\overline{D}^{0})^{-1}\Delta D)
	\end{align*}
	Now multiplying both sides of 
	\begin{align*}
	W\Delta ZW+\Delta D=(\overline{Z}^{0})^{-1}-\overline{D}^{0}
	\end{align*}
	by $(\overline{D}^{0})^{-\frac{1}{2}}$, we have 
	\begin{align*}
	Tr(((\overline{D}^{0})^{-1}\Delta D)^{2}) & \leq Tr(((\overline{D}^{0})^{-1}(\overline{Z}^{0})^{-1}-I))^{2})\\
	& =\|(\overline{D}^{0})^{-\frac{1}{2}}(\overline{Z}^{0})^{-1}(\overline{D}^{0})^{-\frac{1}{2}}-I\|_{F}^{2}\\
	& =\|(I-(\overline{D}^{0})^{\frac{1}{2}}(\overline{Z}^{0})(\overline{D}^{0})^{\frac{1}{2}})((\overline{D}^{0})^{-\frac{1}{2}}(\overline{Z}^{0})^{-1}(\overline{D}^{0})^{-\frac{1}{2}})\|_{F}^{2}\\
	& \leq Tr((I-(\overline{D}^{0})^{\frac{1}{2}}(\overline{Z}^{0})(\overline{D}^{0})^{\frac{1}{2}})^{2})\lambda_{1}(((\overline{D}^{0})^{-\frac{1}{2}}(\overline{Z}^{0})^{-1}(\overline{D}^{0})^{-\frac{1}{2}})^{2})\\
	& \leq\beta^{2}/(1-\beta)^{2}
	\end{align*}
	as desired. 
	
	\begin{comment}
	\begin{proof}
	\begin{align*}
	W\Delta Z+\Delta DW^{-1} & =W(\overline{D}^{0})^{-1}-W\overline{Z}^{0}
	\end{align*}
	and by $W$ on the right we get
	\begin{align*}
	\Delta ZW+W^{-1}\Delta D & =(\overline{D}^{0})^{-1}W-\overline{Z}^{0}W
	\end{align*}
	
	$\overline{D}^{0}\cdot\Delta Z+\Delta D\cdot\overline{Z}^{0}=I-\overline{D}^{0}\cdot\overline{Z}^{0}$
	by $(\overline{D}^{0}\overline{Z}^{0})^{-\frac{1}{2}}$, we have
	\begin{align*}
	\\
	\end{align*}
	\begin{align*}
	(\overline{D}^{0})^{\frac{1}{2}}\Delta Z(\overline{Z}^{0})^{-\frac{1}{2}}+(\overline{D}^{0})^{-\frac{1}{2}}\Delta D(\overline{Z}^{0})^{\frac{1}{2}} & =(\overline{D}^{0}\overline{Z}^{0})^{-\frac{1}{2}}(I-\overline{D}^{0}\cdot\overline{Z}^{0})\\
	& \Longleftrightarrow\\
	Q+P & =R
	\end{align*}
	where 
	\begin{align*}
	P & =(\overline{Z}^{0})^{-\frac{1}{2}}(\overline{D}^{0})^{\frac{1}{2}}\Delta Z\\
	Q & =(\overline{Z}^{0})^{-\frac{1}{2}}(\overline{D}^{0})^{-\frac{1}{2}}\Delta D\overline{Z}^{0}\\
	R & =(\overline{D}^{0}\overline{Z}^{0})^{-\frac{1}{2}}(I-\overline{D}^{0}\cdot\overline{Z}^{0})
	\end{align*}
	and 
	\begin{align*}
	Tr(PQ^{T}) & =Tr(\Delta Z\Delta D)\\
	\end{align*}
	\begin{align*}
	|Tr(PQ^{T})| & \leq\frac{1}{2}|Tr(P^{T}P)+Tr(QQ^{T})+Tr(P^{T}Q)+Tr(Q^{T}P)|\\
	& =\frac{1}{2}Tr(RR^{T})\\
	& \leq\beta
	\end{align*}
	\begin{align*}
	Tr((\overline{D}^{0}\overline{Z}^{0})^{-1}) & \leq\frac{1}{1-\beta}\\
	Tr((I-\overline{D}^{0}\cdot\overline{Z}^{0})^{2}) & \leq\beta^{2}
	\end{align*}
	
	\begin{align*}
	Tr((\overline{D}^{0}\overline{Z}^{0})^{-\frac{1}{2}}(\overline{D}^{0}\overline{Z}^{0})^{-\frac{1}{2}})\\
	\end{align*}
	\begin{align*}
	\|I-\overline{D}^{0}\cdot\overline{Z}^{0}\| & \leq\beta\\
	\|\overline{D}^{0}\cdot\overline{Z}^{0}\| & \geq\sqrt{n}-\beta
	\end{align*}
	\end{proof}
	\end{comment}
	\hfill \halmos
\endproof
%
\begin{proposition} (Proposition \ref{prop:approximate} in the paper)
	Suppose that $(R^{0},S^{0},D^{0},X^{0},Y^{0},Z^{0})$ satisfy 
	
	\begin{align*}
	R^{0} & =M-D^{0}\succeq0\\
	S^{0} & =\kappa^{0}S^{0}-M\succeq0\\
	D^{0} & \succeq0\\
	Z^{0}+\kappa^{0}Y^{0} & =X^{0}
	\end{align*}
	with $\delta(R^{0},X^{0})\leq\delta,\delta(D^{0},Z^{0})\leq\delta,\delta(S^{0},Y^{0})\leq\delta$
	for some $\delta\in(0,1)$. Further, let $\Delta\kappa=\kappa^{0}-\kappa^{1}$
	with 
	\begin{align*}
	\Delta\kappa & =\frac{\beta}{Tr(D^{0}\cdot(\kappa^{0}D^{0}-M)^{-1})}
	\end{align*}
	where $\beta\in(0,1)$ is a sufficiently small constant, then with
	\begin{align*}
	\overline{R}^{0} & =R^{0},\overline{S}^{0}=-\Delta\kappa D^{0}+S^{0},\overline{D}^{0}=D^{0}\\
	\overline{X}^{0} & =X^{0},\overline{Y}^{0}=Y^{0},\overline{Z}^{0}=\Delta\kappa Y^{0}+Z^{0}
	\end{align*}
	we have 
	$\overline{R}^{0} =M-\overline{D}^{0}\succeq0$, $\overline{S}^{0} =\kappa^{1}\overline{D}^{0}-M\succeq 0$, $\overline{D}^{0} \succeq0$, $\overline{Z}^{0}+\kappa^{1}\overline{Y}^{0} =\overline{X}^{0}$,
	and $\delta(\overline{R}^{0},\overline{X}^{0})  \leq\beta$, $\delta(\overline{S}^{0},\overline{Y}^{0})\leq\delta+\beta$, $\delta(\overline{D}^{0},\overline{Z}^{0})\leq\delta+\beta$.
	
\end{proposition}
\proof{Proof}
We have $\delta(\overline{R}^{0},\overline{X}^{0})=\delta(R^{0},X^{0})\leq\delta$
and 
\begin{align*}
\delta(\overline{D}^{0},\overline{Z}^{0})=\|(\overline{D}^{0})^{\frac{1}{2}}\overline{Z}^{0}(\overline{D}^{0})^{\frac{1}{2}}-I\|_{F} & \leq\beta\\
\delta(\overline{S}^{0},\overline{Y}^{0})=\|(\overline{S}^{0})^{\frac{1}{2}}\overline{Y}^{0}(\overline{S}^{0})^{\frac{1}{2}}-I\|_{F} & \leq\beta
\end{align*}
\begin{align*}
\delta(\overline{S}^{0},\overline{Y}^{0})^{2} & =Tr((\overline{S}^{0}\overline{Y}^{0}-I)^{2})\\
& =Tr((S^{0}Y^{0}-\Delta\kappa D^{0}Y^{0}-I)^{2})\\
& =Tr(((S^{0})^{\frac{1}{2}}Y^{0}(S^{0})^{\frac{1}{2}}-\Delta\kappa(S^{0})^{\frac{1}{2}}Y^{0}(S^{0})^{\frac{1}{2}}-I)^{2})\\
& =\|(S^{0})^{\frac{1}{2}}Y^{0}(S^{0})^{\frac{1}{2}}-I-\Delta\kappa(S^{0})^{\frac{1}{2}}Y^{0}(S^{0})^{\frac{1}{2}}\|_{F}^{2}
\end{align*}
so using the triangle inequality of the Frobenius norm, 
\begin{align*}
\delta(\overline{S}^{0},\overline{Y}^{0}) & =\|(S^{0})^{\frac{1}{2}}Y^{0}(S^{0})^{\frac{1}{2}}-I-\Delta\kappa(S^{0})^{\frac{1}{2}}Y^{0}(S^{0})^{\frac{1}{2}}\|_{F}\\
& \leq\|(S^{0})^{\frac{1}{2}}Y^{0}(S^{0})^{\frac{1}{2}}-I\|_{F}+\|\Delta\kappa(S^{0})^{\frac{1}{2}}Y^{0}(S^{0})^{\frac{1}{2}}\|_{F}\\
& \leq\delta+Tr(\Delta\kappa(S^{0})^{\frac{1}{2}}Y^{0}(S^{0})^{\frac{1}{2}})=\delta+\beta
\end{align*}
and similarly $\delta(\overline{D}^{0},\overline{Z}^{0})\leq\delta+\beta$.
\hfill \halmos
\endproof

\begin{theorem}
	(Theorem \ref{thm:approximate center} in the paper) Let $\overline{D}^{0}$
	and $\overline{D}^{1}$ be approximate centers for $\kappa^{0}$ and
	$\kappa^{1}=\kappa^{0}-\frac{\beta}{Tr(\overline{D}^{0}\cdot(\kappa^{0}\overline{D}^{0}-M)^{-1})}$
	respectively, obtained using the Newton update with Nesterov-Todd
	direction for $\beta$ sufficiently small. If 
	\begin{align*}
	\delta(\overline{R}^{0},\overline{X}^{0}) & \leq\delta\\
	\delta(\overline{D}^{0},\overline{Z}^{0}) & \leq\delta\\
	\delta(\overline{S}^{0},\overline{Y}^{0}) & \leq\delta
	\end{align*}
	for $\delta$ a small universal constant, then 
	\begin{align*}
	\delta(\overline{R}^{1},\overline{X}^{1}) & \leq\delta\\
	\delta(\overline{D}^{1},\overline{Z}^{1}) & \leq\delta\\
	\delta(\overline{S}^{1},\overline{Y}^{1}) & \leq\delta
	\end{align*}
	and 
	\begin{align*}
	P(\overline{D}^{1},\kappa^{1}) & \leq P(\overline{D}^{0},\kappa^{0})-c\beta
	\end{align*}
	for $c\in(0,1)$ a universal constant. 
\end{theorem}
\proof{Proof}
	The first part of the proof consists of showing that when the approximate
	center is $O(\eta)$ close to the analytic center, the potential is
	$O(\eta^{2})$ close to the max-potential, for sufficiently small
	$\eta$.
	
	Recall the definition 
	\begin{align*}
	P(D,\kappa) & :=\log\det(M-D)+\log\det(\kappa D-M)+\log\det D
	\end{align*}
	For fixed $\kappa$, suppose we have an approximate center $\overline{D}$
	with 
	\begin{align*}
	\overline{R} & =M-\overline{D}\succeq0\\
	\overline{S} & =\kappa\overline{D}-M\succeq0\\
	\overline{D} & \succeq0\\
	\overline{Z}+\kappa\overline{Y} & =\overline{X}
	\end{align*}
	and
	\begin{align*}
	\delta(\overline{R},\overline{X}) & \leq\eta\\
	\delta(\overline{S},\overline{Y}) & \leq\eta\\
	\delta(\overline{D},\overline{Z}) & \leq\eta
	\end{align*}
	for some small $\eta\in(0,1)$. Let $D$ be the analytic center with
	$\kappa$. The result about Newton update applied to $\overline{D}$
	implies that 
	\begin{align*}
	\|(\overline{D})^{-\frac{1}{2}}D^{(1)}(\overline{D})^{-\frac{1}{2}}-I\|_{F} & \le\frac{\eta}{1-\eta}
	\end{align*}
	where $D'$ is the result of one step of Newton update applied to
	$\overline{D}$. We also know that the new approximate centers have
	distance upper bounded by $\frac{1}{2}\frac{\eta^{2}}{1-\eta}$. Now
	the key is to iterate the Newton update so that we obtain a sequence
	of approximate centers $D^{(1)},D^{(2)},\dots$, that converges to
	$D$. Using the upper bounds on the approximate centers, we obtain,
	with $\overline{D}=D^{(0)}$, 
	\begin{align*}
	\|(\overline{D})^{-\frac{1}{2}}D(\overline{D})^{-\frac{1}{2}}-I\|_{F} & =\|(\overline{D})^{-\frac{1}{2}}D(\overline{D})^{-\frac{1}{2}}-(\overline{D})^{-\frac{1}{2}}(D^{(1)})(\overline{D})^{-\frac{1}{2}}+(\overline{D})^{-\frac{1}{2}}(D^{(1)})(\overline{D})^{-\frac{1}{2}}-I\|_{F}\\
	& =\|(D^{(0)})^{-\frac{1}{2}}D(D^{(0)})^{-\frac{1}{2}}-(D^{(0)})^{-\frac{1}{2}}(D^{(1)})(D^{(0)})^{-\frac{1}{2}}+(D^{(0)})^{-\frac{1}{2}}(D^{(1)})(D^{(0)})^{-\frac{1}{2}}-I\|_{F}\\
	& \leq\|(D^{(0)})^{-\frac{1}{2}}D(D^{(0)})^{-\frac{1}{2}}-(D^{(0)})^{-\frac{1}{2}}(D^{(1)})(D^{(0)})^{-\frac{1}{2}}\|_{F}+\|(D^{(0)})^{-\frac{1}{2}}(D^{(1)})(D^{(0)})^{-\frac{1}{2}}-I\|_{F}\\
	& \leq\sqrt{Tr((D^{(0)})^{-1}(D-(D^{(1)}))^{2}}+\frac{\eta}{1-\eta}\\
	& =\sqrt{Tr((D^{(0)})^{-1}(D^{(1)})(D^{(1)})^{-1}(D-(D^{(1)}))^{2}}+\frac{\eta}{1-\eta}\\
	& \leq\lambda_{1}((D^{(0)})^{-\frac{1}{2}}(D^{(1)})(D^{(0)})^{-\frac{1}{2}})\cdot\sqrt{Tr((D^{(1)})^{-\frac{1}{2}}D(D^{(1)})^{-\frac{1}{2}}-I)^{2}}+\frac{\eta}{1-\eta}\\
	& =\lambda_{1}((D^{(0)})^{-\frac{1}{2}}(D^{(1)})(D^{(0)})^{-\frac{1}{2}})\cdot\|(D^{(1)})^{-\frac{1}{2}}D(D^{(1)})^{-\frac{1}{2}}-I\|_{F}+\frac{\eta}{1-\eta}
	\end{align*}
	where we have used the Cauchy-Schwarz inequality
	\begin{align*}
	\sqrt{Tr(AB)} & \leq\sqrt{Tr(A^{T}A)}\cdot\sqrt{Tr(B^{T}B)}
	\end{align*}
	and the Holder inequality 
	\begin{align*}
	Tr(AB) & \leq\lambda_{1}(A)\cdot Tr(B)
	\end{align*}
	to obtian the last inequality. Now since 
	\begin{align*}
	\|(\overline{D})^{-\frac{1}{2}}D^{(1)}(\overline{D})^{-\frac{1}{2}}-I\|_{F} & \le\frac{\eta}{1-\eta}
	\end{align*}
	we have 
	\begin{align*}
	|\lambda_{1}((D^{(0)})^{-\frac{1}{2}}(D^{(1)})(D^{(0)})^{-\frac{1}{2}})| & \leq\lambda_{1}((D^{(0)})^{-\frac{1}{2}}(D^{(1)})(D^{(0)})^{-\frac{1}{2}}-I)+\lambda_{1}(I)\\
	& \leq\|(D^{(0)})^{-\frac{1}{2}}(D^{(1)})(D^{(0)})^{-\frac{1}{2}}-I\|_{F}+1\\
	& \leq\frac{1}{1-\eta}
	\end{align*}
	The bound on Newton update further implies that 
	\begin{align*}
	\|(D^{(1)})^{-\frac{1}{2}}D^{(2)}(D^{(1)})^{-\frac{1}{2}}-I\|_{F} & \le\frac{\frac{1}{2}\frac{\eta^{2}}{1-\eta}}{1-\frac{1}{2}\frac{\eta^{2}}{1-\eta}}
	\end{align*}
	and iterating the argument above gives 
	\begin{align*}
	\|(\overline{D})^{-\frac{1}{2}}D(\overline{D})^{-\frac{1}{2}}-I\|_{F} & \leq\lambda_{1}((D^{(0)})^{-\frac{1}{2}}(D^{(1)})(D^{(0)})^{-\frac{1}{2}})\cdot\|(D^{(1)})^{-\frac{1}{2}}D(D^{(1)})^{-\frac{1}{2}}-I\|_{F}+\frac{\eta}{1-\eta}\\
	& \leq\frac{1}{1-\eta}\cdot(\lambda_{1}((D^{(1)})^{-\frac{1}{2}}(D^{(2)})(D^{(1)})^{-\frac{1}{2}})\cdot\|(D^{(2)})^{-\frac{1}{2}}D(D^{(2)})^{-\frac{1}{2}}-I\|_{F}+\frac{\frac{1}{2}\frac{\eta^{2}}{1-\eta}}{1-\frac{1}{2}\frac{\eta^{2}}{1-\eta}})+\frac{\eta}{1-\eta}\\
	& \leq\frac{1}{1-\eta}\cdot(\frac{1}{1-\frac{1}{2}\frac{\eta^{2}}{1-\eta}}\cdot\|(D^{(2)})^{-\frac{1}{2}}D(D^{(2)})^{-\frac{1}{2}}-I\|_{F}+\frac{\frac{1}{2}\frac{\eta^{2}}{1-\eta}}{1-\frac{1}{2}\frac{\eta^{2}}{1-\eta}})+\frac{\eta}{1-\eta}
	\end{align*}
	For $\eta<1/2$ , $\frac{1}{2}\frac{\eta^{2}}{1-\eta}\leq\eta^{2}<\eta$,
	so we have the upper bound
	\begin{align*}
	\|(\overline{D})^{-\frac{1}{2}}D(\overline{D})^{-\frac{1}{2}}-I\|_{F} & \leq\frac{1}{1-\eta}\cdot(\frac{1}{1-\frac{1}{2}\frac{\eta^{2}}{1-\eta}}\cdot\|(D^{(2)})^{-\frac{1}{2}}D(D^{(2)})^{-\frac{1}{2}}-I\|_{F}+\frac{\frac{1}{2}\frac{\eta^{2}}{1-\eta}}{1-\frac{1}{2}\frac{\eta^{2}}{1-\eta}})+\frac{\eta}{1-\eta}\\
	& \leq\frac{1}{1-\eta}\cdot\frac{1}{1-\frac{1}{2}\frac{\eta^{2}}{1-\eta}}\cdot\|(D^{(2)})^{-\frac{1}{2}}D(D^{(2)})^{-\frac{1}{2}}-I\|_{F}+\frac{\eta^{2}}{(1-\eta)^{2}}+\frac{\eta}{1-\eta}\\
	& \leq\frac{1}{1-\eta}\cdot\frac{1}{1-\eta^{2}}\cdot\|(D^{(2)})^{-\frac{1}{2}}D(D^{(2)})^{-\frac{1}{2}}-I\|_{F}+\frac{\eta^{2}}{(1-\eta)^{2}}+\frac{\eta}{1-\eta}\\
	& \leq\sum_{k=1}^{n}(\frac{\eta}{1-\eta})^{k}=\frac{\eta}{1-\eta}\frac{1-\eta}{1-2\eta}=\frac{\eta}{1-2\eta}
	\end{align*}
	Now by concavity of $P(D,\kappa)$ in $D$, we have 
	\begin{align*}
	P(D,\kappa) & :=\log\det(M-D)+\log\det(\kappa D-M)+\log\det D
	\end{align*}
	\begin{align*}
	P(D,\kappa)-P(\overline{D},\kappa) & \leq Tr(\nabla_{D}P(\overline{D},\kappa)\cdot(D-\overline{D})\\
	& =Tr((-\overline{R}^{-1}+\kappa\overline{S}^{-1}+\overline{D}^{-1})\cdot(D-\overline{D}))\\
	& =Tr((-\overline{R}^{-1}+\overline{X}+\kappa\overline{S}^{-1}-\kappa\overline{Y}+\overline{D}^{-1}-\overline{Z})\cdot(D-\overline{D}))\\
	& =Tr((-\overline{R}^{-1}+\overline{X})(\overline{R}-R))+Tr((\overline{S}^{-1}-\overline{Y})(S-\overline{S}))+Tr((\overline{D}^{-1}-\overline{Z})\cdot(D-\overline{D}))
	\end{align*}
	The three quantities are all $O(\eta^{2})$: For example,
	\begin{align*}
	Tr((\overline{D}^{-1}-\overline{Z})\cdot(D-\overline{D})) & =Tr((\overline{D})^{\frac{1}{2}}(\overline{D}^{-1}-\overline{Z})(\overline{D})^{\frac{1}{2}}\cdot(\overline{D})^{-\frac{1}{2}}(D-\overline{D})(\overline{D})^{-\frac{1}{2}})\\
	& \leq\|(I-(\overline{D})^{\frac{1}{2}}\overline{Z}(\overline{D})^{\frac{1}{2}})\|_{F}\cdot\|(I-(\overline{D})^{-\frac{1}{2}}D(\overline{D})^{-\frac{1}{2}}\|_{F}\\
	& \leq\eta\cdot\frac{\eta}{1-2\eta}
	\end{align*}
	and similarly we have $O(\eta^{2})$ bounds for the other two quantities,
	because of similar $O(\eta)$ bounds for $\|(\overline{R})^{-\frac{1}{2}}R(\overline{R})^{-\frac{1}{2}}-I\|_{F}$
	and $\|(\overline{S})^{-\frac{1}{2}}S(\overline{S})^{-\frac{1}{2}}-I\|_{F}$. 
	
	Now let $\overline{D}^{0}$ be an approximate center for $\kappa^{0}$,
	and $\overline{D}^{1}$ be an approximate center for $\kappa^{1}$,
	obtained using Newton updates. Recall that $\kappa^{1}=\kappa^{0}-\frac{\beta}{Tr((\overline{D})^{0}\cdot(\kappa^{0}(\overline{D})^{0}-M)^{-1})}.$
	We have, with $\eta=\delta+\beta$,
	\begin{align*}
	P(\kappa^{1},\overline{D}^{1})-P(\kappa^{0},\overline{D}^{0}) & =P(\kappa^{1},\overline{D}^{1})-P(\kappa^{1},D^{1})+P(\kappa^{1},D^{1})-P(\kappa^{0},D^{0})+P(\kappa^{0},D^{0})-P(\kappa^{0},\overline{D}^{0})\\
	& \leq-\beta+P(\kappa^{0},D^{0})-P(\kappa^{0},\overline{D}^{0})\\
	& \leq-\beta+c\cdot\eta^{2}
	\end{align*}
	With $\delta$ and $\beta$ small enough, $-\beta+c\cdot\eta^{2}\leq-c'\beta$
	for some $c'\in(0,1)$, and 
	\begin{align*}
	\delta(\overline{R}^{1},\overline{X}^{1})\leq\frac{1}{2}\frac{(\delta+\beta)^{2}}{1-(\delta+\beta)} & \leq\delta
	\end{align*}
	\hfill \halmos
\endproof
